# Supplementary material for: Do Schwartz Higher-Order Values Help Sentence-Level Human Value Detection? A Study of Hierarchical Gating and Calibration
Source: arXiv:2602.00913 ancillary file (2026-04-07)
Supplement: Supplementary file 1 [file paper-supplement.pdf]

Supplementary Material for  
*Do Schwartz Higher-Order Values Help Sentence-Level  
Human Value Detection? When Hard Gating Hurts*

Víctor Yeste<sup>a,b,\*</sup>, Paolo Rosso<sup>a,c</sup>

<sup>a</sup>*PRHLT Research Center, Universitat Politècnica de València, Valencia, 46022, Spain*

<sup>b</sup>*School of Science, Engineering and Design, Universidad Europea de  
Valencia, Valencia, 46010, Spain*

<sup>c</sup>*Valencian Graduate School and Research Network of Artificial Intelligence (ValgrAI),*

---

**Abstract**

This document contains supplementary material for the article “*Do Schwartz Higher-Order Values Help Sentence-Level Human Value Detection? When Hard Gating Hurts*”. It reports additional corpus statistics, per-value and per-configuration results, ablation tables, and implementation details that complement the main text.

---

**S1. Abbreviation key for moral value labels**

To improve readability in tables (especially per-label significance reports), we use the following abbreviations for the moral value labels:

---

\*Corresponding author

*Email address:* `vicyesmo@upv.es` (Víctor Yeste)

Table S1: Abbreviation mapping for moral value labels used across appendices.

| Abbrev. | Full label                 |
|---------|----------------------------|
| SD-t    | Self-direction: thought    |
| SD-a    | Self-direction: action     |
| Stim    | Stimulation                |
| Hed     | Hedonism                   |
| Ach     | Achievement                |
| Pow-d   | Power: dominance           |
| Pow-r   | Power: resources           |
| Face    | Face                       |
| Sec-per | Security: personal         |
| Sec-soc | Security: societal         |
| Trad    | Tradition                  |
| Conf-r  | Conformity: rules          |
| Conf-i  | Conformity: interpersonal  |
| Hum     | Humility                   |
| Ben-c   | Benevolence: caring        |
| Ben-d   | Benevolence: dependability |
| Uni-c   | Universalism: concern      |
| Uni-n   | Universalism: nature       |
| Uni-t   | Universalism: tolerance    |

## S2. Higher-order category detection results

This appendix reports higher-order (binary) category detection results on the validation and test sets. Validation results (F1 per class and macro-average) are provided for all evaluated model variants. Test results are reported only for the baseline and the best-performing models selected from validation, using either a fixed 0.50 decision threshold for both classes or tuned class-specific thresholds selected on the validation set; additional feature/strategy combinations were explored primarily to assess whether combining signals improved validation performance beyond single-strategy variants.

*S2.1. Growth vs. Self-Protection*

*S2.2. Social Focus vs. Personal Focus*

*S2.3. Openness to Change vs. Conservation*

*S2.4. Self-Transcendence vs. Self-Enhancement*

Table S2: Validation F1-scores for Growth vs. Self-Protection detection (macro-average over the two classes).

| Model                     | Growth | Self-Protection | Macro- $F_1$ |
|---------------------------|--------|-----------------|--------------|
| Baseline                  | 0.55   | 0.61            | 0.58         |
| Token Pruning             | 0.55   | 0.60            | 0.57         |
| 2 prev sent w/ label      | 0.54   | 0.60            | 0.57         |
| MultiLayer                | 0.54   | 0.60            | 0.57         |
| Residual Block            | 0.55   | 0.59            | 0.57         |
| Data Augmentation         | 0.39   | 0.48            | 0.44         |
| Custom Stopwords          | 0.54   | 0.60            | 0.57         |
| NER                       | 0.54   | 0.60            | 0.57         |
| Lex - Schwartz            | 0.54   | 0.59            | 0.56         |
| Lex - VAD                 | 0.54   | 0.60            | 0.57         |
| Lex - EmoLex              | 0.55   | 0.59            | 0.57         |
| Lex - Emotion Intensity   | 0.55   | 0.61            | 0.58         |
| Lex - WorryWords          | 0.54   | 0.59            | 0.56         |
| Lex - LIWC 15             | 0.54   | 0.60            | 0.57         |
| Lex - MFD                 | 0.55   | 0.58            | 0.56         |
| Lex - LIWC 22             | 0.54   | 0.58            | 0.56         |
| Lex - LIWC 22 + Ling Feat | 0.55   | 0.60            | 0.57         |
| Lex - MFD-20              | 0.54   | 0.60            | 0.57         |
| Lex - eMFD                | 0.55   | 0.58            | 0.56         |
| Lex - MJD                 | 0.55   | 0.59            | 0.57         |
| TD - LDA                  | 0.54   | 0.58            | 0.56         |
| TD - NMF                  | 0.55   | 0.59            | 0.57         |
| TD - BERTopic             | 0.55   | 0.59            | 0.57         |

Table S3: Test F1-scores for Growth vs. Self-Protection detection using fixed (0.5) vs. tuned thresholds. Thr and F1 are reported as Growth/Self-Protection pairs; Macro- $F_1$  is the macro-average over the two classes.

| Model    | Thr (G/SP) | F1 (G/SP) | Macro- $F_1$ |
|----------|------------|-----------|--------------|
| Baseline | 0.50/0.50  | 0.56/0.61 | <b>0.58</b>  |
|          | 0.18/0.10  | 0.54/0.62 | <b>0.58</b>  |

Table S4: Validation F1-scores for Social Focus vs. Personal Focus detection (macro-average over the two classes).

| <b>Model</b>                                        | <b>Social</b> | <b>Personal</b> | <b>Macro-<math>F_1</math></b> |
|-----------------------------------------------------|---------------|-----------------|-------------------------------|
| Baseline                                            | 0.59          | 0.50            | 0.54                          |
| Token Pruning                                       | 0.57          | 0.49            | 0.53                          |
| 2 prev sent w/ label                                | 0.59          | 0.50            | 0.54                          |
| MultiLayer                                          | 0.59          | 0.51            | 0.55                          |
| Residual Block                                      | 0.58          | 0.51            | 0.54                          |
| Data Augmentation                                   | 0.48          | 0.36            | 0.42                          |
| Custom Stopwords                                    | 0.57          | 0.49            | 0.53                          |
| NER                                                 | 0.58          | 0.50            | 0.54                          |
| Lex - Schwartz                                      | 0.59          | 0.50            | 0.54                          |
| Lex - VAD                                           | 0.59          | 0.49            | 0.54                          |
| Lex - EmoLex                                        | 0.59          | 0.50            | 0.54                          |
| Lex - Emotion Intensity                             | 0.58          | 0.51            | 0.54                          |
| Lex - WorryWords                                    | 0.58          | 0.51            | 0.54                          |
| Lex - LIWC 15                                       | 0.58          | 0.50            | 0.54                          |
| Lex - MFD                                           | 0.59          | 0.50            | 0.54                          |
| Lex - LIWC 22                                       | 0.06          | 0.01            | 0.03                          |
| Lex - LIWC 22 + Ling Feat                           | 0.59          | 0.50            | 0.54                          |
| Lex - MFD-20                                        | 0.58          | 0.50            | 0.54                          |
| Lex - eMFD                                          | 0.60          | 0.48            | 0.54                          |
| Lex - MJD                                           | 0.59          | 0.50            | 0.54                          |
| TD - LDA                                            | 0.58          | 0.51            | 0.54                          |
| TD - NMF                                            | 0.59          | 0.51            | 0.55                          |
| TD - BERTopic                                       | 0.58          | 0.51            | 0.54                          |
| 2 prev sent w/ label + NER                          | 0.60          | 0.50            | 0.55                          |
| 2 prev sent w/ label + Lex - Schwartz               | 0.58          | 0.50            | 0.54                          |
| 2 prev sent w/ label + Lex - Worry-<br>Words        | 0.59          | 0.51            | 0.55                          |
| 2 prev sent w/ label + Lex - LIWC 15                | 0.60          | 0.50            | 0.55                          |
| 2 prev sent w/ label + Lex - LIWC 22                | 0.58          | 0.50            | 0.54                          |
| 2 prev sent w/ label + Lex - LIWC 22<br>+ Ling Feat | 0.58          | 0.50            | 0.54                          |
| 2 prev sent w/ label + TD - NMF                     | 0.60          | 0.50            | 0.55                          |
| 2 prev sent w/ label + TD - BERTopic                | 0.59          | 0.51            | 0.55                          |
| NER + Lex - Schwartz                                | 0.59          | 0.50            | 0.54                          |
| NER + Lex - WorryWords                              | 0.59          | 0.51            | 0.55                          |
| NER + Lex - LIWC 15                                 | 0.59          | 0.51            | 0.55                          |
| NER + Lex - LIWC 22                                 | 0.59          | 0.50            | 0.54                          |
| NER + Lex - LIWC 22 + Ling Feat                     | 0.59          | 0.50            | 0.54                          |
| NER + TD - NMF                                      | 0.59          | 0.50            | 0.54                          |
| NER + TD - BERTopic                                 | 0.58          | 0.51            | 0.54                          |

Table S5: Test F1-scores for Social Focus vs. Personal Focus detection using fixed (0.5) vs. tuned thresholds. Thr and F1 are reported as Social/Personal pairs; Macro- $F_1$  is the macro-average over the two classes.

| Model                | Thr (S/P) | F1 (S/P)  | Macro- $F_1$ |
|----------------------|-----------|-----------|--------------|
| Baseline             | 0.50/0.50 | 0.46/0.37 | 0.41         |
|                      | 0.11/0.52 | 0.48/0.37 | 0.43         |
| 2 prev sent w/ label | 0.50/0.50 | 0.58/0.51 | 0.54         |
|                      | 0.10/0.15 | 0.59/0.53 | 0.56         |
| NER                  | 0.50/0.50 | 0.59/0.52 | 0.55         |
|                      | 0.10/0.19 | 0.59/0.54 | <b>0.57</b>  |
| Lex - Schwartz       | 0.50/0.50 | 0.59/0.52 | 0.55         |
|                      | 0.10/0.21 | 0.58/0.54 | 0.56         |
| Lex - WorryWords     | 0.50/0.50 | 0.58/0.52 | 0.55         |
|                      | 0.10/0.21 | 0.59/0.54 | <b>0.57</b>  |
| Lex - LIWC 15        | 0.50/0.50 | 0.59/0.50 | 0.55         |
|                      | 0.10/0.17 | 0.59/0.54 | <b>0.57</b>  |
| TD - NMF             | 0.50/0.50 | 0.59/0.52 | 0.56         |
|                      | 0.10/0.20 | 0.58/0.54 | 0.56         |
| TD - BERTopic        | 0.50/0.50 | 0.59/0.51 | 0.55         |
|                      | 0.10/0.22 | 0.58/0.54 | 0.56         |
| Lex - LIWC 22        | 0.50/0.50 | 0.06/0.01 | 0.04         |
|                      | 0.29/0.35 | 0.49/0.28 | 0.38         |

Table S6: Validation F1-scores for Openness to Change vs. Conservation detection (macro-average over the two classes).

| Model                     | Openness | Conservation | Macro- $F_1$ |
|---------------------------|----------|--------------|--------------|
| Baseline                  | 0.34     | 0.49         | 0.42         |
| Token Pruning             | 0.34     | 0.49         | 0.42         |
| 2 prev sent w/ label      | 0.27     | 0.49         | 0.38         |
| MultiLayer                | 0.34     | 0.49         | 0.42         |
| Residual Block            | 0.33     | 0.49         | 0.41         |
| Data Augmentation         | 0.19     | 0.40         | 0.30         |
| Custom Stopwords          | 0.33     | 0.49         | 0.41         |
| NER                       | 0.33     | 0.49         | 0.41         |
| Lex - Schwartz            | 0.34     | 0.47         | 0.40         |
| Lex - VAD                 | 0.33     | 0.50         | 0.42         |
| Lex - EmoLex              | 0.34     | 0.48         | 0.41         |
| Lex - Emotion Intensity   | 0.33     | 0.50         | 0.42         |
| Lex - WorryWords          | 0.33     | 0.49         | 0.41         |
| Lex - LIWC 15             | 0.34     | 0.48         | 0.41         |
| Lex - MFD                 | 0.34     | 0.47         | 0.40         |
| Lex - LIWC 22             | 0.33     | 0.48         | 0.40         |
| Lex - LIWC 22 + Ling Feat | 0.34     | 0.51         | 0.43         |
| Lex - MFD-20              | 0.33     | 0.48         | 0.40         |
| Lex - eMFD                | 0.33     | 0.47         | 0.40         |
| Lex - MJD                 | 0.34     | 0.49         | 0.42         |
| TD - LDA                  | 0.33     | 0.50         | 0.42         |
| TD - NMF                  | 0.34     | 0.49         | 0.42         |
| TD - BERTopic             | 0.34     | 0.49         | 0.42         |

Table S7: Test F1-scores for Openness to Change vs. Conservation detection using fixed (0.5) vs. tuned thresholds. Thr and F1 are reported as Openness/Conservation pairs; Macro- $F_1$  is the macro-average over the two classes.

| Model                     | Thr (O/C) | F1 (O/C)  | Macro- $F_1$ |
|---------------------------|-----------|-----------|--------------|
| Baseline                  | 0.50/0.50 | 0.33/0.50 | <b>0.417</b> |
|                           | 0.85/0.12 | 0.25/0.50 | 0.38         |
| Lex - LIWC 22 + Ling Feat | 0.50/0.50 | 0.34/0.50 | <b>0.421</b> |
|                           | 0.82/0.10 | 0.27/0.51 | 0.39         |

Table S8: Validation F1-scores for Self-Transcendence vs. Self-Enhancement detection (macro-average over the two classes).

| <b>Model</b>              | <b>Self-Trans.</b> | <b>Self-Enh.</b> | <b>Macro-<math>F_1</math></b> |
|---------------------------|--------------------|------------------|-------------------------------|
| Baseline                  | 0.47               | 0.43             | 0.45                          |
| Token Pruning             | 0.45               | 0.43             | 0.44                          |
| 2 prev sent w/ label      | 0.47               | 0.43             | 0.45                          |
| MultiLayer                | 0.46               | 0.42             | 0.44                          |
| Residual Block            | 0.46               | 0.43             | 0.44                          |
| Data Augmentation         | 0.28               | 0.31             | 0.30                          |
| Custom Stopwords          | 0.47               | 0.43             | 0.45                          |
| NER                       | 0.46               | 0.44             | 0.45                          |
| Lex - Schwartz            | 0.45               | 0.45             | 0.45                          |
| Lex - VAD                 | 0.46               | 0.44             | 0.45                          |
| Lex - EmoLex              | 0.45               | 0.42             | 0.44                          |
| Lex - Emotion Intensity   | 0.47               | 0.43             | 0.45                          |
| Lex - WorryWords          | 0.46               | 0.44             | 0.45                          |
| Lex - LIWC 15             | 0.47               | 0.44             | 0.45                          |
| Lex - MFD                 | 0.45               | 0.43             | 0.44                          |
| Lex - LIWC 22             | 0.43               | 0.44             | 0.44                          |
| Lex - LIWC 22 + Ling Feat | 0.46               | 0.43             | 0.44                          |
| Lex - MFD-20              | 0.46               | 0.44             | 0.45                          |
| Lex - eMFD                | 0.46               | 0.44             | 0.45                          |
| Lex - MJD                 | 0.46               | 0.44             | 0.45                          |
| TD - LDA                  | 0.46               | 0.44             | 0.45                          |
| TD - NMF                  | 0.46               | 0.42             | 0.44                          |
| TD - BERTopic             | 0.48               | 0.44             | 0.46                          |



Table S9: Test F1-scores for Self-Transcendence vs. Self-Enhancement detection using fixed (0.5) vs. tuned thresholds. Thr and F1 are reported as Self-Transcendence/Self-Enhancement pairs; Macro- $F_1$  is the macro-average over the two classes.

| Model            | Thr (ST/SE) | F1 (ST/SE) | Macro- $F_1$ |
|------------------|-------------|------------|--------------|
| Baseline         | 0.50/0.50   | 0.52/0.43  | 0.48         |
|                  | 0.27/0.24   | 0.52/0.43  | 0.50         |
| Lex - WorryWords | 0.50/0.50   | 0.51/0.43  | 0.47         |
|                  | 0.16/0.23   | 0.53/0.48  | <b>0.51</b>  |
| Lex - MFD-20     | 0.50/0.50   | 0.52/0.44  | 0.48         |
|                  | 0.21/0.24   | 0.53/0.48  | <b>0.51</b>  |
| TD - BERTopic    | 0.50/0.50   | 0.51/0.44  | 0.48         |
|                  | 0.19/0.29   | 0.53/0.48  | 0.50         |

### S3. Higher-order category detection with a Presence gate

This appendix reports higher-order (binary) category detection results when a Presence detector is used as a gate: for each sentence, the Presence model first decides whether a value is present (using a gate probability threshold), and higher-order predictions are then applied only to sentences passing the gate; multiple Presence models (selected from the best Presence detectors) and gate thresholds are compared on the test set to assess sensitivity to the gating configuration.

*S3.1. Growth vs. Self-Protection*

*S3.2. Social Focus vs. Personal Focus*

*S3.3. Openness to Change vs. Conservation*

*S3.4. Self-Transcendence vs. Self-Enhancement*

Table S10: Validation F1-scores for Growth vs. Self-Protection detection with a Presence gate (macro-average over the two classes).

| <b>Model</b>                     | <b>Growth</b> | <b>Self-Protection</b> | <b>Macro-<math>F_1</math></b> |
|----------------------------------|---------------|------------------------|-------------------------------|
| Baseline                         | 0.72          | 0.82                   | 0.77                          |
| Token Pruning                    | 0.72          | 0.82                   | 0.77                          |
| 2 prev sent w/ label             | 0.72          | 0.83                   | 0.77                          |
| MultiLayer                       | 0.72          | 0.82                   | 0.77                          |
| Residual Block                   | 0.71          | 0.83                   | 0.77                          |
| Data Augmentation                | 0.66          | 0.81                   | 0.74                          |
| Custom Stopwords                 | 0.71          | 0.83                   | 0.77                          |
| NER                              | 0.71          | 0.83                   | 0.77                          |
| Lex - Schwartz                   | 0.71          | 0.83                   | 0.77                          |
| Lex - VAD                        | 0.72          | 0.84                   | 0.78                          |
| Lex - EmoLex                     | 0.72          | 0.82                   | 0.77                          |
| Lex - Emotion Intensity          | 0.73          | 0.82                   | 0.77                          |
| Lex - WorryWords                 | 0.72          | 0.82                   | 0.77                          |
| Lex - LIWC 15                    | 0.72          | 0.82                   | 0.77                          |
| Lex - MFD                        | 0.72          | 0.83                   | 0.77                          |
| Lex - LIWC 22                    | 0.72          | 0.82                   | 0.77                          |
| Lex - LIWC 22 + Ling Feat        | 0.72          | 0.82                   | 0.77                          |
| Lex - MFD-20                     | 0.72          | 0.82                   | 0.77                          |
| Lex - eMFD                       | 0.71          | 0.83                   | 0.77                          |
| Lex - MJD                        | 0.48          | 0.82                   | 0.65                          |
| TD - LDA                         | 0.72          | 0.82                   | 0.77                          |
| TD - NMF                         | 0.72          | 0.82                   | 0.77                          |
| TD - BERTopic                    | 0.71          | 0.73                   | 0.77                          |
| 2 prev sent w/ label + Lex - VAD | 0.72          | 0.82                   | 0.77                          |

Table S11: Test F1-scores for Growth vs. Self-Protection detection with a Presence gate. The configuration column indicates the higher-order model (HO) and the Presence gate model with its gate threshold. Fixed results use a 0.50/0.50 higher-order threshold; tuned results use class-specific higher-order thresholds selected on validation.

| Configuration              | Thr (G/SP) | F1 (G/SP) | Macro- $F_1$ |
|----------------------------|------------|-----------|--------------|
| Baseline                   | 0.50/0.50  | 0.53/0.62 | 0.57         |
| Gate: Baseline@0.50        | 0.10/0.10  | 0.53/0.62 | 0.57         |
| Baseline                   | 0.50/0.50  | 0.53/0.62 | 0.57         |
| Gate: LIWC22+LingFeat@0.50 | 0.10/0.10  | 0.53/0.62 | <b>0.58</b>  |
| Baseline                   | 0.50/0.50  | 0.53/0.60 | 0.57         |
| Gate: LIWC22+LingFeat@0.10 | 0.24/0.10  | 0.53/0.60 | 0.56         |
| Baseline                   | 0.50/0.50  | 0.53/0.61 | 0.57         |
| Gate: 2 prev + EmoLex@0.10 | 0.10/0.10  | 0.53/0.61 | 0.57         |
| Baseline                   | 0.50/0.50  | 0.53/0.61 | 0.57         |
| Gate: 2 prev + LIWC22@0.10 | 0.14/0.10  | 0.53/0.61 | 0.57         |
| Baseline                   | 0.50/0.50  | 0.53/0.61 | 0.57         |
| Gate: 2 prev + eMFD@0.10   | 0.10/0.10  | 0.53/0.61 | 0.57         |
| Lex - VAD                  | 0.50/0.50  | 0.53/0.62 | <b>0.58</b>  |
| Gate: Baseline@0.50        | 0.10/0.10  | 0.53/0.62 | <b>0.58</b>  |
| Lex - VAD                  | 0.50/0.50  | 0.53/0.62 | <b>0.58</b>  |
| Gate: LIWC22+LingFeat@0.50 | 0.10/0.10  | 0.54/0.62 | <b>0.58</b>  |
| Lex - VAD                  | 0.50/0.50  | 0.53/0.61 | 0.57         |
| Gate: LIWC22+LingFeat@0.10 | 0.16/0.10  | 0.53/0.60 | 0.57         |
| Lex - VAD                  | 0.50/0.50  | 0.53/0.61 | 0.57         |
| Gate: 2 prev + EmoLex@0.10 | 0.10/0.10  | 0.53/0.61 | 0.57         |
| Lex - VAD                  | 0.50/0.50  | 0.53/0.62 | 0.57         |
| Gate: 2 prev + LIWC22@0.10 | 0.10/0.10  | 0.53/0.61 | 0.57         |
| Lex - VAD                  | 0.50/0.50  | 0.53/0.61 | 0.57         |
| Gate: 2 prev + eMFD@0.10   | 0.10/0.10  | 0.53/0.61 | 0.57         |

Table S12: Validation F1-scores for Social Focus vs. Personal Focus detection with a Presence gate (macro-average over the two classes).

| Model                                               | Social | Personal | Macro- $F_1$ |
|-----------------------------------------------------|--------|----------|--------------|
| Baseline                                            | 0.76   | 0.71     | 0.74         |
| Token Pruning                                       | 0.77   | 0.69     | 0.73         |
| 2 prev sent w/ label                                | 0.77   | 0.68     | 0.73         |
| MultiLayer                                          | 0.75   | 0.71     | 0.73         |
| Residual Block                                      | 0.76   | 0.71     | 0.74         |
| Data Augmentation                                   | 0.71   | 0.64     | 0.68         |
| Custom Stopwords                                    | 0.76   | 0.71     | 0.74         |
| NER                                                 | 0.75   | 0.72     | 0.74         |
| Lex - Schwartz                                      | 0.76   | 0.69     | 0.72         |
| Lex - VAD                                           | 0.75   | 0.71     | 0.73         |
| Lex - EmoLex                                        | 0.76   | 0.69     | 0.72         |
| Lex - Emotion Intensity                             | 0.76   | 0.70     | 0.73         |
| Lex - WorryWords                                    | 0.76   | 0.71     | 0.74         |
| Lex - LIWC 15                                       | 0.76   | 0.69     | 0.73         |
| Lex - MFD                                           | 0.76   | 0.71     | 0.74         |
| Lex - LIWC 22                                       | 0.76   | 0.71     | 0.74         |
| Lex - LIWC 22 + Ling Feat                           | 0.76   | 0.71     | 0.74         |
| Lex - MFD-20                                        | 0.76   | 0.71     | 0.74         |
| Lex - eMFD                                          | 0.76   | 0.70     | 0.73         |
| Lex - MJD                                           | 0.75   | 0.69     | 0.72         |
| TD - LDA                                            | 0.77   | 0.69     | 0.73         |
| TD - NMF                                            | 0.77   | 0.70     | 0.74         |
| TD - BERTopic                                       | 0.77   | 0.67     | 0.72         |
| 2 prev sent w/ label + Residual Block               | 0.75   | 0.72     | 0.74         |
| 2 prev sent w/ label + Custom Stopwords             | 0.76   | 0.68     | 0.72         |
| 2 prev sent w/ label + NER                          | 0.75   | 0.71     | 0.73         |
| Residual Block + Custom Stopwords                   | 0.76   | 0.71     | 0.74         |
| Residual Block + NER                                | 0.76   | 0.71     | 0.74         |
| NER + Custom Stopwords                              | 0.76   | 0.70     | 0.73         |
| 2 prev sent w/ label + Lex - Schwartz               | 0.75   | 0.72     | 0.74         |
| 2 prev sent w/ label + Lex - EmoLex                 | 0.76   | 0.69     | 0.72         |
| 2 prev sent w/ label + Lex - Emotion Inten-<br>sity | 0.76   | 0.69     | 0.72         |
| 2 prev sent w/ label + Lex - WorryWords             | 0.76   | 0.71     | 0.74         |
| 2 prev sent w/ label + Lex - LIWC 15                | 0.86   | 0.68     | 0.72         |
| 2 prev sent w/ label + Lex - MFD                    | 0.76   | 0.70     | 0.73         |
| 2 prev sent w/ label + Lex - LIWC 22                | 0.76   | 0.72     | 0.74         |
| 2 prev sent w/ label + Lex - MFD-20                 | 0.75   | 0.72     | 0.74         |
| 2 prev sent w/ label + TD - LDA                     | 0.76   | 0.68     | 0.72         |
| 2 prev sent w/ label + TD - NMF                     | 0.76   | 0.70     | 0.73         |
| 2 prev sent w/ label + TD - BERTopic                | 0.77   | 0.68     | 0.73         |

Table S13: Test F1-scores for Social Focus vs. Personal Focus detection with a Presence gate (Part 1/5). Best Macro- $F_1$  values are bolded.

| Configuration              | Thr (S/P) | F1 (S/P)  | Macro- $F_1$ |
|----------------------------|-----------|-----------|--------------|
| Baseline                   | 0.50/0.50 | 0.59/0.52 | 0.55         |
| Gate: Baseline@0.50        | 0.10/0.10 | 0.59/0.52 | <b>0.56</b>  |
| Baseline                   | 0.50/0.50 | 0.59/0.52 | <b>0.56</b>  |
| Gate: LIWC22+LingFeat@0.50 | 0.10/0.10 | 0.59/0.53 | <b>0.56</b>  |
| Baseline                   | 0.50/0.50 | 0.58/0.52 | 0.55         |
| Gate: LIWC22+LingFeat@0.10 | 0.10/0.59 | 0.58/0.52 | 0.55         |
| Baseline                   | 0.50/0.50 | 0.59/0.52 | 0.55         |
| Gate: 2 prev + EmoLex@0.10 | 0.10/0.10 | 0.59/0.52 | 0.55         |
| Baseline                   | 0.50/0.50 | 0.59/0.52 | <b>0.56</b>  |
| Gate: 2 prev + LIWC22@0.10 | 0.10/0.17 | 0.59/0.53 | <b>0.56</b>  |
| Baseline                   | 0.50/0.50 | 0.59/0.51 | 0.55         |
| Gate: 2 prev + eMFD@0.10   | 0.10/0.10 | 0.59/0.52 | 0.55         |
| 2 prev sent w/ label       | 0.50/0.50 | 0.58/0.48 | 0.53         |
| Gate: Baseline@0.50        | 0.10/0.10 | 0.57/0.52 | 0.54         |
| 2 prev sent w/ label       | 0.50/0.50 | 0.59/0.48 | 0.53         |
| Gate: LIWC22+LingFeat@0.50 | 0.10/0.10 | 0.57/0.52 | 0.55         |
| 2 prev sent w/ label       | 0.50/0.50 | 0.57/0.50 | 0.53         |
| Gate: LIWC22+LingFeat@0.10 | 0.11/0.30 | 0.55/0.51 | 0.53         |
| 2 prev sent w/ label       | 0.50/0.50 | 0.58/0.49 | 0.53         |
| Gate: 2 prev + EmoLex@0.10 | 0.10/0.16 | 0.55/0.52 | 0.54         |
| 2 prev sent w/ label       | 0.50/0.50 | 0.58/0.49 | 0.53         |
| Gate: 2 prev + LIWC22@0.10 | 0.10/0.21 | 0.56/0.51 | 0.53         |
| 2 prev sent w/ label       | 0.50/0.50 | 0.58/0.49 | 0.53         |
| Gate: 2 prev + eMFD@0.10   | 0.10/0.15 | 0.56/0.52 | 0.54         |
| NER                        | 0.50/0.50 | 0.59/0.52 | <b>0.56</b>  |
| Gate: Baseline@0.50        | 0.10/0.10 | 0.59/0.53 | <b>0.56</b>  |
| NER                        | 0.50/0.50 | 0.59/0.53 | <b>0.56</b>  |
| Gate: LIWC22+LingFeat@0.50 | 0.10/0.10 | 0.60/0.53 | <b>0.56</b>  |
| NER                        | 0.50/0.50 | 0.58/0.52 | 0.55         |
| Gate: LIWC22+LingFeat@0.10 | 0.10/0.50 | 0.58/0.52 | 0.55         |
| NER                        | 0.50/0.50 | 0.59/0.53 | <b>0.56</b>  |
| Gate: 2 prev + EmoLex@0.10 | 0.10/0.21 | 0.59/0.53 | <b>0.56</b>  |
| NER                        | 0.50/0.50 | 0.59/0.53 | <b>0.56</b>  |
| Gate: 2 prev + LIWC22@0.10 | 0.10/0.39 | 0.59/0.53 | <b>0.56</b>  |
| NER                        | 0.50/0.50 | 0.59/0.52 | <b>0.56</b>  |
| Gate: 2 prev + eMFD@0.10   | 0.10/0.13 | 0.59/0.53 | <b>0.56</b>  |

Table S14: Test F1-scores for Social Focus vs. Personal Focus detection with a Presence gate (Part 2/5). Best Macro- $F_1$  values are bolded.

| Configuration              | Thr (S/P) | F1 (S/P)  | Macro- $F_1$ |
|----------------------------|-----------|-----------|--------------|
| Lex - Schwartz             | 0.50/0.50 | 0.59/0.49 | 0.54         |
| Gate: Baseline@0.50        | 0.10/0.11 | 0.58/0.52 | 0.55         |
| Lex - Schwartz             | 0.50/0.50 | 0.59/0.50 | 0.55         |
| Gate: LIWC22+LingFeat@0.50 | 0.10/0.10 | 0.58/0.52 | 0.55         |
| Lex - Schwartz             | 0.50/0.50 | 0.59/0.50 | 0.54         |
| Gate: LIWC22+LingFeat@0.10 | 0.10/0.42 | 0.56/0.51 | 0.53         |
| Lex - Schwartz             | 0.50/0.50 | 0.59/0.50 | 0.55         |
| Gate: 2 prev + EmoLex@0.10 | 0.10/0.22 | 0.57/0.52 | 0.54         |
| Lex - Schwartz             | 0.50/0.50 | 0.59/0.50 | 0.55         |
| Gate: 2 prev + LIWC22@0.10 | 0.10/0.28 | 0.57/0.52 | 0.54         |
| Lex - Schwartz             | 0.50/0.50 | 0.59/0.50 | 0.55         |
| Gate: 2 prev + eMFD@0.10   | 0.10/0.19 | 0.57/0.52 | 0.54         |
| Lex - EmoLex               | 0.50/0.50 | 0.59/0.49 | 0.54         |
| Gate: Baseline@0.50        | 0.10/0.11 | 0.58/0.52 | 0.55         |
| Lex - EmoLex               | 0.50/0.50 | 0.59/0.50 | 0.54         |
| Gate: LIWC22+LingFeat@0.50 | 0.10/0.10 | 0.58/0.52 | 0.55         |
| Lex - EmoLex               | 0.50/0.50 | 0.59/0.50 | 0.54         |
| Gate: LIWC22+LingFeat@0.10 | 0.10/0.43 | 0.56/0.50 | 0.53         |
| Lex - EmoLex               | 0.50/0.50 | 0.59/0.50 | 0.54         |
| Gate: 2 prev + EmoLex@0.10 | 0.10/0.22 | 0.57/0.52 | 0.55         |
| Lex - EmoLex               | 0.50/0.50 | 0.59/0.50 | 0.55         |
| Gate: 2 prev + LIWC22@0.10 | 0.10/0.26 | 0.57/0.52 | 0.55         |
| Lex - EmoLex               | 0.50/0.50 | 0.59/0.49 | 0.54         |
| Gate: 2 prev + eMFD@0.10   | 0.10/0.19 | 0.57/0.52 | 0.55         |
| Lex - Emotion Intensity    | 0.50/0.50 | 0.59/0.51 | 0.55         |
| Gate: Baseline@0.50        | 0.10/0.10 | 0.59/0.53 | <b>0.56</b>  |
| Lex - Emotion Intensity    | 0.50/0.50 | 0.59/0.51 | 0.55         |
| Gate: LIWC22+LingFeat@0.50 | 0.10/0.10 | 0.59/0.53 | <b>0.56</b>  |
| Lex - Emotion Intensity    | 0.50/0.50 | 0.58/0.52 | 0.55         |
| Gate: LIWC22+LingFeat@0.10 | 0.10/0.45 | 0.57/0.52 | 0.55         |
| Lex - Emotion Intensity    | 0.50/0.50 | 0.58/0.51 | 0.55         |
| Gate: 2 prev + EmoLex@0.10 | 0.10/0.10 | 0.58/0.53 | 0.55         |
| Lex - Emotion Intensity    | 0.50/0.50 | 0.59/0.51 | 0.55         |
| Gate: 2 prev + LIWC22@0.10 | 0.10/0.12 | 0.58/0.53 | 0.55         |
| Lex - Emotion Intensity    | 0.50/0.50 | 0.59/0.51 | 0.55         |
| Gate: 2 prev + eMFD@0.10   | 0.10/0.10 | 0.58/0.53 | 0.55         |

Table S15: Test F1-scores for Social Focus vs. Personal Focus detection with a Presence gate (Part 3/5). Best Macro- $F_1$  values are bolded.

| Configuration              | Thr (S/P) | F1 (S/P)  | Macro- $F_1$ |
|----------------------------|-----------|-----------|--------------|
| Lex - WorryWords           | 0.50/0.50 | 0.59/0.51 | 0.55         |
| Gate: Baseline@0.50        | 0.10/0.10 | 0.59/0.52 | <b>0.56</b>  |
| Lex - WorryWords           | 0.50/0.50 | 0.59/0.52 | 0.55         |
| Gate: LIWC22+LingFeat@0.50 | 0.10/0.10 | 0.59/0.52 | <b>0.56</b>  |
| Lex - WorryWords           | 0.50/0.50 | 0.59/0.51 | 0.55         |
| Gate: LIWC22+LingFeat@0.10 | 0.10/0.64 | 0.58/0.51 | 0.55         |
| Lex - WorryWords           | 0.50/0.50 | 0.59/0.51 | 0.55         |
| Gate: 2 prev + EmoLex@0.10 | 0.10/0.10 | 0.59/0.52 | 0.55         |
| Lex - WorryWords           | 0.50/0.50 | 0.59/0.52 | 0.55         |
| Gate: 2 prev + LIWC22@0.10 | 0.10/0.10 | 0.59/0.52 | <b>0.56</b>  |
| Lex - WorryWords           | 0.50/0.50 | 0.59/0.51 | 0.55         |
| Gate: 2 prev + eMFD@0.10   | 0.10/0.10 | 0.59/0.52 | 0.55         |
| Lex - LIWC 15              | 0.50/0.50 | 0.59/0.49 | 0.54         |
| Gate: Baseline@0.50        | 0.10/0.10 | 0.58/0.53 | 0.55         |
| Lex - LIWC 15              | 0.50/0.50 | 0.60/0.50 | 0.55         |
| Gate: LIWC22+LingFeat@0.50 | 0.10/0.10 | 0.58/0.53 | 0.55         |
| Lex - LIWC 15              | 0.50/0.50 | 0.59/0.50 | 0.55         |
| Gate: LIWC22+LingFeat@0.10 | 0.10/0.40 | 0.56/0.51 | 0.53         |
| Lex - LIWC 15              | 0.50/0.50 | 0.59/0.50 | 0.55         |
| Gate: 2 prev + EmoLex@0.10 | 0.10/0.19 | 0.56/0.53 | 0.55         |
| Lex - LIWC 15              | 0.50/0.50 | 0.59/0.50 | 0.55         |
| Gate: 2 prev + LIWC22@0.10 | 0.10/0.25 | 0.57/0.53 | 0.55         |
| Lex - LIWC 15              | 0.50/0.50 | 0.59/0.50 | 0.55         |
| Gate: 2 prev + eMFD@0.10   | 0.10/0.17 | 0.57/0.53 | 0.55         |
| Lex - MFD                  | 0.50/0.50 | 0.59/0.51 | 0.55         |
| Gate: Baseline@0.50        | 0.10/0.10 | 0.59/0.52 | 0.55         |
| Lex - MFD                  | 0.50/0.50 | 0.59/0.52 | 0.55         |
| Gate: LIWC22+LingFeat@0.50 | 0.10/0.10 | 0.59/0.52 | <b>0.56</b>  |
| Lex - MFD                  | 0.50/0.50 | 0.58/0.51 | 0.55         |
| Gate: LIWC22+LingFeat@0.10 | 0.10/0.81 | 0.58/0.51 | 0.54         |
| Lex - MFD                  | 0.50/0.50 | 0.58/0.52 | 0.55         |
| Gate: 2 prev + EmoLex@0.10 | 0.10/0.10 | 0.58/0.52 | 0.55         |
| Lex - MFD                  | 0.50/0.50 | 0.59/0.52 | 0.55         |
| Gate: 2 prev + LIWC22@0.10 | 0.10/0.15 | 0.58/0.52 | 0.55         |
| Lex - MFD                  | 0.50/0.50 | 0.59/0.51 | 0.55         |
| Gate: 2 prev + eMFD@0.10   | 0.10/0.10 | 0.59/0.52 | 0.55         |

Table S16: Test F1-scores for Social Focus vs. Personal Focus detection with a Presence gate (Part 4/5). Best Macro- $F_1$  values are bolded.

| Configuration              | Thr (S/P) | F1 (S/P)  | Macro- $F_1$ |
|----------------------------|-----------|-----------|--------------|
| Lex - LIWC 22              | 0.50/0.50 | 0.59/0.51 | 0.55         |
| Gate: Baseline@0.50        | 0.10/0.10 | 0.59/0.52 | <b>0.56</b>  |
| Lex - LIWC 22              | 0.50/0.50 | 0.60/0.51 | 0.55         |
| Gate: LIWC22+LingFeat@0.50 | 0.10/0.10 | 0.60/0.52 | <b>0.56</b>  |
| Lex - LIWC 22              | 0.50/0.50 | 0.59/0.51 | 0.55         |
| Gate: LIWC22+LingFeat@0.10 | 0.10/0.60 | 0.58/0.51 | 0.54         |
| Lex - LIWC 22              | 0.50/0.50 | 0.59/0.51 | 0.55         |
| Gate: 2 prev + EmoLex@0.10 | 0.10/0.10 | 0.58/0.52 | 0.55         |
| Lex - LIWC 22              | 0.50/0.50 | 0.59/0.51 | 0.55         |
| Gate: 2 prev + LIWC22@0.10 | 0.10/0.18 | 0.59/0.52 | 0.55         |
| Lex - LIWC 22              | 0.50/0.50 | 0.59/0.51 | 0.55         |
| Gate: 2 prev + eMFD@0.10   | 0.10/0.10 | 0.59/0.52 | 0.55         |
| Lex - LIWC 22 + Ling Feat  | 0.50/0.50 | 0.59/0.50 | 0.55         |
| Gate: Baseline@0.50        | 0.10/0.10 | 0.59/0.52 | 0.55         |
| Lex - LIWC 22 + Ling Feat  | 0.50/0.50 | 0.59/0.51 | 0.55         |
| Gate: LIWC22+LingFeat@0.50 | 0.10/0.10 | 0.59/0.52 | <b>0.56</b>  |
| Lex - LIWC 22 + Ling Feat  | 0.50/0.50 | 0.58/0.51 | 0.54         |
| Gate: LIWC22+LingFeat@0.10 | 0.10/0.59 | 0.58/0.51 | 0.54         |
| Lex - LIWC 22 + Ling Feat  | 0.50/0.50 | 0.58/0.51 | 0.55         |
| Gate: 2 prev + EmoLex@0.10 | 0.10/0.10 | 0.58/0.52 | 0.55         |
| Lex - LIWC 22 + Ling Feat  | 0.50/0.50 | 0.58/0.51 | 0.55         |
| Gate: 2 prev + LIWC22@0.10 | 0.10/0.11 | 0.58/0.52 | 0.55         |
| Lex - LIWC 22 + Ling Feat  | 0.50/0.50 | 0.58/0.51 | 0.55         |
| Gate: 2 prev + eMFD@0.10   | 0.10/0.10 | 0.59/0.52 | 0.55         |
| Lex - MFD-20               | 0.50/0.50 | 0.59/0.52 | 0.55         |
| Gate: Baseline@0.50        | 0.10/0.10 | 0.59/0.53 | <b>0.56</b>  |
| Lex - MFD-20               | 0.50/0.50 | 0.59/0.52 | <b>0.56</b>  |
| Gate: LIWC22+LingFeat@0.50 | 0.10/0.10 | 0.59/0.53 | <b>0.56</b>  |
| Lex - MFD-20               | 0.50/0.50 | 0.58/0.52 | 0.55         |
| Gate: LIWC22+LingFeat@0.10 | 0.10/0.57 | 0.58/0.51 | 0.55         |
| Lex - MFD-20               | 0.50/0.50 | 0.58/0.52 | 0.55         |
| Gate: 2 prev + EmoLex@0.10 | 0.10/0.10 | 0.58/0.53 | 0.55         |
| Lex - MFD-20               | 0.50/0.50 | 0.59/0.52 | 0.55         |
| Gate: 2 prev + LIWC22@0.10 | 0.10/0.10 | 0.58/0.53 | <b>0.56</b>  |
| Lex - MFD-20               | 0.50/0.50 | 0.59/0.52 | 0.55         |
| Gate: 2 prev + eMFD@0.10   | 0.10/0.10 | 0.58/0.52 | 0.55         |



Table S17: Test F1-scores for Social Focus vs. Personal Focus detection with a Presence gate (Part 5/5). Best Macro- $F_1$  values are bolded.

| Configuration              | Thr (S/P) | F1 (S/P)  | Macro- $F_1$ |
|----------------------------|-----------|-----------|--------------|
| TD - LDA                   | 0.50/0.50 | 0.59/0.50 | 0.55         |
| Gate: Baseline@0.50        | 0.10/0.12 | 0.58/0.52 | 0.55         |
| TD - LDA                   | 0.50/0.50 | 0.59/0.51 | 0.55         |
| Gate: LIWC22+LingFeat@0.50 | 0.10/0.11 | 0.58/0.52 | 0.55         |
| TD - LDA                   | 0.50/0.50 | 0.58/0.51 | 0.55         |
| Gate: LIWC22+LingFeat@0.10 | 0.10/0.38 | 0.55/0.52 | 0.54         |
| TD - LDA                   | 0.50/0.50 | 0.59/0.51 | 0.55         |
| Gate: 2 prev + EmoLex@0.10 | 0.10/0.21 | 0.56/0.52 | 0.54         |
| TD - LDA                   | 0.50/0.50 | 0.59/0.51 | 0.55         |
| Gate: 2 prev + LIWC22@0.10 | 0.10/0.25 | 0.56/0.52 | 0.54         |
| TD - LDA                   | 0.50/0.50 | 0.59/0.50 | 0.55         |
| Gate: 2 prev + eMFD@0.10   | 0.10/0.19 | 0.57/0.52 | 0.54         |
| TD - NMF                   | 0.50/0.50 | 0.59/0.50 | 0.55         |
| Gate: Baseline@0.50        | 0.10/0.13 | 0.57/0.52 | 0.55         |
| TD - NMF                   | 0.50/0.50 | 0.59/0.50 | 0.55         |
| Gate: LIWC22+LingFeat@0.50 | 0.10/0.12 | 0.57/0.52 | 0.55         |
| TD - NMF                   | 0.50/0.50 | 0.58/0.51 | 0.54         |
| Gate: LIWC22+LingFeat@0.10 | 0.10/0.39 | 0.55/0.52 | 0.53         |
| TD - NMF                   | 0.50/0.50 | 0.59/0.50 | 0.54         |
| Gate: 2 prev + EmoLex@0.10 | 0.10/0.24 | 0.56/0.53 | 0.54         |
| TD - NMF                   | 0.50/0.50 | 0.59/0.51 | 0.55         |
| Gate: 2 prev + LIWC22@0.10 | 0.10/0.27 | 0.56/0.52 | 0.54         |
| TD - NMF                   | 0.50/0.50 | 0.59/0.50 | 0.54         |
| Gate: 2 prev + eMFD@0.10   | 0.10/0.21 | 0.56/0.52 | 0.54         |
| TD - BERTopic              | 0.50/0.50 | 0.59/0.49 | 0.54         |
| Gate: Baseline@0.50        | 0.10/0.14 | 0.57/0.52 | 0.55         |
| TD - BERTopic              | 0.50/0.50 | 0.60/0.49 | 0.55         |
| Gate: LIWC22+LingFeat@0.50 | 0.10/0.13 | 0.58/0.53 | 0.55         |
| TD - BERTopic              | 0.50/0.50 | 0.58/0.50 | 0.54         |
| Gate: LIWC22+LingFeat@0.10 | 0.10/0.40 | 0.55/0.51 | 0.53         |
| TD - BERTopic              | 0.50/0.50 | 0.59/0.50 | 0.54         |
| Gate: 2 prev + EmoLex@0.10 | 0.10/0.24 | 0.56/0.52 | 0.54         |
| TD - BERTopic              | 0.50/0.50 | 0.59/0.50 | 0.55         |
| Gate: 2 prev + LIWC22@0.10 | 0.10/0.28 | 0.56/0.50 | 0.54         |
| TD - BERTopic              | 0.50/0.50 | 0.59/0.49 | 0.54         |
| Gate: 2 prev + eMFD@0.10   | 0.10/0.22 | 0.56/0.52 | 0.54         |

Table S18: Validation F1-scores for Openness to Change vs. Conservation detection with a Presence gate (macro-average over the two classes).

| <b>Model</b>                       | <b>Openness</b> | <b>Conservation</b> | <b>Macro-<math>F_1</math></b> |
|------------------------------------|-----------------|---------------------|-------------------------------|
| Baseline                           | 0.45            | 0.68                | 0.57                          |
| Token Pruning                      | 0.45            | 0.68                | 0.57                          |
| 2 prev sent w/ label               | 0.43            | 0.66                | 0.55                          |
| MultiLayer                         | 0.46            | 0.67                | 0.57                          |
| Residual Block                     | 0.45            | 0.70                | 0.57                          |
| Data Augmentation                  | 0.30            | 0.58                | 0.44                          |
| Custom Stopwords                   | 0.45            | 0.68                | 0.57                          |
| NER                                | 0.47            | 0.67                | 0.57                          |
| Lex - Schwartz                     | 0.46            | 0.68                | 0.57                          |
| Lex - VAD                          | 0.47            | 0.67                | 0.57                          |
| Lex - EmoLex                       | 0.45            | 0.66                | 0.56                          |
| Lex - Emotion Intensity            | 0.47            | 0.69                | 0.58                          |
| Lex - WorryWords                   | 0.47            | 0.67                | 0.57                          |
| Lex - LIWC 15                      | 0.48            | 0.68                | 0.58                          |
| Lex - MFD                          | 0.46            | 0.68                | 0.57                          |
| Lex - LIWC 22                      | 0.46            | 0.69                | 0.57                          |
| Lex - LIWC 22 + Ling Feat          | 0.46            | 0.69                | 0.57                          |
| Lex - MFD-20                       | 0.47            | 0.66                | 0.56                          |
| Lex - eMFD                         | 0.46            | 0.67                | 0.57                          |
| Lex - MJD                          | 0.47            | 0.67                | 0.57                          |
| TD - LDA                           | 0.48            | 0.67                | 0.57                          |
| TD - NMF                           | 0.49            | 0.67                | 0.58                          |
| TD - BERTopic                      | 0.47            | 0.67                | 0.57                          |
| NER + Lex - VAD                    | 0.46            | 0.69                | 0.57                          |
| NER + Lex - Emotion Inten-<br>sity | 0.48            | 0.69                | 0.58                          |
| NER + Lex - LIWC 15                | 0.46            | 0.69                | 0.57                          |
| NER + TD - NMF                     | 0.46            | 0.68                | 0.57                          |

Table S19: Test F1-scores for Openness to Change vs. Conservation detection with a Presence gate (Part 1/3). Best Macro- $F_1$  values are bolded.

| Configuration              | Thr (O/C) | F1 (O/C)  | Macro- $F_1$ |
|----------------------------|-----------|-----------|--------------|
| Baseline                   | 0.50/0.50 | 0.31/0.52 | 0.413        |
| Gate: Baseline@0.50        | 0.78/0.12 | 0.27/0.50 | 0.381        |
| Baseline                   | 0.50/0.50 | 0.30/0.52 | 0.412        |
| Gate: LIWC22+LingFeat@0.50 | 0.73/0.12 | 0.27/0.50 | 0.384        |
| Baseline                   | 0.50/0.50 | 0.32/0.51 | 0.416        |
| Gate: LIWC22+LingFeat@0.10 | 0.50/0.35 | 0.32/0.51 | 0.414        |
| Baseline                   | 0.50/0.50 | 0.31/0.51 | 0.413        |
| Gate: 2 prev + EmoLex@0.10 | 0.88/0.23 | 0.23/0.50 | 0.365        |
| Baseline                   | 0.50/0.50 | 0.32/0.52 | 0.420        |
| Gate: 2 prev + LIWC22@0.10 | 0.50/0.27 | 0.32/0.51 | 0.414        |
| Baseline                   | 0.50/0.50 | 0.32/0.51 | 0.414        |
| Gate: 2 prev + eMFD@0.10   | 0.87/0.23 | 0.23/0.50 | 0.365        |
| NER                        | 0.50/0.50 | 0.32/0.52 | 0.421        |
| Gate: Baseline@0.50        | 0.79/0.13 | 0.28/0.49 | 0.386        |
| NER                        | 0.50/0.50 | 0.32/0.52 | 0.420        |
| Gate: LIWC22+LingFeat@0.50 | 0.77/0.12 | 0.28/0.50 | 0.391        |
| NER                        | 0.50/0.50 | 0.34/0.51 | 0.422        |
| Gate: LIWC22+LingFeat@0.10 | 0.50/0.40 | 0.34/0.51 | 0.420        |
| NER                        | 0.50/0.50 | 0.33/0.51 | 0.420        |
| Gate: 2 prev + EmoLex@0.10 | 0.87/0.23 | 0.26/0.49 | 0.376        |
| NER                        | 0.50/0.50 | 0.33/0.52 | 0.423        |
| Gate: 2 prev + LIWC22@0.10 | 0.89/0.27 | 0.26/0.50 | 0.381        |
| NER                        | 0.50/0.50 | 0.33/0.51 | 0.421        |
| Gate: 2 prev + eMFD@0.10   | 0.83/0.23 | 0.28/0.50 | 0.386        |
| Lex - VAD                  | 0.50/0.50 | 0.32/0.53 | 0.424        |
| Gate: Baseline@0.50        | 0.79/0.11 | 0.28/0.50 | 0.387        |
| Lex - VAD                  | 0.50/0.50 | 0.32/0.53 | 0.425        |
| Gate: LIWC22+LingFeat@0.50 | 0.79/0.10 | 0.27/0.50 | 0.386        |
| Lex - VAD                  | 0.50/0.50 | 0.33/0.52 | 0.426        |
| Gate: LIWC22+LingFeat@0.10 | 0.50/0.32 | 0.33/0.50 | 0.419        |
| Lex - VAD                  | 0.50/0.50 | 0.33/0.52 | 0.424        |
| Gate: 2 prev + EmoLex@0.10 | 0.88/0.20 | 0.25/0.50 | 0.375        |
| Lex - VAD                  | 0.50/0.50 | 0.33/0.53 | 0.429        |
| Gate: 2 prev + LIWC22@0.10 | 0.89/0.23 | 0.26/0.50 | 0.382        |
| Lex - VAD                  | 0.50/0.50 | 0.33/0.52 | 0.423        |
| Gate: 2 prev + eMFD@0.10   | 0.86/0.19 | 0.26/0.50 | 0.380        |

Table S20: Test F1-scores for Openness to Change vs. Conservation detection with a Presence gate (Part 2/3). Best Macro- $F_1$  values are bolded.

| Configuration              | Thr (O/C) | F1 (O/C)  | Macro- $F_1$ |
|----------------------------|-----------|-----------|--------------|
| Lex - Emotion Intensity    | 0.50/0.50 | 0.31/0.53 | 0.421        |
| Gate: Baseline@0.50        | 0.58/0.18 | 0.30/0.50 | 0.401        |
| Lex - Emotion Intensity    | 0.50/0.50 | 0.32/0.53 | 0.422        |
| Gate: LIWC22+LingFeat@0.50 | 0.58/0.17 | 0.30/0.50 | 0.402        |
| Lex - Emotion Intensity    | 0.50/0.50 | 0.34/0.52 | 0.427        |
| Gate: LIWC22+LingFeat@0.10 | 0.82/0.41 | 0.23/0.51 | 0.370        |
| Lex - Emotion Intensity    | 0.50/0.50 | 0.33/0.52 | 0.425        |
| Gate: 2 prev + EmoLex@0.10 | 0.72/0.27 | 0.26/0.50 | 0.377        |
| Lex - Emotion Intensity    | 0.50/0.50 | 0.34/0.52 | <b>0.430</b> |
| Gate: 2 prev + LIWC22@0.10 | 0.75/0.32 | 0.26/0.51 | 0.384        |
| Lex - Emotion Intensity    | 0.50/0.50 | 0.33/0.52 | 0.424        |
| Gate: 2 prev + eMFD@0.10   | 0.70/0.27 | 0.27/0.50 | 0.386        |
| Lex - LIWC 15              | 0.50/0.50 | 0.32/0.52 | 0.422        |
| Gate: Baseline@0.50        | 0.84/0.12 | 0.27/0.50 | 0.385        |
| Lex - LIWC 15              | 0.50/0.50 | 0.32/0.52 | 0.422        |
| Gate: LIWC22+LingFeat@0.50 | 0.83/0.11 | 0.28/0.50 | 0.389        |
| Lex - LIWC 15              | 0.50/0.50 | 0.33/0.51 | 0.422        |
| Gate: LIWC22+LingFeat@0.10 | 0.50/0.36 | 0.33/0.50 | 0.418        |
| Lex - LIWC 15              | 0.50/0.50 | 0.33/0.52 | 0.421        |
| Gate: 2 prev + EmoLex@0.10 | 0.50/0.20 | 0.33/0.49 | 0.411        |
| Lex - LIWC 15              | 0.50/0.50 | 0.33/0.52 | 0.424        |
| Gate: 2 prev + LIWC22@0.10 | 0.50/0.23 | 0.33/0.50 | 0.417        |
| Lex - LIWC 15              | 0.50/0.50 | 0.33/0.51 | 0.421        |
| Gate: 2 prev + eMFD@0.10   | 0.88/0.20 | 0.27/0.50 | 0.383        |
| TD - NMF                   | 0.50/0.50 | 0.32/0.52 | 0.423        |
| Gate: Baseline@0.50        | 0.80/0.15 | 0.27/0.50 | 0.383        |
| TD - NMF                   | 0.50/0.50 | 0.32/0.52 | 0.424        |
| Gate: LIWC22+LingFeat@0.50 | 0.79/0.13 | 0.28/0.50 | 0.388        |
| TD - NMF                   | 0.50/0.50 | 0.34/0.51 | 0.426        |
| Gate: LIWC22+LingFeat@0.10 | 0.50/0.40 | 0.34/0.51 | 0.424        |
| TD - NMF                   | 0.50/0.50 | 0.33/0.52 | 0.426        |
| Gate: 2 prev + EmoLex@0.10 | 0.88/0.25 | 0.25/0.50 | 0.375        |
| TD - NMF                   | 0.50/0.50 | 0.34/0.52 | 0.428        |
| Gate: 2 prev + LIWC22@0.10 | 0.50/0.28 | 0.34/0.50 | 0.420        |
| TD - NMF                   | 0.50/0.50 | 0.34/0.51 | 0.425        |
| Gate: 2 prev + eMFD@0.10   | 0.87/0.25 | 0.26/0.50 | 0.377        |

Table S21: Test F1-scores for Openness to Change vs. Conservation detection with a Presence gate (Part 3/3). Best Macro- $F_1$  values are bolded.

| <b>Configuration</b>          | <b>Thr (O/C)</b> | <b>F1 (O/C)</b> | <b>Macro-<math>F_1</math></b> |
|-------------------------------|------------------|-----------------|-------------------------------|
| NER + Lex - VAD               | 0.50/0.50        | 0.31/0.52       | 0.415                         |
| Gate: Baseline@0.50           | 0.76/0.13        | 0.27/0.50       | 0.385                         |
| NER + Lex - VAD               | 0.50/0.50        | 0.31/0.52       | 0.414                         |
| Gate: LIWC22+LingFeat@0.50    | 0.76/0.12        | 0.27/0.50       | 0.384                         |
| NER + Lex - VAD               | 0.50/0.50        | 0.33/0.51       | 0.419                         |
| Gate: LIWC22+LingFeat@0.10    | 0.50/0.35        | 0.33/0.50       | 0.415                         |
| NER + Lex - VAD               | 0.50/0.50        | 0.32/0.52       | 0.416                         |
| Gate: 2 prev + EmoLex@0.10    | 0.88/0.22        | 0.23/0.50       | 0.362                         |
| NER + Lex - VAD               | 0.50/0.50        | 0.32/0.52       | 0.421                         |
| Gate: 2 prev + LIWC22@0.10    | 0.50/0.26        | 0.32/0.50       | 0.413                         |
| NER + Lex - VAD               | 0.50/0.50        | 0.32/0.51       | 0.416                         |
| Gate: 2 prev + eMFD@0.10      | 0.84/0.23        | 0.25/0.50       | 0.376                         |
| NER + Lex - Emotion Intensity | 0.50/0.50        | 0.31/0.52       | 0.415                         |
| Gate: Baseline@0.50           | 0.83/0.14        | 0.26/0.50       | 0.379                         |
| NER + Lex - Emotion Intensity | 0.50/0.50        | 0.31/0.52       | 0.415                         |
| Gate: LIWC22+LingFeat@0.50    | 0.83/0.13        | 0.25/0.50       | 0.376                         |
| NER + Lex - Emotion Intensity | 0.50/0.50        | 0.32/0.51       | 0.416                         |
| Gate: LIWC22+LingFeat@0.10    | 0.50/0.36        | 0.32/0.50       | 0.411                         |
| NER + Lex - Emotion Intensity | 0.50/0.50        | 0.31/0.51       | 0.413                         |
| Gate: 2 prev + EmoLex@0.10    | 0.50/0.23        | 0.31/0.50       | 0.404                         |
| NER + Lex - Emotion Intensity | 0.50/0.50        | 0.31/0.52       | 0.416                         |
| Gate: 2 prev + LIWC22@0.10    | 0.50/0.28        | 0.31/0.50       | 0.409                         |
| NER + Lex - Emotion Intensity | 0.50/0.50        | 0.31/0.51       | 0.413                         |
| Gate: 2 prev + eMFD@0.10      | 0.50/0.24        | 0.31/0.50       | 0.405                         |

Table S22: Validation F1-scores for Self-Transcendence vs. Self-Enhancement detection with a Presence gate (macro-average over the two classes).

| <b>Model</b>                         | <b>Self-Trans.</b> | <b>Self-Enh.</b> | <b>Macro-<math>F_1</math></b> |
|--------------------------------------|--------------------|------------------|-------------------------------|
| Baseline                             | 0.57               | 0.61             | 0.59                          |
| Token Pruning                        | 0.54               | 0.63             | 0.58                          |
| 2 prev sent w/ label                 | 0.57               | 0.58             | 0.57                          |
| MultiLayer                           | 0.58               | 0.60             | 0.59                          |
| Residual Block                       | 0.58               | 0.58             | 0.58                          |
| Data Augmentation                    | 0.46               | 0.55             | 0.50                          |
| Custom Stopwords                     | 0.57               | 0.61             | 0.59                          |
| NER                                  | 0.58               | 0.59             | 0.58                          |
| Lex - Schwartz                       | 0.57               | 0.59             | 0.58                          |
| Lex - VAD                            | 0.57               | 0.61             | 0.59                          |
| Lex - EmoLex                         | 0.57               | 0.60             | 0.58                          |
| Lex - Emotion Intensity              | 0.56               | 0.60             | 0.58                          |
| Lex - WorryWords                     | 0.57               | 0.60             | 0.58                          |
| Lex - LIWC 15                        | 0.56               | 0.62             | 0.59                          |
| Lex - MFD                            | 0.57               | 0.58             | 0.57                          |
| Lex - LIWC 22                        | 0.57               | 0.59             | 0.58                          |
| Lex - LIWC 22 + Ling Feat            | 0.56               | 0.60             | 0.58                          |
| Lex - MFD-20                         | 0.57               | 0.60             | 0.58                          |
| Lex - eMFD                           | 0.56               | 0.60             | 0.58                          |
| Lex - MJD                            | 0.57               | 0.60             | 0.58                          |
| TD - LDA                             | 0.56               | 0.60             | 0.58                          |
| TD - NMF                             | 0.58               | 0.58             | 0.58                          |
| TD - BERTopic                        | 0.58               | 0.58             | 0.58                          |
| MultiLayer + NER                     | 0.57               | 0.61             | 0.59                          |
| MultiLayer + Lex - VAD               | 0.58               | 0.60             | 0.59                          |
| MultiLayer + Lex - Emotion Intensity | 0.58               | 0.61             | 0.60                          |
| MultiLayer + Lex - WorryWords        | 0.57               | 0.60             | 0.58                          |
| MultiLayer + Lex - LIWC 15           | 0.55               | 0.61             | 0.58                          |
| MultiLayer + Lex - LIWC 22           | 0.57               | 0.62             | 0.60                          |
| NER + Lex - VAD                      | 0.56               | 0.60             | 0.58                          |
| NER + Lex - Emotion Intensity        | 0.55               | 0.62             | 0.58                          |
| NER + Lex - WorryWords               | 0.58               | 0.59             | 0.58                          |
| NER + Lex - LIWC 15                  | 0.55               | 0.61             | 0.58                          |
| NER + Lex - LIWC 22                  | 0.57               | 0.61             | 0.59                          |

Table S23: Test F1-scores for Self-Transcendence vs. Self-Enhancement detection with a Presence gate (Part 1/8). Thr and F1 are reported as Self-Transcendence/Self-Enhancement pairs; Macro- $F_1$  is the macro-average over the two classes. Best Macro- $F_1$  values are bolded.

| Configuration              | Thr (ST/SE) | F1 (ST/SE) | Macro- $F_1$ |
|----------------------------|-------------|------------|--------------|
| Baseline                   | 0.50/0.50   | 0.50/0.47  | 0.49         |
| Gate: Baseline@0.50        | 0.18/0.36   | 0.50/0.47  | 0.49         |
| Baseline                   | 0.50/0.50   | 0.50/0.47  | 0.49         |
| Gate: LIWC22+LingFeat@0.50 | 0.18/0.33   | 0.50/0.48  | 0.49         |
| Baseline                   | 0.50/0.50   | 0.51/0.46  | 0.49         |
| Gate: LIWC22+LingFeat@0.10 | 0.34/0.73   | 0.51/0.45  | 0.48         |
| Baseline                   | 0.50/0.50   | 0.51/0.47  | 0.49         |
| Gate: 2 prev + EmoLex@0.10 | 0.27/0.57   | 0.50/0.46  | 0.48         |
| Baseline                   | 0.50/0.50   | 0.51/0.47  | 0.49         |
| Gate: 2 prev + LIWC22@0.10 | 0.27/0.62   | 0.50/0.46  | 0.48         |
| Baseline                   | 0.50/0.50   | 0.51/0.46  | 0.48         |
| Gate: 2 prev + eMFD@0.10   | 0.22/0.52   | 0.50/0.46  | 0.48         |
| Lex - Emotion Intensity    | 0.50/0.50   | 0.52/0.45  | 0.49         |
| Gate: Baseline@0.50        | 0.26/0.29   | 0.51/0.48  | 0.49         |
| Lex - Emotion Intensity    | 0.50/0.50   | 0.52/0.45  | 0.49         |
| Gate: LIWC22+LingFeat@0.50 | 0.26/0.28   | 0.51/0.48  | 0.49         |
| Lex - Emotion Intensity    | 0.50/0.50   | 0.53/0.46  | 0.49         |
| Gate: LIWC22+LingFeat@0.10 | 0.37/0.51   | 0.52/0.46  | 0.49         |
| Lex - Emotion Intensity    | 0.50/0.50   | 0.52/0.46  | 0.49         |
| Gate: 2 prev + EmoLex@0.10 | 0.33/0.42   | 0.52/0.47  | 0.49         |
| Lex - Emotion Intensity    | 0.50/0.50   | 0.53/0.46  | 0.49         |
| Gate: 2 prev + LIWC22@0.10 | 0.32/0.45   | 0.52/0.47  | 0.49         |
| Lex - Emotion Intensity    | 0.50/0.50   | 0.52/0.45  | 0.49         |
| Gate: 2 prev + eMFD@0.10   | 0.29/0.39   | 0.52/0.46  | 0.49         |

Table S24: Test F1-scores for Self-Transcendence vs. Self-Enhancement detection with a Presence gate (Part 2/8). Thr and F1 are reported as Self-Transcendence/Self-Enhancement pairs; Macro- $F_1$  is the macro-average over the two classes. Best Macro- $F_1$  values are bolded.

| Configuration              | Thr (ST/SE) | F1 (ST/SE) | Macro- $F_1$ |
|----------------------------|-------------|------------|--------------|
| Lex - WorryWords           | 0.50/0.50   | 0.51/0.46  | 0.49         |
| Gate: Baseline@0.50        | 0.17/0.30   | 0.51/0.48  | <b>0.50</b>  |
| Lex - WorryWords           | 0.50/0.50   | 0.51/0.45  | 0.48         |
| Gate: LIWC22+LingFeat@0.50 | 0.16/0.27   | 0.51/0.48  | <b>0.50</b>  |
| Lex - WorryWords           | 0.50/0.50   | 0.52/0.46  | 0.49         |
| Gate: LIWC22+LingFeat@0.10 | 0.25/0.51   | 0.53/0.46  | 0.39         |
| Lex - WorryWords           | 0.50/0.50   | 0.52/0.46  | 0.49         |
| Gate: 2 prev + EmoLex@0.10 | 0.21/0.41   | 0.52/0.47  | <b>0.50</b>  |
| Lex - WorryWords           | 0.50/0.50   | 0.52/0.46  | 0.49         |
| Gate: 2 prev + LIWC22@0.10 | 0.21/0.44   | 0.52/0.47  | 0.49         |
| Lex - WorryWords           | 0.50/0.50   | 0.52/0.45  | 0.48         |
| Gate: 2 prev + eMFD@0.10   | 0.19/0.39   | 0.52/0.47  | 0.49         |
| Lex - LIWC 22              | 0.50/0.50   | 0.51/0.46  | 0.49         |
| Gate: Baseline@0.50        | 0.18/0.30   | 0.51/0.48  | <b>0.50</b>  |
| Lex - LIWC 22              | 0.50/0.50   | 0.51/0.46  | 0.49         |
| Gate: LIWC22+LingFeat@0.50 | 0.18/0.28   | 0.51/0.48  | <b>0.50</b>  |
| Lex - LIWC 22              | 0.50/0.50   | 0.52/0.46  | 0.49         |
| Gate: LIWC22+LingFeat@0.10 | 0.29/0.54   | 0.52/0.46  | 0.49         |
| Lex - LIWC 22              | 0.50/0.50   | 0.52/0.46  | 0.49         |
| Gate: 2 prev + EmoLex@0.10 | 0.24/0.43   | 0.52/0.47  | <b>0.50</b>  |
| Lex - LIWC 22              | 0.50/0.50   | 0.52/0.46  | 0.49         |
| Gate: 2 prev + LIWC22@0.10 | 0.23/0.46   | 0.52/0.47  | 0.49         |
| Lex - LIWC 22              | 0.50/0.50   | 0.52/0.46  | 0.49         |
| Gate: 2 prev + eMFD@0.10   | 0.21/0.42   | 0.52/0.47  | 0.49         |



Table S25: Test F1-scores for Self-Transcendence vs. Self-Enhancement detection with a Presence gate (Part 3/8). Thr and F1 are reported as Self-Transcendence/Self-Enhancement pairs; Macro- $F_1$  is the macro-average over the two classes. Best Macro- $F_1$  values are bolded.

| Configuration                   | Thr (ST/SE) | F1 (ST/SE) | Macro- $F_1$ |
|---------------------------------|-------------|------------|--------------|
| MultiLayer + Lex - Emotion Int. | 0.50/0.50   | 0.51/0.47  | 0.49         |
| Gate: Baseline@0.50             | 0.20/0.29   | 0.51/0.48  | <b>0.50</b>  |
| MultiLayer + Lex - Emotion Int. | 0.50/0.50   | 0.51/0.47  | 0.49         |
| Gate: LIWC22+LingFeat@0.50      | 0.20/0.27   | 0.51/0.48  | <b>0.50</b>  |
| MultiLayer + Lex - Emotion Int. | 0.50/0.50   | 0.52/0.47  | <b>0.50</b>  |
| Gate: LIWC22+LingFeat@0.10      | 0.34/0.58   | 0.53/0.46  | <b>0.50</b>  |
| MultiLayer + Lex - Emotion Int. | 0.50/0.50   | 0.52/0.47  | 0.49         |
| Gate: 2 prev + EmoLex@0.10      | 0.27/0.45   | 0.52/0.47  | <b>0.50</b>  |
| MultiLayer + Lex - Emotion Int. | 0.50/0.50   | 0.52/0.47  | <b>0.50</b>  |
| Gate: 2 prev + LIWC22@0.10      | 0.28/0.48   | 0.53/0.48  | <b>0.50</b>  |
| MultiLayer + Lex - Emotion Int. | 0.50/0.50   | 0.52/0.46  | 0.49         |
| Gate: 2 prev + eMFD@0.10        | 0.23/0.42   | 0.52/0.47  | <b>0.50</b>  |
| MultiLayer + Lex - LIWC 22      | 0.50/0.50   | 0.50/0.47  | 0.48         |
| Gate: Baseline@0.50             | 0.13/0.35   | 0.51/0.48  | 0.49         |
| MultiLayer + Lex - LIWC 22      | 0.50/0.50   | 0.50/0.47  | 0.48         |
| Gate: LIWC22+LingFeat@0.50      | 0.13/0.34   | 0.51/0.48  | 0.49         |
| MultiLayer + Lex - LIWC 22      | 0.50/0.50   | 0.51/0.47  | 0.49         |
| Gate: LIWC22+LingFeat@0.10      | 0.27/0.70   | 0.52/0.46  | 0.49         |
| MultiLayer + Lex - LIWC 22      | 0.50/0.50   | 0.50/0.47  | 0.49         |
| Gate: 2 prev + EmoLex@0.10      | 0.20/0.54   | 0.51/0.47  | 0.49         |
| MultiLayer + Lex - LIWC 22      | 0.50/0.50   | 0.51/0.47  | 0.49         |
| Gate: 2 prev + LIWC22@0.10      | 0.20/0.59   | 0.52/0.46  | 0.49         |
| MultiLayer + Lex - LIWC 22      | 0.50/0.50   | 0.50/0.46  | 0.48         |
| Gate: 2 prev + eMFD@0.10        | 0.16/0.50   | 0.51/0.46  | 0.49         |

Table S26: Test F1-scores for Social Focus vs. Personal Focus detection with a Presence gate (Part 4/8). Thr and F1 are reported as Social/Personal pairs; Macro- $F_1$  is the macro-average over the two classes. Best Macro- $F_1$  values are bolded.

| Configuration              | Thr (S/P) | F1 (S/P)  | Macro- $F_1$ |
|----------------------------|-----------|-----------|--------------|
| Lex - LIWC 15              | 0.50/0.50 | 0.59/0.49 | 0.54         |
| Gate: Baseline@0.50        | 0.10/0.10 | 0.58/0.53 | 0.55         |
| Lex - LIWC 15              | 0.50/0.50 | 0.60/0.50 | 0.55         |
| Gate: LIWC22+LingFeat@0.50 | 0.10/0.10 | 0.58/0.53 | 0.55         |
| Lex - LIWC 15              | 0.50/0.50 | 0.59/0.50 | 0.55         |
| Gate: LIWC22+LingFeat@0.10 | 0.10/0.40 | 0.56/0.51 | 0.53         |
| Lex - LIWC 15              | 0.50/0.50 | 0.59/0.50 | 0.55         |
| Gate: 2 prev + EmoLex@0.10 | 0.10/0.19 | 0.56/0.53 | 0.55         |
| Lex - LIWC 15              | 0.50/0.50 | 0.59/0.50 | 0.55         |
| Gate: 2 prev + LIWC22@0.10 | 0.10/0.25 | 0.57/0.53 | 0.55         |
| Lex - LIWC 15              | 0.50/0.50 | 0.59/0.50 | 0.55         |
| Gate: 2 prev + eMFD@0.10   | 0.10/0.17 | 0.57/0.53 | 0.55         |
| Lex - MFD                  | 0.50/0.50 | 0.59/0.51 | 0.55         |
| Gate: Baseline@0.50        | 0.10/0.10 | 0.59/0.52 | 0.55         |
| Lex - MFD                  | 0.50/0.50 | 0.59/0.52 | 0.55         |
| Gate: LIWC22+LingFeat@0.50 | 0.10/0.10 | 0.59/0.52 | <b>0.56</b>  |
| Lex - MFD                  | 0.50/0.50 | 0.58/0.51 | 0.55         |
| Gate: LIWC22+LingFeat@0.10 | 0.10/0.81 | 0.58/0.51 | 0.54         |
| Lex - MFD                  | 0.50/0.50 | 0.58/0.52 | 0.55         |
| Gate: 2 prev + EmoLex@0.10 | 0.10/0.10 | 0.58/0.52 | 0.55         |
| Lex - MFD                  | 0.50/0.50 | 0.59/0.52 | 0.55         |
| Gate: 2 prev + LIWC22@0.10 | 0.10/0.15 | 0.58/0.52 | 0.55         |
| Lex - MFD                  | 0.50/0.50 | 0.59/0.51 | 0.55         |
| Gate: 2 prev + eMFD@0.10   | 0.10/0.10 | 0.59/0.52 | 0.55         |
| Lex - LIWC 22              | 0.50/0.50 | 0.59/0.51 | 0.55         |
| Gate: Baseline@0.50        | 0.10/0.10 | 0.59/0.52 | <b>0.56</b>  |
| Lex - LIWC 22              | 0.50/0.50 | 0.60/0.51 | 0.55         |
| Gate: LIWC22+LingFeat@0.50 | 0.10/0.10 | 0.60/0.52 | <b>0.56</b>  |
| Lex - LIWC 22              | 0.50/0.50 | 0.59/0.51 | 0.55         |
| Gate: LIWC22+LingFeat@0.10 | 0.10/0.60 | 0.58/0.51 | 0.54         |
| Lex - LIWC 22              | 0.50/0.50 | 0.59/0.51 | 0.55         |
| Gate: 2 prev + EmoLex@0.10 | 0.10/0.10 | 0.58/0.52 | 0.55         |
| Lex - LIWC 22              | 0.50/0.50 | 0.59/0.51 | 0.55         |
| Gate: 2 prev + LIWC22@0.10 | 0.10/0.18 | 0.59/0.52 | 0.55         |
| Lex - LIWC 22              | 0.50/0.50 | 0.59/0.51 | 0.55         |
| Gate: 2 prev + eMFD@0.10   | 0.10/0.10 | 0.59/0.52 | 0.55         |

Table S27: Test F1-scores for Social Focus vs. Personal Focus detection with a Presence gate (Part 5/8). Thr and F1 are reported as Social/Personal pairs; Macro- $F_1$  is the macro-average over the two classes. Best Macro- $F_1$  values are bolded.

| Configuration              | Thr (S/P) | F1 (S/P)  | Macro- $F_1$ |
|----------------------------|-----------|-----------|--------------|
| Lex - LIWC 22 + Ling Feat  | 0.50/0.50 | 0.59/0.50 | 0.55         |
| Gate: Baseline@0.50        | 0.10/0.10 | 0.59/0.52 | 0.55         |
| Lex - LIWC 22 + Ling Feat  | 0.50/0.50 | 0.59/0.51 | 0.55         |
| Gate: LIWC22+LingFeat@0.50 | 0.10/0.10 | 0.59/0.52 | <b>0.56</b>  |
| Lex - LIWC 22 + Ling Feat  | 0.50/0.50 | 0.58/0.51 | 0.54         |
| Gate: LIWC22+LingFeat@0.10 | 0.10/0.59 | 0.58/0.51 | 0.54         |
| Lex - LIWC 22 + Ling Feat  | 0.50/0.50 | 0.58/0.51 | 0.55         |
| Gate: 2 prev + EmoLex@0.10 | 0.10/0.10 | 0.58/0.52 | 0.55         |
| Lex - LIWC 22 + Ling Feat  | 0.50/0.50 | 0.58/0.51 | 0.55         |
| Gate: 2 prev + LIWC22@0.10 | 0.10/0.11 | 0.58/0.52 | 0.55         |
| Lex - LIWC 22 + Ling Feat  | 0.50/0.50 | 0.58/0.51 | 0.55         |
| Gate: 2 prev + eMFD@0.10   | 0.10/0.10 | 0.59/0.52 | 0.55         |
| Lex - MFD-20               | 0.50/0.50 | 0.59/0.52 | 0.55         |
| Gate: Baseline@0.50        | 0.10/0.10 | 0.59/0.53 | <b>0.56</b>  |
| Lex - MFD-20               | 0.50/0.50 | 0.59/0.52 | <b>0.56</b>  |
| Gate: LIWC22+LingFeat@0.50 | 0.10/0.10 | 0.59/0.53 | <b>0.56</b>  |
| Lex - MFD-20               | 0.50/0.50 | 0.58/0.52 | 0.55         |
| Gate: LIWC22+LingFeat@0.10 | 0.10/0.57 | 0.58/0.51 | 0.55         |
| Lex - MFD-20               | 0.50/0.50 | 0.58/0.52 | 0.55         |
| Gate: 2 prev + EmoLex@0.10 | 0.10/0.10 | 0.58/0.53 | 0.55         |
| Lex - MFD-20               | 0.50/0.50 | 0.59/0.52 | 0.55         |
| Gate: 2 prev + LIWC22@0.10 | 0.10/0.10 | 0.58/0.53 | <b>0.56</b>  |
| Lex - MFD-20               | 0.50/0.50 | 0.59/0.52 | 0.55         |
| Gate: 2 prev + eMFD@0.10   | 0.10/0.10 | 0.58/0.52 | 0.55         |
| TD - LDA                   | 0.50/0.50 | 0.59/0.50 | 0.55         |
| Gate: Baseline@0.50        | 0.10/0.12 | 0.58/0.52 | 0.55         |
| TD - LDA                   | 0.50/0.50 | 0.59/0.51 | 0.55         |
| Gate: LIWC22+LingFeat@0.50 | 0.10/0.11 | 0.58/0.52 | 0.55         |
| TD - LDA                   | 0.50/0.50 | 0.58/0.51 | 0.55         |
| Gate: LIWC22+LingFeat@0.10 | 0.10/0.38 | 0.55/0.52 | 0.54         |
| TD - LDA                   | 0.50/0.50 | 0.59/0.51 | 0.55         |
| Gate: 2 prev + EmoLex@0.10 | 0.10/0.21 | 0.56/0.52 | 0.54         |
| TD - LDA                   | 0.50/0.50 | 0.59/0.51 | 0.55         |
| Gate: 2 prev + LIWC22@0.10 | 0.10/0.25 | 0.56/0.52 | 0.54         |
| TD - LDA                   | 0.50/0.50 | 0.59/0.50 | 0.55         |
| Gate: 2 prev + eMFD@0.10   | 0.10/0.19 | 0.57/0.52 | 0.54         |

Table S28: Test F1-scores for Social Focus vs. Personal Focus detection with a Presence gate (Part 6/8). Thr and F1 are reported as Social/Personal pairs; Macro- $F_1$  is the macro-average over the two classes. Best Macro- $F_1$  values are bolded.

| Configuration              | Thr (S/P) | F1 (S/P)  | Macro- $F_1$ |
|----------------------------|-----------|-----------|--------------|
| TD - NMF                   | 0.50/0.50 | 0.59/0.50 | 0.55         |
| Gate: Baseline@0.50        | 0.10/0.13 | 0.57/0.52 | 0.55         |
| TD - NMF                   | 0.50/0.50 | 0.59/0.50 | 0.55         |
| Gate: LIWC22+LingFeat@0.50 | 0.10/0.12 | 0.57/0.52 | 0.55         |
| TD - NMF                   | 0.50/0.50 | 0.58/0.51 | 0.54         |
| Gate: LIWC22+LingFeat@0.10 | 0.10/0.39 | 0.55/0.52 | 0.53         |
| TD - NMF                   | 0.50/0.50 | 0.59/0.50 | 0.54         |
| Gate: 2 prev + EmoLex@0.10 | 0.10/0.24 | 0.56/0.53 | 0.54         |
| TD - NMF                   | 0.50/0.50 | 0.59/0.51 | 0.55         |
| Gate: 2 prev + LIWC22@0.10 | 0.10/0.27 | 0.56/0.52 | 0.54         |
| TD - NMF                   | 0.50/0.50 | 0.59/0.50 | 0.54         |
| Gate: 2 prev + eMFD@0.10   | 0.10/0.21 | 0.56/0.52 | 0.54         |
| TD - BERTopic              | 0.50/0.50 | 0.59/0.49 | 0.54         |
| Gate: Baseline@0.50        | 0.10/0.14 | 0.57/0.52 | 0.55         |
| TD - BERTopic              | 0.50/0.50 | 0.60/0.49 | 0.55         |
| Gate: LIWC22+LingFeat@0.50 | 0.10/0.13 | 0.58/0.53 | 0.55         |
| TD - BERTopic              | 0.50/0.50 | 0.58/0.50 | 0.54         |
| Gate: LIWC22+LingFeat@0.10 | 0.10/0.40 | 0.55/0.51 | 0.53         |
| TD - BERTopic              | 0.50/0.50 | 0.59/0.50 | 0.54         |
| Gate: 2 prev + EmoLex@0.10 | 0.10/0.24 | 0.56/0.52 | 0.54         |
| TD - BERTopic              | 0.50/0.50 | 0.59/0.50 | 0.55         |
| Gate: 2 prev + LIWC22@0.10 | 0.10/0.28 | 0.56/0.50 | 0.54         |
| TD - BERTopic              | 0.50/0.50 | 0.59/0.49 | 0.54         |
| Gate: 2 prev + eMFD@0.10   | 0.10/0.22 | 0.56/0.52 | 0.54         |
| Lex - LIWC 22 + Ling Feat  | 0.50/0.50 | 0.59/0.50 | 0.55         |
| Gate: Baseline@0.50        | 0.10/0.10 | 0.59/0.52 | 0.55         |
| Lex - LIWC 22 + Ling Feat  | 0.50/0.50 | 0.59/0.51 | 0.55         |
| Gate: LIWC22+LingFeat@0.50 | 0.10/0.10 | 0.59/0.52 | <b>0.56</b>  |
| Lex - LIWC 22 + Ling Feat  | 0.50/0.50 | 0.58/0.51 | 0.54         |
| Gate: LIWC22+LingFeat@0.10 | 0.10/0.59 | 0.58/0.51 | 0.54         |
| Lex - LIWC 22 + Ling Feat  | 0.50/0.50 | 0.58/0.51 | 0.55         |
| Gate: 2 prev + EmoLex@0.10 | 0.10/0.10 | 0.58/0.52 | 0.55         |
| Lex - LIWC 22 + Ling Feat  | 0.50/0.50 | 0.58/0.51 | 0.55         |
| Gate: 2 prev + LIWC22@0.10 | 0.10/0.11 | 0.58/0.52 | 0.55         |
| Lex - LIWC 22 + Ling Feat  | 0.50/0.50 | 0.58/0.51 | 0.55         |
| Gate: 2 prev + eMFD@0.10   | 0.10/0.10 | 0.59/0.52 | 0.55         |

Table S29: Test F1-scores for Social Focus vs. Personal Focus detection with a Presence gate (Part 7/8). Thr and F1 are reported as Social/Personal pairs; Macro- $F_1$  is the macro-average over the two classes. Best Macro- $F_1$  values are bolded.

| Configuration              | Thr (S/P) | F1 (S/P)  | Macro- $F_1$ |
|----------------------------|-----------|-----------|--------------|
| Lex - MFD-20               | 0.50/0.50 | 0.59/0.52 | 0.55         |
| Gate: Baseline@0.50        | 0.10/0.10 | 0.59/0.53 | <b>0.56</b>  |
| Lex - MFD-20               | 0.50/0.50 | 0.59/0.52 | <b>0.56</b>  |
| Gate: LIWC22+LingFeat@0.50 | 0.10/0.10 | 0.59/0.53 | <b>0.56</b>  |
| Lex - MFD-20               | 0.50/0.50 | 0.58/0.52 | 0.55         |
| Gate: LIWC22+LingFeat@0.10 | 0.10/0.57 | 0.58/0.51 | 0.55         |
| Lex - MFD-20               | 0.50/0.50 | 0.58/0.52 | 0.55         |
| Gate: 2 prev + EmoLex@0.10 | 0.10/0.10 | 0.58/0.53 | 0.55         |
| Lex - MFD-20               | 0.50/0.50 | 0.59/0.52 | 0.55         |
| Gate: 2 prev + LIWC22@0.10 | 0.10/0.10 | 0.58/0.53 | <b>0.56</b>  |
| Lex - MFD-20               | 0.50/0.50 | 0.59/0.52 | 0.55         |
| Gate: 2 prev + eMFD@0.10   | 0.10/0.10 | 0.58/0.52 | 0.55         |
| TD - LDA                   | 0.50/0.50 | 0.59/0.50 | 0.55         |
| Gate: Baseline@0.50        | 0.10/0.12 | 0.58/0.52 | 0.55         |
| TD - LDA                   | 0.50/0.50 | 0.59/0.51 | 0.55         |
| Gate: LIWC22+LingFeat@0.50 | 0.10/0.11 | 0.58/0.52 | 0.55         |
| TD - LDA                   | 0.50/0.50 | 0.58/0.51 | 0.55         |
| Gate: LIWC22+LingFeat@0.10 | 0.10/0.38 | 0.55/0.52 | 0.54         |
| TD - LDA                   | 0.50/0.50 | 0.59/0.51 | 0.55         |
| Gate: 2 prev + EmoLex@0.10 | 0.10/0.21 | 0.56/0.52 | 0.54         |
| TD - LDA                   | 0.50/0.50 | 0.59/0.51 | 0.55         |
| Gate: 2 prev + LIWC22@0.10 | 0.10/0.25 | 0.56/0.52 | 0.54         |
| TD - LDA                   | 0.50/0.50 | 0.59/0.50 | 0.55         |
| Gate: 2 prev + eMFD@0.10   | 0.10/0.19 | 0.57/0.52 | 0.54         |
| TD - NMF                   | 0.50/0.50 | 0.59/0.50 | 0.55         |
| Gate: Baseline@0.50        | 0.10/0.13 | 0.57/0.52 | 0.55         |
| TD - NMF                   | 0.50/0.50 | 0.59/0.50 | 0.55         |
| Gate: LIWC22+LingFeat@0.50 | 0.10/0.12 | 0.57/0.52 | 0.55         |
| TD - NMF                   | 0.50/0.50 | 0.58/0.51 | 0.54         |
| Gate: LIWC22+LingFeat@0.10 | 0.10/0.39 | 0.55/0.52 | 0.53         |
| TD - NMF                   | 0.50/0.50 | 0.59/0.50 | 0.54         |
| Gate: 2 prev + EmoLex@0.10 | 0.10/0.24 | 0.56/0.53 | 0.54         |
| TD - NMF                   | 0.50/0.50 | 0.59/0.51 | 0.55         |
| Gate: 2 prev + LIWC22@0.10 | 0.10/0.27 | 0.56/0.52 | 0.54         |
| TD - NMF                   | 0.50/0.50 | 0.59/0.50 | 0.54         |
| Gate: 2 prev + eMFD@0.10   | 0.10/0.21 | 0.56/0.52 | 0.54         |

Table S30: Test F1-scores for Social Focus vs. Personal Focus detection with a Presence gate (Part 8/8). Thr and F1 are reported as Social/Personal pairs; Macro- $F_1$  is the macro-average over the two classes. Best Macro- $F_1$  values are bolded.

| Configuration              | Thr (S/P) | F1 (S/P)  | Macro- $F_1$ |
|----------------------------|-----------|-----------|--------------|
| TD - BERTopic              | 0.50/0.50 | 0.59/0.49 | 0.54         |
| Gate: Baseline@0.50        | 0.10/0.14 | 0.57/0.52 | 0.55         |
| TD - BERTopic              | 0.50/0.50 | 0.60/0.49 | 0.55         |
| Gate: LIWC22+LingFeat@0.50 | 0.10/0.13 | 0.58/0.53 | 0.55         |
| TD - BERTopic              | 0.50/0.50 | 0.58/0.50 | 0.54         |
| Gate: LIWC22+LingFeat@0.10 | 0.10/0.40 | 0.55/0.51 | 0.53         |
| TD - BERTopic              | 0.50/0.50 | 0.59/0.50 | 0.54         |
| Gate: 2 prev + EmoLex@0.10 | 0.10/0.24 | 0.56/0.52 | 0.54         |
| TD - BERTopic              | 0.50/0.50 | 0.59/0.50 | 0.55         |
| Gate: 2 prev + LIWC22@0.10 | 0.10/0.28 | 0.56/0.50 | 0.54         |
| TD - BERTopic              | 0.50/0.50 | 0.59/0.49 | 0.54         |
| Gate: 2 prev + eMFD@0.10   | 0.10/0.22 | 0.56/0.52 | 0.54         |

#### S4. Moral value detection with Higher-Order category gates

This appendix reports moral value detection results when higher-order category detectors are used as gates. For each higher-order category, the best model is selected on the validation set, and moral value detectors are then evaluated on the test set only for the moral values belonging to that higher-order category; for transparency, we report validation F1-scores per moral value (and macro-average) for all evaluated variants, and test macro-average F1 for the explored gate/threshold configurations.

##### *S4.1. Growth gate*

##### *S4.2. Self-Protection gate*

Table S31: Validation F1-scores for moral value detection under the Growth gate. Macro- $F_1$  is the macro-average over the 11 moral values.

| Model                     | SD-t | SD-a | Stim | Hed  | Ach  | Hum  | Ben-c | Ben-d | Uni-c | Uni-n | Uni-t | Macro- $F_1$ |
|---------------------------|------|------|------|------|------|------|-------|-------|-------|-------|-------|--------------|
| Baseline                  | 0.27 | 0.47 | 0.44 | 0.46 | 0.65 | 0.21 | 0.38  | 0.42  | 0.54  | 0.78  | 0.39  | <b>0.46</b>  |
| Token Pruning             | 0.25 | 0.49 | 0.43 | 0.47 | 0.64 | 0.11 | 0.35  | 0.40  | 0.46  | 0.79  | 0.43  | 0.44         |
| 2 prev sent w/ label      | 0.27 | 0.47 | 0.44 | 0.46 | 0.65 | 0.21 | 0.38  | 0.42  | 0.54  | 0.78  | 0.39  | <b>0.46</b>  |
| MultiLayer                | 0.20 | 0.48 | 0.45 | 0.50 | 0.62 | 0.00 | 0.38  | 0.40  | 0.51  | 0.77  | 0.37  | 0.43         |
| Residual Block            | 0.24 | 0.46 | 0.42 | 0.49 | 0.65 | 0.09 | 0.38  | 0.40  | 0.52  | 0.78  | 0.38  | 0.44         |
| Data Augmentation         | 0.18 | 0.31 | 0.33 | 0.35 | 0.55 | 0.12 | 0.29  | 0.26  | 0.40  | 0.65  | 0.23  | 0.33         |
| Custom Stopwords          | 0.22 | 0.49 | 0.42 | 0.45 | 0.65 | 0.12 | 0.36  | 0.42  | 0.50  | 0.79  | 0.37  | 0.44         |
| NER                       | 0.24 | 0.50 | 0.41 | 0.47 | 0.65 | 0.04 | 0.42  | 0.45  | 0.53  | 0.78  | 0.36  | 0.44         |
| Lex - Schwartz            | 0.24 | 0.47 | 0.46 | 0.44 | 0.64 | 0.08 | 0.41  | 0.40  | 0.51  | 0.79  | 0.37  | 0.44         |
| Lex - VAD                 | 0.24 | 0.48 | 0.40 | 0.48 | 0.64 | 0.00 | 0.43  | 0.41  | 0.55  | 0.79  | 0.37  | 0.44         |
| Lex - EmoLex              | 0.25 | 0.49 | 0.40 | 0.43 | 0.65 | 0.15 | 0.37  | 0.42  | 0.53  | 0.79  | 0.38  | 0.44         |
| Lex - Emotion Intensity   | 0.24 | 0.49 | 0.39 | 0.49 | 0.64 | 0.16 | 0.40  | 0.40  | 0.53  | 0.78  | 0.37  | 0.44         |
| Lex - WorryWords          | 0.25 | 0.48 | 0.40 | 0.50 | 0.66 | 0.11 | 0.38  | 0.39  | 0.53  | 0.79  | 0.37  | 0.44         |
| Lex - LIWC 15             | 0.22 | 0.47 | 0.43 | 0.45 | 0.65 | 0.08 | 0.37  | 0.42  | 0.53  | 0.79  | 0.40  | 0.44         |
| Lex - MFD                 | 0.26 | 0.48 | 0.45 | 0.44 | 0.64 | 0.08 | 0.39  | 0.40  | 0.51  | 0.79  | 0.37  | 0.44         |
| Lex - LIWC 22             | 0.27 | 0.47 | 0.44 | 0.46 | 0.65 | 0.19 | 0.38  | 0.41  | 0.52  | 0.78  | 0.33  | 0.45         |
| Lex - LIWC 22 + Ling Feat | 0.27 | 0.47 | 0.44 | 0.46 | 0.65 | 0.19 | 0.38  | 0.41  | 0.52  | 0.78  | 0.33  | 0.45         |
| Lex - MFD-20              | 0.20 | 0.48 | 0.40 | 0.49 | 0.66 | 0.11 | 0.40  | 0.40  | 0.53  | 0.79  | 0.36  | 0.44         |
| Lex - eMFD                | 0.22 | 0.47 | 0.42 | 0.48 | 0.65 | 0.11 | 0.39  | 0.40  | 0.54  | 0.79  | 0.37  | 0.44         |
| Lex - MJD                 | 0.22 | 0.50 | 0.38 | 0.48 | 0.64 | 0.08 | 0.42  | 0.41  | 0.54  | 0.78  | 0.37  | 0.44         |
| TD - LDA                  | 0.21 | 0.50 | 0.40 | 0.52 | 0.65 | 0.12 | 0.42  | 0.42  | 0.51  | 0.76  | 0.36  | 0.44         |
| TD - NMF                  | 0.25 | 0.48 | 0.45 | 0.47 | 0.65 | 0.20 | 0.37  | 0.38  | 0.49  | 0.78  | 0.38  | 0.45         |
| TD - BERTopic             | 0.20 | 0.50 | 0.39 | 0.51 | 0.65 | 0.12 | 0.41  | 0.43  | 0.50  | 0.75  | 0.36  | 0.44         |

Table S32: Test macro-average F1 for moral value detection under the Growth gate for the explored detector threshold and gate configuration pairs. Values are reported with 4 decimals to avoid artificial ties.

| <b>Configuration</b>                                  | <b>Macro-<math>F_1</math></b> |
|-------------------------------------------------------|-------------------------------|
| Model: Baseline@0.50. Gate: Baseline@0.50             | 0.2629                        |
| Model: Baseline@0.50. Gate: Baseline@0.18             | 0.2693                        |
| Model: 2 prev sent w/ label@0.50. Gate: Baseline@0.50 | 0.2650                        |
| Model: 2 prev sent w/ label@0.50. Gate: Baseline@0.18 | 0.2643                        |
| Model: Baseline@0.30. Gate: Baseline@0.50             | <b>0.2707</b>                 |
| Model: Baseline@0.60. Gate: Baseline@0.18             | 0.2691                        |
| Model: 2 prev sent w/ label@0.45. Gate: Baseline@0.50 | 0.2658                        |
| Model: 2 prev sent w/ label@0.40. Gate: Baseline@0.18 | 0.2622                        |



Table S33: Validation F1-scores for moral value detection under the Self-Protection gate. Macro- $F_1$  is the macro-average over the 10 moral values.

| Model                   | Ach  | Pow-d | Pow-r | Face | Sec-per | Sec-soc | Trad | Confr | Confr-onter | Hum  | Macro- $F_1$ |
|-------------------------|------|-------|-------|------|---------|---------|------|-------|-------------|------|--------------|
| Baseline                | 0.59 | 0.48  | 0.57  | 0.40 | 0.53    | 0.61    | 0.64 | 0.65  | 0.25        | 0.04 | <b>0.48</b>  |
| Token Pruning           | 0.58 | 0.48  | 0.56  | 0.34 | 0.56    | 0.63    | 0.65 | 0.65  | 0.14        | 0.00 | 0.46         |
| 2 prev sent w/ label    | 0.60 | 0.52  | 0.52  | 0.38 | 0.55    | 0.61    | 0.63 | 0.65  | 0.27        | 0.04 | 0.48         |
| MultiLayer              | 0.57 | 0.49  | 0.54  | 0.37 | 0.52    | 0.62    | 0.59 | 0.67  | 0.20        | 0.00 | 0.46         |
| Residual Block          | 0.61 | 0.48  | 0.57  | 0.39 | 0.50    | 0.61    | 0.65 | 0.66  | 0.27        | 0.04 | 0.48         |
| Data Augmentation       | 0.41 | 0.40  | 0.37  | 0.30 | 0.42    | 0.52    | 0.46 | 0.51  | 0.08        | 0.00 | 0.35         |
| Custom Stopwords        | 0.60 | 0.47  | 0.53  | 0.38 | 0.54    | 0.60    | 0.61 | 0.66  | 0.23        | 0.14 | 0.48         |
| NER                     | 0.60 | 0.51  | 0.53  | 0.39 | 0.56    | 0.61    | 0.63 | 0.66  | 0.24        | 0.08 | 0.48         |
| Lex - Schwartz          | 0.58 | 0.49  | 0.56  | 0.37 | 0.54    | 0.61    | 0.66 | 0.65  | 0.22        | 0.08 | 0.48         |
| Lex - VAD               | 0.60 | 0.48  | 0.57  | 0.40 | 0.53    | 0.62    | 0.62 | 0.64  | 0.26        | 0.10 | 0.48         |
| Lex - EmoLex            | 0.59 | 0.49  | 0.54  | 0.37 | 0.55    | 0.61    | 0.65 | 0.64  | 0.24        | 0.12 | 0.48         |
| Lex - Emotion Intensity | 0.60 | 0.51  | 0.51  | 0.41 | 0.55    | 0.60    | 0.64 | 0.68  | 0.26        | 0.04 | 0.48         |
| Lex - WorryWords        | 0.60 | 0.48  | 0.59  | 0.40 | 0.57    | 0.63    | 0.64 | 0.63  | 0.12        | 0.00 | 0.47         |
| Lex - LIWC 15           | 0.60 | 0.50  | 0.53  | 0.36 | 0.53    | 0.61    | 0.63 | 0.64  | 0.27        | 0.10 | 0.48         |
| Lex - MFD               | 0.58 | 0.49  | 0.56  | 0.38 | 0.55    | 0.61    | 0.66 | 0.64  | 0.21        | 0.08 | 0.48         |
| Lex - LIWC 22           | 0.58 | 0.50  | 0.56  | 0.39 | 0.55    | 0.60    | 0.59 | 0.65  | 0.23        | 0.14 | 0.48         |
| Lex - LIWC 22 + Ling    | 0.58 | 0.50  | 0.56  | 0.39 | 0.55    | 0.60    | 0.59 | 0.65  | 0.23        | 0.14 | 0.48         |
| Feat                    |      |       |       |      |         |         |      |       |             |      |              |
| Lex - MFD-20            | 0.61 | 0.51  | 0.51  | 0.38 | 0.56    | 0.59    | 0.64 | 0.67  | 0.24        | 0.04 | 0.48         |
| Lex - eMFD              | 0.60 | 0.49  | 0.56  | 0.39 | 0.50    | 0.63    | 0.64 | 0.66  | 0.25        | 0.04 | 0.48         |
| Lex - MJD               | 0.59 | 0.50  | 0.52  | 0.40 | 0.56    | 0.60    | 0.65 | 0.67  | 0.23        | 0.04 | 0.48         |
| TD - LDA                | 0.59 | 0.47  | 0.56  | 0.41 | 0.54    | 0.61    | 0.62 | 0.64  | 0.23        | 0.07 | 0.47         |
| TD - NMF                | 0.59 | 0.48  | 0.57  | 0.38 | 0.51    | 0.63    | 0.64 | 0.66  | 0.25        | 0.04 | 0.48         |
| TD - BERTopic           | 0.57 | 0.48  | 0.53  | 0.39 | 0.53    | 0.61    | 0.65 | 0.65  | 0.27        | 0.07 | 0.48         |

Table S34: Test macro-average F1 for moral value detection under the Self-Protection gate for the explored detector threshold and gate configuration pairs. Values are reported with 4 decimals to avoid artificial ties.

| <b>Configuration</b>                      | <b>Macro-<math>F_1</math></b> |
|-------------------------------------------|-------------------------------|
| Model: Baseline@0.50. Gate: Baseline@0.50 | 0.2935                        |
| Model: Baseline@0.50. Gate: Baseline@0.10 | 0.2988                        |
| Model: Baseline@0.15. Gate: Baseline@0.50 | <b>0.3062</b>                 |
| Model: Baseline@0.60. Gate: Baseline@0.10 | 0.2983                        |

Table S35: Validation F1-scores for moral values detection with a Social Focus gate (macro-average over all moral values).

| Model                           | Sec-soc | Trad | Confr | Confi | Hum  | Benc-c | Ben-d | Uni-c | Uni-n | Unit | Macro- $F_1$ |
|---------------------------------|---------|------|-------|-------|------|--------|-------|-------|-------|------|--------------|
| <b>Baseline</b>                 | 0.70    | 0.66 | 0.72  | 0.34  | 0.18 | 0.41   | 0.42  | 0.48  | 0.81  | 0.38 | <b>0.51</b>  |
| Token Pruning                   | 0.69    | 0.62 | 0.69  | 0.33  | 0.15 | 0.36   | 0.40  | 0.46  | 0.79  | 0.37 | 0.49         |
| 2 prev sent w/ label            | 0.69    | 0.65 | 0.69  | 0.34  | 0.13 | 0.37   | 0.40  | 0.50  | 0.80  | 0.33 | 0.49         |
| MultiLayer                      | 0.70    | 0.62 | 0.71  | 0.32  | 0.00 | 0.40   | 0.41  | 0.45  | 0.75  | 0.35 | 0.47         |
| Residual Block                  | 0.71    | 0.64 | 0.71  | 0.33  | 0.12 | 0.37   | 0.38  | 0.47  | 0.81  | 0.39 | 0.49         |
| Data Augmentation               | 0.60    | 0.49 | 0.56  | 0.13  | 0.00 | 0.32   | 0.31  | 0.40  | 0.62  | 0.33 | 0.38         |
| Custom Stopwords                | 0.69    | 0.64 | 0.71  | 0.32  | 0.13 | 0.28   | 0.40  | 0.51  | 0.80  | 0.32 | 0.48         |
| NER                             | 0.69    | 0.63 | 0.71  | 0.30  | 0.21 | 0.40   | 0.41  | 0.47  | 0.80  | 0.35 | 0.50         |
| Lex - Schwartz                  | 0.68    | 0.63 | 0.70  | 0.33  | 0.13 | 0.39   | 0.40  | 0.50  | 0.81  | 0.31 | 0.49         |
| Lex - VAD                       | 0.70    | 0.65 | 0.70  | 0.33  | 0.12 | 0.37   | 0.41  | 0.49  | 0.81  | 0.29 | 0.49         |
| Lex - EmoLex                    | 0.68    | 0.62 | 0.70  | 0.33  | 0.13 | 0.38   | 0.41  | 0.50  | 0.80  | 0.32 | 0.49         |
| Lex - Emotion Intensity         | 0.69    | 0.62 | 0.72  | 0.36  | 0.13 | 0.30   | 0.41  | 0.50  | 0.80  | 0.34 | 0.49         |
| Lex - WorryWords                | 0.68    | 0.65 | 0.71  | 0.33  | 0.13 | 0.40   | 0.35  | 0.48  | 0.81  | 0.36 | 0.49         |
| Lex - LIWC 15                   | 0.69    | 0.65 | 0.70  | 0.32  | 0.17 | 0.36   | 0.36  | 0.50  | 0.81  | 0.30 | 0.49         |
| Lex - MFD                       | 0.68    | 0.63 | 0.70  | 0.32  | 0.13 | 0.39   | 0.41  | 0.50  | 0.81  | 0.33 | 0.49         |
| Lex - LIWC 22                   | 0.70    | 0.65 | 0.70  | 0.35  | 0.17 | 0.38   | 0.41  | 0.52  | 0.81  | 0.27 | 0.50         |
| Lex - LIWC 22 + Ling Feat       | 0.69    | 0.64 | 0.70  | 0.33  | 0.17 | 0.39   | 0.42  | 0.48  | 0.80  | 0.34 | 0.50         |
| Lex - MFD-20                    | 0.69    | 0.66 | 0.71  | 0.35  | 0.18 | 0.34   | 0.43  | 0.47  | 0.80  | 0.33 | 0.50         |
| Lex - eMFD                      | 0.69    | 0.65 | 0.70  | 0.38  | 0.20 | 0.32   | 0.41  | 0.49  | 0.80  | 0.36 | 0.50         |
| Lex - MJD                       | 0.70    | 0.66 | 0.69  | 0.31  | 0.16 | 0.43   | 0.40  | 0.49  | 0.81  | 0.31 | 0.50         |
| TD - LDA                        | 0.70    | 0.64 | 0.70  | 0.33  | 0.17 | 0.39   | 0.40  | 0.48  | 0.81  | 0.35 | 0.50         |
| TD - NMF                        | 0.70    | 0.65 | 0.71  | 0.33  | 0.09 | 0.39   | 0.40  | 0.48  | 0.81  | 0.36 | 0.49         |
| TD - BERTopic                   | 0.71    | 0.64 | 0.70  | 0.35  | 0.09 | 0.40   | 0.38  | 0.48  | 0.81  | 0.32 | 0.49         |
| NER + Lex - Schwartz            | 0.70    | 0.65 | 0.71  | 0.33  | 0.23 | 0.37   | 0.41  | 0.48  | 0.79  | 0.36 | 0.50         |
| NER + Lex - VAD                 | 0.70    | 0.66 | 0.72  | 0.37  | 0.14 | 0.37   | 0.41  | 0.45  | 0.81  | 0.34 | 0.50         |
| NER + Lex - EmoLex              | 0.70    | 0.66 | 0.71  | 0.34  | 0.12 | 0.36   | 0.43  | 0.47  | 0.79  | 0.37 | 0.50         |
| NER + Lex - MFD                 | 0.69    | 0.66 | 0.70  | 0.33  | 0.09 | 0.39   | 0.41  | 0.46  | 0.81  | 0.35 | 0.49         |
| NER + Lex - LIWC 22             | 0.70    | 0.62 | 0.72  | 0.29  | 0.15 | 0.40   | 0.43  | 0.47  | 0.81  | 0.36 | 0.50         |
| NER + Lex - LIWC 22 + Ling Feat | 0.70    | 0.62 | 0.72  | 0.29  | 0.15 | 0.40   | 0.43  | 0.47  | 0.81  | 0.36 | 0.50         |
| NER + Lex - MFD-20              | 0.70    | 0.64 | 0.72  | 0.32  | 0.21 | 0.36   | 0.42  | 0.49  | 0.79  | 0.35 | 0.50         |
| NER + Lex - eMFD                | 0.70    | 0.64 | 0.71  | 0.31  | 0.21 | 0.37   | 0.40  | 0.48  | 0.80  | 0.34 | 0.50         |
| NER + Lex - MJD                 | 0.70    | 0.65 | 0.72  | 0.32  | 0.13 | 0.39   | 0.41  | 0.49  | 0.82  | 0.36 | 0.50         |
| NER + Lex - TD - LDA            | 0.70    | 0.64 | 0.72  | 0.35  | 0.12 | 0.38   | 0.41  | 0.47  | 0.80  | 0.37 | 0.50         |

Table S36: Test Macro- $F_1$  for moral values detection with a Social Focus gate (Part 1/3). Best Macro- $F_1$  is bolded (ties included). Values are reported with 4 decimals to avoid artificial ties.

| Configuration                                               | Macro- $F_1$ |
|-------------------------------------------------------------|--------------|
| Model: Baseline@0.50. Gate: TD - NMF@0.50                   | 0.3090       |
| Model: Baseline@0.50. Gate: 2 prev sent w/ label@0.10       | 0.3082       |
| Model: Baseline@0.50. Gate: NER@0.10                        | 0.3093       |
| Model: Baseline@0.50. Gate: Lex - WorryWords@0.10           | 0.3098       |
| Model: Baseline@0.50. Gate: Lex - LIWC 15@0.10              | 0.3063       |
| Model: Baseline@0.25. Gate: TD - NMF@0.50                   | 0.3183       |
| Model: Baseline@0.55. Gate: 2 prev sent w/ label@0.10       | 0.3063       |
| Model: Baseline@0.55. Gate: NER@0.10                        | 0.3080       |
| Model: Baseline@0.55. Gate: Lex - WorryWords@0.10           | 0.3087       |
| Model: Baseline@0.55. Gate: Lex - LIWC 15@0.10              | 0.3050       |
| Model: NER@0.50. Gate: TD - NMF@0.50                        | 0.3042       |
| Model: NER@0.50. Gate: 2 prev sent w/ label@0.10            | 0.3071       |
| Model: NER@0.50. Gate: NER@0.10                             | 0.3077       |
| Model: NER@0.50. Gate: Lex - WorryWords@0.10                | 0.3106       |
| Model: NER@0.50. Gate: Lex - LIWC 15@0.10                   | 0.3057       |
| Model: NER@0.20. Gate: TD - NMF@0.50                        | 0.3194       |
| Model: NER@0.45. Gate: 2 prev sent w/ label@0.10            | 0.3057       |
| Model: NER@0.45. Gate: NER@0.10                             | 0.3075       |
| Model: NER@0.45. Gate: Lex - WorryWords@0.10                | 0.3100       |
| Model: NER@0.45. Gate: Lex - LIWC 15@0.10                   | 0.3054       |
| Model: Lex - Schwartz@0.50. Gate: TD - NMF@0.50             | 0.2976       |
| Model: Lex - Schwartz@0.50. Gate: 2 prev sent w/ label@0.10 | 0.3064       |
| Model: Lex - Schwartz@0.50. Gate: NER@0.10                  | 0.3067       |
| Model: Lex - Schwartz@0.50. Gate: Lex - WorryWords@0.10     | 0.3090       |
| Model: Lex - Schwartz@0.50. Gate: Lex - LIWC 15@0.10        | 0.3037       |
| Model: Lex - Schwartz@0.30. Gate: TD - NMF@0.50             | 0.3091       |
| Model: Lex - Schwartz@0.50. Gate: 2 prev sent w/ label@0.10 | 0.3064       |
| Model: Lex - Schwartz@0.50. Gate: NER@0.10                  | 0.3067       |
| Model: Lex - Schwartz@0.50. Gate: Lex - WorryWords@0.10     | 0.3090       |
| Model: Lex - Schwartz@0.50. Gate: Lex - LIWC 15@0.10        | 0.3037       |
| Model: Lex - VAD@0.50. Gate: TD - NMF@0.50                  | 0.2996       |
| Model: Lex - VAD@0.50. Gate: 2 prev sent w/ label@0.10      | 0.3074       |
| Model: Lex - VAD@0.50. Gate: NER@0.10                       | 0.3064       |
| Model: Lex - VAD@0.50. Gate: Lex - WorryWords@0.10          | 0.3080       |
| Model: Lex - VAD@0.50. Gate: Lex - LIWC 15@0.10             | 0.3050       |
| Model: Lex - VAD@0.20. Gate: TD - NMF@0.50                  | 0.3253       |
| Model: Lex - VAD@0.45. Gate: 2 prev sent w/ label@0.10      | 0.3098       |
| Model: Lex - VAD@0.45. Gate: NER@0.10                       | 0.3086       |
| Model: Lex - VAD@0.45. Gate: Lex - WorryWords@0.10          | 0.3106       |
| Model: Lex - VAD@0.45. Gate: Lex - LIWC 15@0.10             | 0.3064       |

Table S37: Test Macro- $F_1$  for moral values detection with a Social Focus gate (Part 2/3). Best Macro- $F_1$  is bolded (ties included). Values are reported with 4 decimals to avoid artificial ties.

| Configuration                                                          | Macro- $F_1$ |
|------------------------------------------------------------------------|--------------|
| Model: Lex - EmoLex@0.50. Gate: TD - NMF@0.50                          | 0.2970       |
| Model: Lex - EmoLex@0.50. Gate: 2 prev sent w/ label@0.10              | 0.3046       |
| Model: Lex - EmoLex@0.50. Gate: NER@0.10                               | 0.3062       |
| Model: Lex - EmoLex@0.50. Gate: Lex - WorryWords@0.10                  | 0.3084       |
| Model: Lex - EmoLex@0.50. Gate: Lex - LIWC 15@0.10                     | 0.3031       |
| Model: Lex - EmoLex@0.30. Gate: TD - NMF@0.50                          | 0.3086       |
| Model: Lex - EmoLex@0.55. Gate: Lex - WorryWords@0.10                  | 0.3071       |
| Model: Lex - EmoLex@0.50. Gate: Lex - LIWC 15@0.10                     | 0.3031       |
| Model: Lex - MFD@0.50. Gate: TD - NMF@0.50                             | 0.2983       |
| Model: Lex - MFD@0.50. Gate: 2 prev sent w/ label@0.10                 | 0.3063       |
| Model: Lex - MFD@0.50. Gate: NER@0.10                                  | 0.3071       |
| Model: Lex - MFD@0.50. Gate: Lex - WorryWords@0.10                     | 0.3097       |
| Model: Lex - MFD@0.50. Gate: Lex - LIWC 15@0.10                        | 0.3041       |
| Model: Lex - MFD@0.30. Gate: TD - NMF@0.50                             | 0.3077       |
| Model: Lex - MFD@0.50. Gate: 2 prev sent w/ label@0.10                 | 0.3063       |
| Model: Lex - MFD@0.50. Gate: NER@0.10                                  | 0.3071       |
| Model: Lex - MFD@0.50. Gate: Lex - WorryWords@0.10                     | 0.3097       |
| Model: Lex - MFD@0.50. Gate: Lex - LIWC 15@0.10                        | 0.3041       |
| Model: Lex - LIWC 22@0.50. Gate: TD - NMF@0.50                         | 0.2926       |
| Model: Lex - LIWC 22@0.50. Gate: 2 prev sent w/ label@0.10             | 0.3022       |
| Model: Lex - LIWC 22@0.50. Gate: NER@0.10                              | 0.3032       |
| Model: Lex - LIWC 22@0.50. Gate: Lex - WorryWords@0.10                 | 0.3069       |
| Model: Lex - LIWC 22@0.50. Gate: Lex - LIWC 15@0.10                    | 0.3009       |
| Model: Lex - LIWC 22@0.30. Gate: TD - NMF@0.50                         | 0.3134       |
| Model: Lex - LIWC 22@0.60. Gate: 2 prev sent w/ label@0.10             | 0.2969       |
| Model: Lex - LIWC 22@0.45. Gate: NER@0.10                              | 0.3065       |
| Model: Lex - LIWC 22@0.60. Gate: Lex - WorryWords@0.10                 | 0.3007       |
| Model: Lex - LIWC 22@0.60. Gate: Lex - LIWC 15@0.10                    | 0.2961       |
| Model: Lex - LIWC 22 + Ling Feat@0.50. Gate: TD - NMF@0.50             | 0.3163       |
| Model: Lex - LIWC 22 + Ling Feat@0.50. Gate: 2 prev sent w/ label@0.10 | 0.3089       |
| Model: Lex - LIWC 22 + Ling Feat@0.50. Gate: NER@0.10                  | 0.3123       |
| Model: Lex - LIWC 22 + Ling Feat@0.50. Gate: Lex - WorryWords@0.10     | 0.3152       |
| Model: Lex - LIWC 22 + Ling Feat@0.50. Gate: Lex - LIWC 15@0.10        | 0.3117       |
| Model: Lex - LIWC 22 + Ling Feat@0.15. Gate: TD - NMF@0.50             | 0.3134       |
| Model: Lex - LIWC 22 + Ling Feat@0.55. Gate: 2 prev sent w/ label@0.10 | 0.3122       |
| Model: Lex - LIWC 22 + Ling Feat@0.55. Gate: NER@0.10                  | 0.3161       |
| Model: Lex - LIWC 22 + Ling Feat@0.55. Gate: Lex - WorryWords@0.10     | 0.3185       |
| Model: Lex - LIWC 22 + Ling Feat@0.55. Gate: Lex - LIWC 15@0.10        | 0.3148       |

Table S38: Test Macro- $F_1$  for moral values detection with a Social Focus gate (Part 3/3). Best Macro- $F_1$  is bolded (ties included). Values are reported with 4 decimals to avoid artificial ties.

| Configuration                                             | Macro- $F_1$  |
|-----------------------------------------------------------|---------------|
| Model: Lex - MFD-20@0.50. Gate: TD - NMF@0.50             | 0.2963        |
| Model: Lex - MFD-20@0.50. Gate: 2 prev sent w/ label@0.10 | 0.2945        |
| Model: Lex - MFD-20@0.50. Gate: NER@0.10                  | 0.2960        |
| Model: Lex - MFD-20@0.50. Gate: Lex - WorryWords@0.10     | 0.2988        |
| Model: Lex - MFD-20@0.50. Gate: Lex - LIWC 15@0.10        | 0.2948        |
| Model: Lex - MFD-20@0.20. Gate: TD - NMF@0.50             | 0.3086        |
| Model: Lex - MFD-20@0.40. Gate: 2 prev sent w/ label@0.10 | 0.2956        |
| Model: Lex - MFD-20@0.60. Gate: NER@0.10                  | 0.2974        |
| Model: Lex - MFD-20@0.60. Gate: Lex - WorryWords@0.10     | 0.3003        |
| Model: Lex - MFD-20@0.55. Gate: Lex - LIWC 15@0.10        | 0.2967        |
| Model: Lex - eMFD@0.50. Gate: TD - NMF@0.50               | 0.2952        |
| Model: Lex - eMFD@0.50. Gate: 2 prev sent w/ label@0.10   | 0.2953        |
| Model: Lex - eMFD@0.50. Gate: NER@0.10                    | 0.2975        |
| Model: Lex - eMFD@0.50. Gate: Lex - WorryWords@0.10       | 0.2997        |
| Model: Lex - eMFD@0.50. Gate: Lex - LIWC 15@0.10          | 0.2954        |
| Model: Lex - eMFD@0.25. Gate: TD - NMF@0.50               | 0.3058        |
| Model: Lex - eMFD@0.60. Gate: 2 prev sent w/ label@0.10   | 0.2978        |
| Model: Lex - eMFD@0.60. Gate: NER@0.10                    | 0.2999        |
| Model: Lex - eMFD@0.60. Gate: Lex - WorryWords@0.10       | 0.3023        |
| Model: Lex - eMFD@0.50. Gate: Lex - LIWC 15@0.10          | 0.2954        |
| Model: Lex - MJD@0.50. Gate: TD - NMF@0.50                | 0.3032        |
| Model: Lex - MJD@0.50. Gate: 2 prev sent w/ label@0.10    | 0.3105        |
| Model: Lex - MJD@0.50. Gate: NER@0.10                     | 0.3110        |
| Model: Lex - MJD@0.50. Gate: Lex - WorryWords@0.10        | 0.3138        |
| Model: Lex - MJD@0.50. Gate: Lex - LIWC 15@0.10           | 0.3099        |
| Model: Lex - MJD@0.25. Gate: TD - NMF@0.50                | <b>0.3256</b> |
| Model: Lex - MJD@0.40. Gate: 2 prev sent w/ label@0.10    | 0.3116        |
| Model: Lex - MJD@0.40. Gate: NER@0.10                     | 0.3118        |
| Model: Lex - MJD@0.45. Gate: Lex - WorryWords@0.10        | 0.3153        |
| Model: Lex - MJD@0.45. Gate: Lex - LIWC 15@0.10           | 0.3109        |
| Model: TD - LDA@0.50. Gate: TD - NMF@0.50                 | 0.3118        |
| Model: TD - LDA@0.50. Gate: 2 prev sent w/ label@0.10     | 0.3146        |
| Model: TD - LDA@0.50. Gate: NER@0.10                      | 0.3138        |
| Model: TD - LDA@0.50. Gate: Lex - WorryWords@0.10         | 0.3169        |
| Model: TD - LDA@0.50. Gate: Lex - LIWC 15@0.10            | 0.3124        |
| Model: TD - LDA@0.15. Gate: TD - NMF@0.50                 | 0.3251        |
| Model: TD - LDA@0.45. Gate: 2 prev sent w/ label@0.10     | 0.3162        |
| Model: TD - LDA@0.50. Gate: NER@0.10                      | 0.3138        |
| Model: TD - LDA@0.50. Gate: Lex - WorryWords@0.10         | 0.3169        |
| Model: TD - LDA@0.50. Gate: Lex - LIWC 15@0.10            | 0.3124        |

Table S39: Validation F1-scores for moral values detection with a Personal Focus gate (macro-average over all moral values). Best model (by Macro- $F_1$ ) is bolded.

| Model                            | SD-t | SD-a | Stim | Hed  | Ach  | Pow-d | Pow-r | Face | Sec-per | Macro- $F_1$ |
|----------------------------------|------|------|------|------|------|-------|-------|------|---------|--------------|
| Baseline                         | 0.24 | 0.42 | 0.47 | 0.50 | 0.60 | 0.62  | 0.66  | 0.46 | 0.60    | 0.51         |
| Token Pruning                    | 0.25 | 0.44 | 0.47 | 0.49 | 0.58 | 0.61  | 0.62  | 0.41 | 0.59    | 0.50         |
| 2 prev sent w/ label             | 0.28 | 0.43 | 0.45 | 0.48 | 0.60 | 0.64  | 0.63  | 0.44 | 0.62    | 0.51         |
| MultiLayer                       | 0.23 | 0.43 | 0.45 | 0.43 | 0.59 | 0.64  | 0.63  | 0.43 | 0.64    | 0.50         |
| Residual Block                   | 0.27 | 0.42 | 0.43 | 0.52 | 0.61 | 0.64  | 0.63  | 0.41 | 0.62    | 0.51         |
| Data Augmentation                | 0.22 | 0.31 | 0.34 | 0.37 | 0.52 | 0.50  | 0.50  | 0.34 | 0.54    | 0.40         |
| Custom Stopwords                 | 0.18 | 0.43 | 0.48 | 0.52 | 0.59 | 0.62  | 0.61  | 0.43 | 0.60    | 0.50         |
| NER                              | 0.25 | 0.42 | 0.45 | 0.48 | 0.59 | 0.64  | 0.64  | 0.39 | 0.60    | 0.50         |
| Lex - Schwartz                   | 0.29 | 0.42 | 0.46 | 0.49 | 0.60 | 0.62  | 0.60  | 0.48 | 0.62    | 0.51         |
| Lex - VAD                        | 0.24 | 0.43 | 0.46 | 0.52 | 0.61 | 0.63  | 0.63  | 0.42 | 0.62    | 0.51         |
| Lex - EmoLex                     | 0.29 | 0.43 | 0.45 | 0.49 | 0.59 | 0.63  | 0.62  | 0.48 | 0.61    | 0.51         |
| Lex - Emotion Intensity          | 0.31 | 0.43 | 0.45 | 0.49 | 0.60 | 0.60  | 0.61  | 0.49 | 0.61    | 0.51         |
| Lex - WorryWords                 | 0.23 | 0.43 | 0.41 | 0.47 | 0.57 | 0.63  | 0.66  | 0.47 | 0.60    | 0.50         |
| Lex - LIWC 15                    | 0.23 | 0.40 | 0.51 | 0.52 | 0.57 | 0.61  | 0.57  | 0.46 | 0.64    | 0.50         |
| Lex - MFD                        | 0.30 | 0.41 | 0.43 | 0.51 | 0.57 | 0.64  | 0.64  | 0.48 | 0.59    | 0.51         |
| Lex - LIWC 22                    | 0.31 | 0.43 | 0.48 | 0.48 | 0.58 | 0.61  | 0.60  | 0.46 | 0.62    | 0.51         |
| Lex - LIWC 22 + Ling Feat        | 0.31 | 0.43 | 0.48 | 0.48 | 0.58 | 0.61  | 0.60  | 0.46 | 0.62    | 0.51         |
| Lex - MFD-20                     | 0.28 | 0.43 | 0.43 | 0.50 | 0.58 | 0.64  | 0.64  | 0.44 | 0.61    | 0.51         |
| Lex - eMFD                       | 0.28 | 0.43 | 0.44 | 0.51 | 0.59 | 0.64  | 0.64  | 0.44 | 0.61    | 0.51         |
| <b>Lex - MJD</b>                 | 0.32 | 0.42 | 0.47 | 0.51 | 0.60 | 0.60  | 0.63  | 0.48 | 0.62    | <b>0.52</b>  |
| TD - LDA                         | 0.26 | 0.43 | 0.48 | 0.48 | 0.61 | 0.64  | 0.63  | 0.44 | 0.61    | 0.51         |
| TD - NMF                         | 0.27 | 0.45 | 0.47 | 0.50 | 0.60 | 0.64  | 0.63  | 0.45 | 0.61    | 0.51         |
| TD - BERTopic                    | 0.21 | 0.43 | 0.48 | 0.52 | 0.60 | 0.64  | 0.65  | 0.41 | 0.62    | 0.51         |
| 2 prev sent w/ label + Lex - MJD | 0.23 | 0.43 | 0.46 | 0.52 | 0.59 | 0.64  | 0.61  | 0.46 | 0.63    | 0.51         |

Table S40: Test Macro- $F_1$  for moral values detection with a Personal Focus gate. Configurations are reported as: Model (threshold) and Gate model (filter threshold). Best Macro- $F_1$  is bolded (ties included). Values are reported with 4 decimals to avoid artificial ties.

| Configuration                                      | Macro- $F_1$  |
|----------------------------------------------------|---------------|
| Model: Baseline@0.50. Gate: TD - NMF@0.50          | 0.2530        |
| Model: Baseline@0.50. Gate: NER@0.19               | 0.2842        |
| Model: Baseline@0.50. Gate: Lex - Schwartz@0.21    | 0.2824        |
| Model: Baseline@0.50. Gate: Lex - WorryWords@0.21  | 0.2792        |
| Model: Baseline@0.50. Gate: Lex - LIWC 15@0.17     | 0.2812        |
| Model: Baseline@0.50. Gate: TD - NMF@0.20          | 0.2818        |
| Model: Baseline@0.50. Gate: TD - BERTopic@0.22     | 0.2789        |
| Model: Baseline@0.45. Gate: TD - NMF@0.50          | 0.2607        |
| Model: Baseline@0.55. Gate: NER@0.19               | 0.2836        |
| Model: Baseline@0.55. Gate: Lex - Schwartz@0.21    | 0.2814        |
| Model: Baseline@0.55. Gate: Lex - WorryWords@0.21  | 0.2792        |
| Model: Baseline@0.55. Gate: Lex - LIWC 15@0.17     | 0.2805        |
| Model: Baseline@0.55. Gate: TD - NMF@0.20          | 0.2816        |
| Model: Baseline@0.55. Gate: TD - BERTopic@0.22     | 0.2785        |
| Model: Lex - MJD@0.50. Gate: TD - NMF@0.50         | 0.2605        |
| Model: Lex - MJD@0.50. Gate: NER@0.19              | 0.2830        |
| Model: Lex - MJD@0.50. Gate: Lex - Schwartz@0.21   | 0.2794        |
| Model: Lex - MJD@0.50. Gate: Lex - WorryWords@0.21 | 0.2784        |
| Model: Lex - MJD@0.50. Gate: Lex - LIWC 15@0.17    | 0.2810        |
| Model: Lex - MJD@0.50. Gate: TD - NMF@0.20         | 0.2826        |
| Model: Lex - MJD@0.50. Gate: TD - BERTopic@0.22    | 0.2798        |
| Model: Lex - MJD@0.35. Gate: TD - NMF@0.50         | 0.2606        |
| Model: Lex - MJD@0.70. Gate: NER@0.19              | <b>0.2868</b> |
| Model: Lex - MJD@0.70. Gate: Lex - Schwartz@0.21   | 0.2826        |
| Model: Lex - MJD@0.70. Gate: Lex - WorryWords@0.21 | 0.2815        |
| Model: Lex - MJD@0.70. Gate: Lex - LIWC 15@0.17    | 0.2827        |
| Model: Lex - MJD@0.70. Gate: TD - NMF@0.20         | 0.2847        |
| Model: Lex - MJD@0.70. Gate: TD - BERTopic@0.22    | 0.2840        |



Table S41: Validation F1-scores for moral values detection with an Openness gate (macro-average over the four moral values). Best model (by Macro- $F_1$ ) is bolded.

| Model                        | SD-t | SD-a | Stim | Hed  | Macro- $F_1$ |
|------------------------------|------|------|------|------|--------------|
| Baseline                     | 0.37 | 0.71 | 0.60 | 0.63 | 0.58         |
| Token Pruning                | 0.38 | 0.68 | 0.70 | 0.63 | 0.60         |
| 2 prev sent w/ label         | 0.35 | 0.61 | 0.65 | 0.67 | 0.60         |
| MultiLayer                   | 0.36 | 0.61 | 0.66 | 0.66 | 0.60         |
| Residual Block               | 0.34 | 0.71 | 0.65 | 0.66 | 0.59         |
| Data Augmentation            | 0.27 | 0.65 | 0.61 | 0.58 | 0.53         |
| Custom Stopwords             | 0.36 | 0.70 | 0.66 | 0.59 | 0.58         |
| NER                          | 0.39 | 0.71 | 0.68 | 0.69 | <b>0.62</b>  |
| Lex - Schwartz               | 0.34 | 0.68 | 0.67 | 0.66 | 0.59         |
| Lex - VAD                    | 0.37 | 0.72 | 0.65 | 0.65 | 0.60         |
| Lex - EmoLex                 | 0.38 | 0.70 | 0.65 | 0.65 | 0.60         |
| Lex - Emotion Intensity      | 0.36 | 0.70 | 0.66 | 0.68 | 0.60         |
| Lex - WorryWords             | 0.36 | 0.69 | 0.66 | 0.67 | 0.60         |
| Lex - LIWC 15                | 0.38 | 0.69 | 0.67 | 0.65 | 0.60         |
| Lex - MFD                    | 0.39 | 0.69 | 0.65 | 0.65 | 0.60         |
| Lex - LIWC 22                | 0.36 | 0.72 | 0.69 | 0.65 | 0.60         |
| Lex - LIWC 22 + Ling Feat    | 0.36 | 0.72 | 0.69 | 0.65 | 0.60         |
| Lex - MFD-20                 | 0.40 | 0.68 | 0.67 | 0.64 | 0.60         |
| Lex - eMFD                   | 0.37 | 0.68 | 0.66 | 0.65 | 0.59         |
| Lex - MJD                    | 0.39 | 0.71 | 0.66 | 0.66 | 0.61         |
| TD - LDA                     | 0.41 | 0.71 | 0.64 | 0.67 | 0.61         |
| TD - NMF                     | 0.38 | 0.70 | 0.65 | 0.67 | 0.60         |
| TD - BERTopic                | 0.37 | 0.70 | 0.68 | 0.63 | 0.60         |
| Custom Stopwords + Lex - MJD | 0.38 | 0.70 | 0.68 | 0.68 | 0.61         |
| Custom Stopwords + TD - LDA  | 0.36 | 0.73 | 0.66 | 0.66 | 0.60         |
| NER + Lex - MJD              | 0.38 | 0.71 | 0.63 | 0.67 | 0.60         |
| NER + TD - LDA               | 0.42 | 0.72 | 0.65 | 0.69 | <b>0.62</b>  |

Table S42: Test Macro- $F_1$  for moral values detection with an Openness gate. Configurations are reported as: Model (threshold) and Gate model (filter threshold). Best Macro- $F_1$  is bolded (ties included). Values are reported with 4 decimals to avoid artificial ties.

| Configuration                                                    | Macro- $F_1$  |
|------------------------------------------------------------------|---------------|
| Model: Baseline@0.50. Gate: Lex - LIWC 22 + Ling Feat@0.50       | 0.2228        |
| Model: Baseline@0.50. Gate: Lex - LIWC 22 + Ling Feat@0.82       | 0.1720        |
| Model: NER@0.50. Gate: Lex - LIWC 22 + Ling Feat@0.50            | 0.2304        |
| Model: NER@0.50. Gate: Lex - LIWC 22 + Ling Feat@0.82            | 0.1932        |
| Model: Lex - MJD@0.50. Gate: Lex - LIWC 22 + Ling Feat@0.50      | 0.2263        |
| Model: Lex - MJD@0.50. Gate: Lex - LIWC 22 + Ling Feat@0.82      | 0.1840        |
| Model: TD - LDA@0.50. Gate: Lex - LIWC 22 + Ling Feat@0.50       | 0.2241        |
| Model: TD - LDA@0.50. Gate: Lex - LIWC 22 + Ling Feat@0.82       | 0.1832        |
| Model: NER + TD - LDA@0.50. Gate: Lex - LIWC 22 + Ling Feat@0.50 | <b>0.2349</b> |
| Model: NER + TD - LDA@0.50. Gate: Lex - LIWC 22 + Ling Feat@0.82 | 0.1893        |
| Model: Baseline@0.25. Gate: Lex - LIWC 22 + Ling Feat@0.82       | 0.1958        |
| Model: NER@0.60. Gate: Lex - LIWC 22 + Ling Feat@0.50            | 0.2270        |
| Model: NER@0.35. Gate: Lex - LIWC 22 + Ling Feat@0.82            | 0.1944        |
| Model: Lex - MJD@0.55. Gate: Lex - LIWC 22 + Ling Feat@0.50      | 0.2265        |
| Model: Lex - MJD@0.25. Gate: Lex - LIWC 22 + Ling Feat@0.82      | 0.1865        |
| Model: TD - LDA@0.45. Gate: Lex - LIWC 22 + Ling Feat@0.50       | 0.2283        |
| Model: TD - LDA@0.25. Gate: Lex - LIWC 22 + Ling Feat@0.82       | 0.1946        |
| Model: NER + TD - LDA@0.35. Gate: Lex - LIWC 22 + Ling Feat@0.50 | 0.2293        |
| Model: NER + TD - LDA@0.20. Gate: Lex - LIWC 22 + Ling Feat@0.82 | 0.1899        |

Table S43: Validation F1-scores for moral values detection with a Conservation gate (macro-average over the seven moral values). Best model (by Macro- $F_1$ ) is bolded.

| Model                           | Face | Sec-per | Sec-res | Trad | Confr | Confi | Hum  | Macro- $F_1$ |
|---------------------------------|------|---------|---------|------|-------|-------|------|--------------|
| Baseline                        | 0.48 | 0.60    | 0.78    | 0.71 | 0.74  | 0.33  | 0.11 | 0.54         |
| Token Pruning                   | 0.47 | 0.56    | 0.76    | 0.66 | 0.73  | 0.30  | 0.24 | 0.53         |
| 2 prev sent w/ label            | 0.46 | 0.60    | 0.78    | 0.73 | 0.74  | 0.38  | 0.09 | 0.54         |
| MultiLayer                      | 0.47 | 0.57    | 0.78    | 0.68 | 0.74  | 0.33  | 0.04 | 0.52         |
| Residual Block                  | 0.43 | 0.60    | 0.77    | 0.68 | 0.75  | 0.37  | 0.19 | 0.54         |
| Data Augmentation               | 0.29 | 0.50    | 0.67    | 0.56 | 0.63  | 0.17  | 0.04 | 0.41         |
| Custom Stopwords                | 0.46 | 0.58    | 0.78    | 0.67 | 0.74  | 0.32  | 0.16 | 0.53         |
| NER                             | 0.49 | 0.60    | 0.78    | 0.73 | 0.75  | 0.35  | 0.20 | <b>0.56</b>  |
| Lex - Schwartz                  | 0.48 | 0.59    | 0.77    | 0.69 | 0.74  | 0.35  | 0.17 | 0.54         |
| Lex - VAD                       | 0.47 | 0.59    | 0.79    | 0.68 | 0.75  | 0.34  | 0.13 | 0.54         |
| Lex - EmoLex                    | 0.47 | 0.60    | 0.78    | 0.71 | 0.75  | 0.36  | 0.11 | 0.54         |
| Lex - Emotion Intensity         | 0.46 | 0.58    | 0.77    | 0.71 | 0.74  | 0.38  | 0.15 | 0.54         |
| Lex - WorryWords                | 0.48 | 0.58    | 0.76    | 0.71 | 0.76  | 0.35  | 0.11 | 0.54         |
| Lex - LIWC 15                   | 0.44 | 0.59    | 0.78    | 0.71 | 0.75  | 0.38  | 0.12 | 0.54         |
| Lex - MFD                       | 0.48 | 0.59    | 0.78    | 0.71 | 0.75  | 0.35  | 0.10 | 0.54         |
| Lex - LIWC 22                   | 0.45 | 0.58    | 0.76    | 0.69 | 0.76  | 0.36  | 0.16 | 0.54         |
| Lex - LIWC 22 + Ling Feat       | 0.46 | 0.58    | 0.77    | 0.70 | 0.76  | 0.37  | 0.14 | 0.54         |
| Lex - MFD-20                    | 0.46 | 0.57    | 0.78    | 0.71 | 0.74  | 0.37  | 0.15 | 0.54         |
| Lex - eMFD                      | 0.42 | 0.59    | 0.77    | 0.73 | 0.75  | 0.37  | 0.15 | 0.54         |
| Lex - MJD                       | 0.47 | 0.60    | 0.77    | 0.71 | 0.74  | 0.36  | 0.15 | 0.54         |
| TD - LDA                        | 0.45 | 0.64    | 0.79    | 0.67 | 0.75  | 0.33  | 0.13 | 0.54         |
| TD - NMF                        | 0.46 | 0.61    | 0.77    | 0.71 | 0.74  | 0.33  | 0.16 | 0.54         |
| TD - BERTopic                   | 0.48 | 0.57    | 0.77    | 0.71 | 0.73  | 0.32  | 0.18 | 0.54         |
| NER + Lex - Schwartz            | 0.45 | 0.61    | 0.79    | 0.67 | 0.75  | 0.31  | 0.12 | 0.53         |
| NER + Lex - EmoLex              | 0.45 | 0.61    | 0.79    | 0.68 | 0.75  | 0.32  | 0.12 | 0.53         |
| NER + Lex - MFD                 | 0.47 | 0.59    | 0.78    | 0.71 | 0.75  | 0.33  | 0.14 | 0.54         |
| NER + Lex - LIWC 22             | 0.45 | 0.58    | 0.78    | 0.72 | 0.75  | 0.37  | 0.11 | 0.54         |
| NER + Lex - LIWC 22 + Ling Feat | 0.45 | 0.58    | 0.78    | 0.72 | 0.75  | 0.37  | 0.11 | 0.54         |
| NER + Lex - eMFD                | 0.47 | 0.58    | 0.77    | 0.70 | 0.75  | 0.32  | 0.18 | 0.54         |
| NER + Lex - MJD                 | 0.46 | 0.59    | 0.77    | 0.70 | 0.75  | 0.33  | 0.15 | 0.54         |
| NER + TD - LDA                  | 0.45 | 0.60    | 0.78    | 0.71 | 0.75  | 0.34  | 0.22 | 0.55         |

Table S44: Test Macro- $F_1$  for moral values detection with a Conservation gate (Part 1/3). Configurations are reported as: Model (threshold) and Gate model (filter threshold). Best Macro- $F_1$  is bolded (ties included). Values are reported with 4 decimals to avoid artificial ties.

| Configuration                                                               | Macro- $F_1$  |
|-----------------------------------------------------------------------------|---------------|
| Model: Baseline@0.50. Gate: Baseline@0.50                                   | 0.2809        |
| Model: Baseline@0.50. Gate: Lex - LIWC 22 + Ling Feat@0.50                  | 0.2855        |
| Model: Baseline@0.50. Gate: Lex - LIWC 22 + Ling Feat@0.10                  | 0.2916        |
| Model: NER@0.50. Gate: Baseline@0.50                                        | 0.2823        |
| Model: NER@0.50. Gate: Lex - LIWC 22 + Ling Feat@0.50                       | 0.2841        |
| Model: NER@0.50. Gate: Lex - LIWC 22 + Ling Feat@0.10                       | 0.2937        |
| Model: Lex - Schwartz@0.50. Gate: Baseline@0.50                             | 0.2869        |
| Model: Lex - Schwartz@0.50. Gate: Lex - LIWC 22 + Ling Feat@0.50            | 0.2886        |
| Model: Lex - Schwartz@0.50. Gate: Lex - LIWC 22 + Ling Feat@0.10            | <b>0.2972</b> |
| Model: Lex - EmoLex@0.50. Gate: Baseline@0.50                               | 0.2798        |
| Model: Lex - EmoLex@0.50. Gate: Lex - LIWC 22 + Ling Feat@0.50              | 0.2835        |
| Model: Lex - EmoLex@0.50. Gate: Lex - LIWC 22 + Ling Feat@0.10              | 0.2872        |
| Model: Lex - MFD@0.50. Gate: Baseline@0.50                                  | 0.2792        |
| Model: Lex - MFD@0.50. Gate: Lex - LIWC 22 + Ling Feat@0.50                 | 0.2827        |
| Model: Lex - MFD@0.50. Gate: Lex - LIWC 22 + Ling Feat@0.10                 | 0.2874        |
| Model: Lex - LIWC 22@0.50. Gate: Baseline@0.50                              | 0.2819        |
| Model: Lex - LIWC 22@0.50. Gate: Lex - LIWC 22 + Ling Feat@0.50             | 0.2835        |
| Model: Lex - LIWC 22@0.50. Gate: Lex - LIWC 22 + Ling Feat@0.10             | 0.2872        |
| Model: Lex - LIWC 22 + Ling Feat@0.50. Gate: Baseline@0.50                  | 0.2804        |
| Model: Lex - LIWC 22 + Ling Feat@0.50. Gate: Lex - LIWC 22 + Ling Feat@0.50 | 0.2829        |
| Model: Lex - LIWC 22 + Ling Feat@0.50. Gate: Lex - LIWC 22 + Ling Feat@0.10 | 0.2913        |
| Model: Lex - eMFD@0.50. Gate: Baseline@0.50                                 | 0.2775        |
| Model: Lex - eMFD@0.50. Gate: Lex - LIWC 22 + Ling Feat@0.50                | 0.2797        |
| Model: Lex - eMFD@0.50. Gate: Lex - LIWC 22 + Ling Feat@0.10                | 0.2859        |

Table S45: Test Macro- $F_1$  for moral values detection with a Conservation gate (Part 2/3). Configurations are reported as: Model (threshold) and Gate model (filter threshold). Best Macro- $F_1$  is bolded (ties included). Values are reported with 4 decimals to avoid artificial ties.

| Configuration                                                               | Macro- $F_1$ |
|-----------------------------------------------------------------------------|--------------|
| Model: Lex - MJD@0.50. Gate: Baseline@0.50                                  | 0.2790       |
| Model: Lex - MJD@0.50. Gate: Lex - LIWC 22 + Ling Feat@0.50                 | 0.2813       |
| Model: Lex - MJD@0.50. Gate: Lex - LIWC 22 + Ling Feat@0.10                 | 0.2811       |
| Model: TD - LDA@0.50. Gate: Baseline@0.50                                   | 0.2675       |
| Model: TD - LDA@0.50. Gate: Lex - LIWC 22 + Ling Feat@0.50                  | 0.2677       |
| Model: TD - LDA@0.50. Gate: Lex - LIWC 22 + Ling Feat@0.10                  | 0.2854       |
| Model: Baseline@0.30. Gate: Baseline@0.50                                   | 0.2921       |
| Model: Baseline@0.30. Gate: Lex - LIWC 22 + Ling Feat@0.50                  | 0.2961       |
| Model: Baseline@0.40. Gate: Lex - LIWC 22 + Ling Feat@0.10                  | 0.2918       |
| Model: NER@0.15. Gate: Baseline@0.50                                        | 0.2821       |
| Model: NER@0.50. Gate: Lex - LIWC 22 + Ling Feat@0.50                       | 0.2841       |
| Model: NER@0.75. Gate: Lex - LIWC 22 + Ling Feat@0.10                       | 0.2945       |
| Model: Lex - Schwartz@0.15. Gate: Baseline@0.50                             | 0.2840       |
| Model: Lex - Schwartz@0.15. Gate: Lex - LIWC 22 + Ling Feat@0.50            | 0.2889       |
| Model: Lex - Schwartz@0.40. Gate: Lex - LIWC 22 + Ling Feat@0.10            | 0.2932       |
| Model: Lex - EmoLex@0.20. Gate: Baseline@0.50                               | 0.2836       |
| Model: Lex - EmoLex@0.20. Gate: Lex - LIWC 22 + Ling Feat@0.50              | 0.2879       |
| Model: Lex - EmoLex@0.75. Gate: Lex - LIWC 22 + Ling Feat@0.10              | 0.2934       |
| Model: Lex - MFD@0.20. Gate: Baseline@0.50                                  | 0.2828       |
| Model: Lex - MFD@0.15. Gate: Lex - LIWC 22 + Ling Feat@0.50                 | 0.2859       |
| Model: Lex - MFD@0.75. Gate: Lex - LIWC 22 + Ling Feat@0.10                 | 0.2942       |
| Model: Lex - LIWC 22@0.10. Gate: Baseline@0.50                              | 0.2795       |
| Model: Lex - LIWC 22@0.10. Gate: Lex - LIWC 22 + Ling Feat@0.50             | 0.2787       |
| Model: Lex - LIWC 22@0.45. Gate: Lex - LIWC 22 + Ling Feat@0.10             | 0.2846       |
| Model: Lex - LIWC 22 + Ling Feat@0.20. Gate: Baseline@0.50                  | 0.2806       |
| Model: Lex - LIWC 22 + Ling Feat@0.20. Gate: Lex - LIWC 22 + Ling Feat@0.50 | 0.2840       |
| Model: Lex - LIWC 22 + Ling Feat@0.65. Gate: Lex - LIWC 22 + Ling Feat@0.10 | 0.2932       |

Table S46: Test Macro- $F_1$  for moral values detection with a Conservation gate (Part 3/3). Configurations are reported as: Model (threshold) and Gate model (filter threshold). Best Macro- $F_1$  is bolded (ties included). Values are reported with 4 decimals to avoid artificial ties.

| <b>Configuration</b>                                         | <b>Macro-<math>F_1</math></b> |
|--------------------------------------------------------------|-------------------------------|
| Model: Lex - eMFD@0.20. Gate: Baseline@0.50                  | 0.2837                        |
| Model: Lex - eMFD@0.20. Gate: Lex - LIWC 22 + Ling Feat@0.50 | 0.2844                        |
| Model: Lex - eMFD@0.50. Gate: Lex - LIWC 22 + Ling Feat@0.10 | 0.2859                        |
| Model: Lex - MJD@0.25. Gate: Baseline@0.50                   | 0.2792                        |
| Model: Lex - MJD@0.50. Gate: Lex - LIWC 22 + Ling Feat@0.50  | 0.2813                        |
| Model: Lex - MJD@0.65. Gate: Lex - LIWC 22 + Ling Feat@0.10  | 0.2851                        |
| Model: TD - LDA@0.35. Gate: Baseline@0.50                    | 0.2780                        |
| Model: TD - LDA@0.35. Gate: Lex - LIWC 22 + Ling Feat@0.50   | 0.2786                        |
| Model: TD - LDA@0.50. Gate: Lex - LIWC 22 + Ling Feat@0.10   | 0.2854                        |

Table S47: Validation F1-scores for moral values detection with a Self-Transcendence gate (macro-average over the six moral values). Best model(s) (by Macro- $F_1$ ) are bolded (ties included).

| Model                                 | Hum  | Ben-c | Ben-d | Uni-c | Uni-n | Uni-t | Macro- $F_1$ |
|---------------------------------------|------|-------|-------|-------|-------|-------|--------------|
| Baseline                              | 0.31 | 0.48  | 0.53  | 0.67  | 0.92  | 0.48  | 0.57         |
| Token Pruning                         | 0.19 | 0.54  | 0.50  | 0.66  | 0.89  | 0.47  | 0.54         |
| 2 prev sent w/ label                  | 0.31 | 0.54  | 0.53  | 0.67  | 0.89  | 0.48  | 0.57         |
| MultiLayer                            | 0.00 | 0.51  | 0.52  | 0.66  | 0.90  | 0.45  | 0.51         |
| Residual Block                        | 0.38 | 0.47  | 0.51  | 0.65  | 0.89  | 0.45  | 0.56         |
| Data Augmentation                     | 0.15 | 0.40  | 0.45  | 0.59  | 0.80  | 0.37  | 0.46         |
| Custom Stopwords                      | 0.28 | 0.48  | 0.51  | 0.67  | 0.89  | 0.50  | 0.56         |
| NER                                   | 0.20 | 0.51  | 0.53  | 0.69  | 0.91  | 0.50  | 0.56         |
| Lex - Schwartz                        | 0.32 | 0.52  | 0.49  | 0.67  | 0.91  | 0.49  | 0.57         |
| Lex - VAD                             | 0.30 | 0.53  | 0.51  | 0.69  | 0.90  | 0.46  | 0.57         |
| Lex - EmoLex                          | 0.34 | 0.51  | 0.49  | 0.67  | 0.91  | 0.48  | 0.57         |
| Lex - Emotion Intensity               | 0.27 | 0.50  | 0.55  | 0.68  | 0.89  | 0.47  | 0.56         |
| Lex - WorryWords                      | 0.20 | 0.52  | 0.50  | 0.68  | 0.89  | 0.50  | 0.55         |
| Lex - LIWC 15                         | 0.31 | 0.49  | 0.49  | 0.71  | 0.89  | 0.47  | 0.56         |
| Lex - MFD                             | 0.30 | 0.54  | 0.45  | 0.68  | 0.91  | 0.48  | 0.56         |
| Lex - LIWC 22                         | 0.20 | 0.53  | 0.50  | 0.68  | 0.89  | 0.49  | 0.55         |
| Lex - LIWC 22 + Ling Feat             | 0.20 | 0.53  | 0.50  | 0.68  | 0.89  | 0.49  | 0.55         |
| Lex - MFD-20                          | 0.36 | 0.47  | 0.51  | 0.68  | 0.90  | 0.49  | 0.57         |
| Lex - eMFD                            | 0.36 | 0.48  | 0.52  | 0.68  | 0.90  | 0.47  | 0.57         |
| Lex - MJD                             | 0.24 | 0.54  | 0.49  | 0.68  | 0.90  | 0.50  | 0.56         |
| TD - LDA                              | 0.21 | 0.47  | 0.51  | 0.67  | 0.89  | 0.47  | 0.54         |
| TD - NMF                              | 0.33 | 0.50  | 0.52  | 0.66  | 0.89  | 0.47  | 0.56         |
| TD - BERTopic                         | 0.39 | 0.48  | 0.51  | 0.66  | 0.90  | 0.45  | 0.57         |
| 2 prev sent w/ label + Lex - Schwartz | 0.34 | 0.50  | 0.57  | 0.69  | 0.89  | 0.47  | <b>0.58</b>  |
| 2 prev sent w/ label + Lex - EmoLex   | 0.37 | 0.50  | 0.56  | 0.69  | 0.90  | 0.48  | <b>0.58</b>  |
| 2 prev sent w/ label + Lex - MFD      | 0.34 | 0.50  | 0.57  | 0.69  | 0.89  | 0.46  | <b>0.58</b>  |

Table S48: Test Macro- $F_1$  for moral values detection with a Self-Transcendence gate. Configurations are reported as: Model (threshold) and Gate model (filter threshold). Best Macro- $F_1$  is bolded. Values are reported with 4 decimals to avoid artificial ties.

| Configuration                                           | Macro- $F_1$  |
|---------------------------------------------------------|---------------|
| Model: Baseline@0.50. Gate: Baseline@0.50               | 0.2877        |
| Model: Baseline@0.50. Gate: Lex - MFD-20@0.50           | 0.2984        |
| Model: Baseline@0.50. Gate: Lex - WorryWords@0.16       | 0.3007        |
| Model: Baseline@0.50. Gate: Lex - MFD-20@0.21           | 0.2986        |
| Model: Baseline@0.50. Gate: TD - BERTopic@0.19          | 0.2990        |
| Model: Lex - Schwartz@0.50. Gate: Baseline@0.50         | 0.2857        |
| Model: Lex - Schwartz@0.50. Gate: Lex - MFD-20@0.50     | 0.2940        |
| Model: Lex - Schwartz@0.50. Gate: Lex - WorryWords@0.16 | 0.3014        |
| Model: Lex - Schwartz@0.50. Gate: Lex - MFD-20@0.21     | 0.2982        |
| Model: Lex - Schwartz@0.50. Gate: TD - BERTopic@0.19    | 0.3002        |
| Model: Lex - EmoLex@0.50. Gate: Baseline@0.50           | 0.2826        |
| Model: Lex - EmoLex@0.50. Gate: Lex - MFD-20@0.50       | 0.2912        |
| Model: Lex - EmoLex@0.50. Gate: Lex - WorryWords@0.16   | 0.2986        |
| Model: Lex - EmoLex@0.50. Gate: Lex - MFD-20@0.21       | 0.2965        |
| Model: Lex - EmoLex@0.50. Gate: TD - BERTopic@0.19      | 0.2985        |
| Model: Lex - MFD@0.50. Gate: Baseline@0.50              | 0.2719        |
| Model: Lex - MFD@0.50. Gate: Lex - MFD-20@0.50          | 0.2842        |
| Model: Lex - MFD@0.50. Gate: Lex - WorryWords@0.16      | 0.2955        |
| Model: Lex - MFD@0.50. Gate: Lex - MFD-20@0.21          | 0.2935        |
| Model: Lex - MFD@0.50. Gate: TD - BERTopic@0.19         | 0.2938        |
| Model: Baseline@0.15. Gate: Baseline@0.50               | 0.2948        |
| Model: Baseline@0.25. Gate: Lex - MFD-20@0.50           | <b>0.3073</b> |
| Model: Baseline@0.65. Gate: Lex - WorryWords@0.16       | 0.2936        |
| Model: Baseline@0.65. Gate: Lex - MFD-20@0.21           | 0.2877        |
| Model: Baseline@0.65. Gate: TD - BERTopic@0.19          | 0.2899        |
| Model: Lex - Schwartz@0.30. Gate: Baseline@0.50         | 0.2874        |
| Model: Lex - Schwartz@0.30. Gate: Lex - MFD-20@0.50     | 0.2970        |
| Model: Lex - Schwartz@0.40. Gate: Lex - WorryWords@0.16 | 0.3023        |
| Model: Lex - Schwartz@0.40. Gate: Lex - MFD-20@0.21     | 0.2993        |
| Model: Lex - Schwartz@0.30. Gate: TD - BERTopic@0.19    | 0.2959        |
| Model: Lex - EmoLex@0.30. Gate: Baseline@0.50           | 0.2838        |
| Model: Lex - EmoLex@0.30. Gate: Lex - MFD-20@0.50       | 0.2931        |
| Model: Lex - EmoLex@0.55. Gate: Lex - WorryWords@0.16   | 0.2993        |
| Model: Lex - EmoLex@0.60. Gate: Lex - MFD-20@0.21       | 0.2987        |
| Model: Lex - EmoLex@0.40. Gate: TD - BERTopic@0.19      | 0.2960        |
| Model: Lex - MFD@0.25. Gate: Baseline@0.50              | 0.2907        |
| Model: Lex - MFD@0.25. Gate: Lex - MFD-20@0.50          | 0.3006        |
| Model: Lex - MFD@0.50. Gate: Lex - WorryWords@0.16      | 0.2955        |
| Model: Lex - MFD@0.50. Gate: Lex - MFD-20@0.21          | 0.2935        |
| Model: Lex - MFD@0.50. Gate: TD - BERTopic@0.19         | 0.2938        |



Table S49: Validation F1-scores for moral values detection with a Self-Enhancement gate (macro-average over the five moral values). Best model (by Macro- $F_1$ ) is bolded.

| Model                        | Hed  | Ach  | Pow-d | Pow-r | Face | Macro- $F_1$ |
|------------------------------|------|------|-------|-------|------|--------------|
| Baseline                     | 0.61 | 0.72 | 0.75  | 0.71  | 0.56 | 0.67         |
| Token Pruning                | 0.62 | 0.71 | 0.73  | 0.71  | 0.51 | 0.66         |
| 2 prev sent w/ label         | 0.62 | 0.71 | 0.74  | 0.60  | 0.54 | 0.66         |
| MultiLayer                   | 0.64 | 0.70 | 0.74  | 0.72  | 0.53 | 0.67         |
| Residual Block               | 0.65 | 0.71 | 0.75  | 0.70  | 0.54 | 0.67         |
| Data Augmentation            | 0.48 | 0.61 | 0.62  | 0.62  | 0.45 | 0.56         |
| Custom Stopwords             | 0.62 | 0.70 | 0.74  | 0.71  | 0.53 | 0.66         |
| NER                          | 0.65 | 0.70 | 0.74  | 0.72  | 0.53 | 0.67         |
| Lex - Schwartz               | 0.65 | 0.72 | 0.75  | 0.71  | 0.56 | <b>0.68</b>  |
| Lex - VAD                    | 0.61 | 0.70 | 0.75  | 0.71  | 0.53 | 0.66         |
| Lex - EmoLex                 | 0.62 | 0.72 | 0.76  | 0.69  | 0.56 | 0.67         |
| Lex - Emotion Inten-<br>sity | 0.66 | 0.71 | 0.74  | 0.68  | 0.57 | 0.67         |
| Lex - WorryWords             | 0.66 | 0.70 | 0.74  | 0.70  | 0.57 | 0.67         |
| Lex - LIWC 15                | 0.62 | 0.71 | 0.74  | 0.71  | 0.55 | 0.67         |
| Lex - MFD                    | 0.64 | 0.72 | 0.76  | 0.69  | 0.56 | 0.67         |
| Lex - LIWC 22                | 0.65 | 0.70 | 0.75  | 0.69  | 0.56 | 0.67         |
| Lex - LIWC 22 +<br>Ling Feat | 0.65 | 0.70 | 0.75  | 0.69  | 0.56 | 0.67         |
| Lex - MFD-20                 | 0.63 | 0.72 | 0.75  | 0.69  | 0.56 | 0.67         |
| Lex - eMFD                   | 0.63 | 0.72 | 0.75  | 0.70  | 0.55 | 0.67         |
| Lex - MJD                    | 0.62 | 0.70 | 0.75  | 0.72  | 0.54 | 0.67         |
| TD - LDA                     | 0.64 | 0.71 | 0.75  | 0.70  | 0.55 | 0.67         |
| TD - NMF                     | 0.63 | 0.71 | 0.75  | 0.70  | 0.56 | 0.67         |
| TD - BERTopic                | 0.60 | 0.70 | 0.74  | 0.69  | 0.55 | 0.66         |

Table S50: Test Macro- $F_1$  for moral values detection with a Self-Enhancement gate. Configurations are reported as: Model (threshold) and Gate model (filter threshold). Best Macro- $F_1$  is bolded. Values are reported with 4 decimals to avoid artificial ties.

| Configuration                                           | Macro- $F_1$  |
|---------------------------------------------------------|---------------|
| Model: Baseline@0.50. Gate: Lex - MFD-20@0.50           | 0.2835        |
| Model: Baseline@0.50. Gate: TD - BERTopic@0.50          | 0.2866        |
| Model: Baseline@0.50. Gate: Lex - WorryWords@0.23       | 0.3140        |
| Model: Baseline@0.50. Gate: Lex - MFD-20@0.24           | 0.3119        |
| Model: Baseline@0.50. Gate: TD - BERTopic@0.29          | 0.3117        |
| Model: Lex - Schwartz@0.50. Gate: Lex - MFD-20@0.50     | 0.2851        |
| Model: Lex - Schwartz@0.50. Gate: TD - BERTopic@0.50    | 0.2891        |
| Model: Lex - Schwartz@0.50. Gate: Lex - WorryWords@0.23 | 0.3188        |
| Model: Lex - Schwartz@0.50. Gate: Lex - MFD-20@0.24     | 0.3135        |
| Model: Lex - Schwartz@0.50. Gate: TD - BERTopic@0.29    | 0.3145        |
| Model: Baseline@0.25. Gate: Lex - MFD-20@0.50           | 0.2951        |
| Model: Baseline@0.30. Gate: TD - BERTopic@0.50          | 0.2905        |
| Model: Baseline@0.60. Gate: Lex - WorryWords@0.23       | 0.3095        |
| Model: Baseline@0.55. Gate: Lex - MFD-20@0.24           | 0.3096        |
| Model: Baseline@0.55. Gate: TD - BERTopic@0.29          | 0.3074        |
| Model: Lex - Schwartz@0.25. Gate: Lex - MFD-20@0.50     | 0.2966        |
| Model: Lex - Schwartz@0.25. Gate: TD - BERTopic@0.50    | 0.2967        |
| Model: Lex - Schwartz@0.55. Gate: Lex - WorryWords@0.23 | <b>0.3192</b> |
| Model: Lex - Schwartz@0.55. Gate: Lex - MFD-20@0.24     | 0.3137        |
| Model: Lex - Schwartz@0.55. Gate: TD - BERTopic@0.29    | 0.3145        |

## S5. Moral value detection with higher-order category gates and LLMs

This appendix reports moral value (multi-class) detection results restricted to the moral values belonging to each higher-order category. Two complementary settings are included: (i) supervised moral value classifiers evaluated under the best higher-order category gates selected on validation, and (ii) LLM-based moral value detection using `google-gemma-2-9b-it` under analogous higher-order category constraints. For each higher-order category, we first report validation results used to select the best configuration, and then test results obtained with the selected gate/model setup.

*S5.1. Growth*

*S5.2. Self-Protection*

*S5.3. Social Focus*

*S5.4. Personal Focus*

*S5.5. Openness To Change*

*S5.6. Conservation*

*S5.7. Self-Transcendence*

*S5.8. Self-Enhancement*

Table S51: LLM (google-gemma-2-9b-it) validation F1-scores for moral values within the Growth category. Best Macro- $F_1$  is bolded.

| <b>Setup</b>                                                                                                            | <b>SD-t</b> | <b>SD-a</b> | <b>Stim</b> | <b>Hed</b> | <b>Ach</b> | <b>Hum</b> | <b>Ben-c</b> | <b>Ben-d</b> | <b>Uni-c</b> | <b>Uni-n</b> | <b>Uni-t</b> | <b>Macro</b> |
|-------------------------------------------------------------------------------------------------------------------------|-------------|-------------|-------------|------------|------------|------------|--------------|--------------|--------------|--------------|--------------|--------------|
| Zero-shot (adapted). Prompt: defi-                                                                                      | 0.09        | 0.16        | 0.12        | 0.26       | 0.23       | 0.07       | 0.19         | 0.12         | 0.20         | 0.48         | 0.14         | 0.186        |
| nition                                                                                                                  |             |             |             |            |            |            |              |              |              |              |              |              |
| Zero-shot hier (SBERT gate). Tora=0.36; Cov=0.733. Prompt: definition                                                   | 0.08        | 0.17        | 0.16        | 0.23       | 0.24       | 0.08       | 0.20         | 0.14         | 0.22         | 0.51         | 0.16         | <b>0.199</b> |
| Few-shot (adapted). Prompt: definition-12                                                                               | 0.08        | 0.14        | 0.14        | 0.24       | 0.28       | 0.05       | 0.15         | 0.13         | 0.24         | 0.53         | 0.13         | 0.192        |
| Few-shot hier (SBERT gate). Tora=0.29; Cov=0.821. Prompt: definition-12                                                 | 0.08        | 0.14        | 0.16        | 0.23       | 0.28       | 0.06       | 0.15         | 0.13         | 0.25         | 0.56         | 0.14         | 0.198        |
| QLoRA hier (SBERT gate). Args: LR=2e-4; r=8; $\alpha$ =16; epochs=3; max_seq_len=256. Tora=0; Cov=1. Prompt: definition | 0.02        | 0.17        | 0.24        | 0.27       | 0.33       | 0.07       | 0.19         | 0.21         | 0.02         | 0.21         | 0.14         | 0.170        |

Table S52: LLM (google-gemma-2-9b-it) test F1-scores for moral values within the Growth category. Best Macro- $F_1$  is bolded.

| <b>Setup</b>                          | <b>SD-t</b> | <b>SD-a</b> | <b>Stim</b> | <b>Hed</b> | <b>Ach</b> | <b>Hum</b> | <b>Ben-c</b> | <b>Ben-d</b> | <b>Uni-c</b> | <b>Uni-n</b> | <b>Uni-t</b> | <b>Macro</b> |
|---------------------------------------|-------------|-------------|-------------|------------|------------|------------|--------------|--------------|--------------|--------------|--------------|--------------|
| Zero-shot (adapted). Prompt: defi-    | 0.14        | 0.17        | 0.09        | 0.26       | 0.22       | 0.04       | 0.17         | 0.10         | 0.23         | 0.45         | 0.14         | 0.183        |
| nition                                |             |             |             |            |            |            |              |              |              |              |              |              |
| Zero-shot hier (SBERT gate).          | 0.13        | 0.18        | 0.12        | 0.26       | 0.21       | 0.03       | 0.19         | 0.09         | 0.25         | 0.50         | 0.14         | 0.192        |
| Prompt: definition                    |             |             |             |            |            |            |              |              |              |              |              |              |
| Few-shot (adapted). Prompt:           | 0.10        | 0.15        | 0.11        | 0.24       | 0.26       | 0.04       | 0.13         | 0.11         | 0.26         | 0.51         | 0.19         | 0.191        |
| definition-12                         |             |             |             |            |            |            |              |              |              |              |              |              |
| Few-shot hier (SBERT gate).           | 0.10        | 0.15        | 0.13        | 0.23       | 0.23       | 0.04       | 0.14         | 0.10         | 0.27         | 0.52         | 0.20         | <b>0.194</b> |
| Prompt: definition-12                 |             |             |             |            |            |            |              |              |              |              |              |              |
| QLoRA hier (SBERT gate). Args:        | 0.03        | 0.12        | 0.13        | 0.21       | 0.21       | 0.06       | 0.15         | 0.17         | 0.04         | 0.27         | 0.06         | 0.132        |
| LR=2e-4; r=8; $\alpha$ =16; epochs=3; |             |             |             |            |            |            |              |              |              |              |              |              |
| max_seq_len=256. Prompt: defini-      |             |             |             |            |            |            |              |              |              |              |              |              |
| tion                                  |             |             |             |            |            |            |              |              |              |              |              |              |

Table S53: LLM (google-gemma-2-9b-it) validation F1-scores for moral values within the Self-Protection category. Best Macro- $F_1$  is bolded.

| <b>Setup</b>                                                                                                                     | <b>Ach</b> | <b>Pow-d</b> | <b>Pow-r</b> | <b>Face</b> | <b>Sec-pers</b> | <b>Sec-soc</b> | <b>Trad</b> | <b>Conf-r</b> | <b>Conf-i</b> | <b>Hum</b> | <b>Macro</b> |
|----------------------------------------------------------------------------------------------------------------------------------|------------|--------------|--------------|-------------|-----------------|----------------|-------------|---------------|---------------|------------|--------------|
| Zero-shot (adapted). Prompt: def-<br>initiation                                                                                  | 0.28       | 0.21         | 0.23         | 0.18        | 0.20            | 0.26           | 0.28        | 0.32          | 0.04          | 0.09       | 0.209        |
| Zero-shot hier (SBERT gate).<br>Tora=0.28; Cov=0.832. Prompt:<br>definition                                                      | 0.30       | 0.21         | 0.23         | 0.19        | 0.21            | 0.28           | 0.30        | 0.33          | 0.05          | 0.10       | 0.222        |
| Few-shot (adapted). Prompt:<br>definition-11                                                                                     | 0.31       | 0.28         | 0.31         | 0.14        | 0.22            | 0.32           | 0.23        | 0.36          | 0.08          | 0.04       | 0.230        |
| Few-shot hier (SBERT gate).<br>Tora=0.36; Cov=0.733. Prompt:<br>definition-11                                                    | 0.30       | 0.28         | 0.32         | 0.16        | 0.23            | 0.34           | 0.27        | 0.37          | 0.09          | 0.05       | 0.239        |
| QLoRA hier (SBERT gate). Args:<br>LR=2e-4; r=8; $\alpha$ =16; epochs=3;<br>max_seq_len=256. Tora=0;<br>Cov=1. Prompt: definition | 0.33       | 0.28         | 0.28         | 0.24        | 0.33            | 0.46           | 0.40        | 0.46          | 0.04          | 0.07       | <b>0.291</b> |

Table S54: LLM (google-gemma-2-9b-it) test F1-scores for moral values within the Self-Protection category. Best Macro- $F_1$  is bolded.

| <b>Setup</b>                                                                                             | <b>Ach</b> | <b>Pow-d</b> | <b>Pow-r</b> | <b>Face</b> | <b>Sec-pers</b> | <b>Sec-soc</b> | <b>Trad</b> | <b>Conf-r</b> | <b>Conf-i</b> | <b>Hum</b> | <b>Macro</b> |
|----------------------------------------------------------------------------------------------------------|------------|--------------|--------------|-------------|-----------------|----------------|-------------|---------------|---------------|------------|--------------|
| Zero-shot (adapted). Prompt: def-<br>initiation                                                          | 0.28       | 0.19         | 0.21         | 0.16        | 0.24            | 0.24           | 0.28        | 0.30          | 0.04          | 0.09       | 0.204        |
| Zero-shot hier (SBERT gate).<br>Prompt: definition                                                       | 0.26       | 0.17         | 0.20         | 0.19        | 0.25            | 0.28           | 0.33        | 0.30          | 0.05          | 0.06       | 0.209        |
| Few-shot (adapted). Prompt: definition-11                                                                | 0.27       | 0.23         | 0.32         | 0.12        | 0.26            | 0.30           | 0.20        | 0.36          | 0.07          | 0.06       | 0.220        |
| Few-shot hier (SBERT gate).<br>Prompt: definition-11                                                     | 0.20       | 0.21         | 0.31         | 0.11        | 0.25            | 0.32           | 0.25        | 0.34          | 0.08          | 0.04       | 0.212        |
| QLoRA hier (SBERT gate). Args: LR=2e-4; r=8; $\alpha$ =16; epochs=3; max_seq_len=256. Prompt: definition | 0.21       | 0.22         | 0.31         | 0.18        | 0.25            | 0.41           | 0.47        | 0.38          | 0.05          | 0.06       | <b>0.254</b> |

Table S55: LLM (google-gemma-2-9b-it) validation F1-scores for moral values within the Social Focus category. Best Macro- $F_1$  is bolded.

| <b>Setup</b>                                                                                                            | <b>Sec-soc</b> | <b>Trad</b> | <b>Confr-r</b> | <b>Confi</b> | <b>Hum</b> | <b>Ben-c</b> | <b>Ben-d</b> | <b>Uni-c</b> | <b>Uni-n</b> | <b>Uni-t</b> | <b>Macro</b> |
|-------------------------------------------------------------------------------------------------------------------------|----------------|-------------|----------------|--------------|------------|--------------|--------------|--------------|--------------|--------------|--------------|
| Zero-shot (adapted). Prompt: definition                                                                                 | 0.06           | 0.24        | 0.27           | 0.07         | 0.05       | 0.25         | 0.09         | 0.30         | 0.48         | 0.13         | 0.194        |
| Zero-shot hier (SBERT gate). Tora=0.38; Cov=0.703. Prompt: definition                                                   | 0.05           | 0.28        | 0.31           | 0.08         | 0.03       | 0.25         | 0.09         | 0.31         | 0.54         | 0.13         | 0.207        |
| Few-shot (adapted). Prompt: definition-11                                                                               | 0.37           | 0.37        | 0.31           | 0.08         | 0.07       | 0.22         | 0.08         | 0.28         | 0.55         | 0.16         | 0.247        |
| Few-shot hier (SBERT gate). Tora=0.38; Cov=0.703. Prompt: definition-11                                                 | 0.38           | 0.37        | 0.32           | 0.08         | 0.07       | 0.22         | 0.08         | 0.28         | 0.57         | 0.17         | <b>0.253</b> |
| QLoRA hier (SBERT gate). Args: LR=2e-4; r=8; $\alpha$ =16; epochs=3; max_seq_len=256. Tora=0; Cov=1. Prompt: definition | 0.46           | 0.40        | 0.46           | 0.04         | 0.07       | 0.19         | 0.21         | 0.02         | 0.21         | 0.14         | 0.221        |



Table S56: LLM (google-gemma-2-9b-it) test F1-scores for moral values within the Social Focus category. Best Macro- $F_1$  is bolded.

| <b>Setup</b>                                                                                             | <b>Sec-soc</b> | <b>Trad</b> | <b>Confr</b> | <b>Confr</b> | <b>Conf-i</b> | <b>Hum</b> | <b>Ben-c</b> | <b>Ben-d</b> | <b>Uni-c</b> | <b>Uni-n</b> | <b>Uni-t</b> | <b>Macro</b> |
|----------------------------------------------------------------------------------------------------------|----------------|-------------|--------------|--------------|---------------|------------|--------------|--------------|--------------|--------------|--------------|--------------|
| Zero-shot (adapted). Prompt: definition                                                                  | 0.06           | 0.20        | 0.25         | 0.07         | 0.07          | 0.08       | 0.25         | 0.07         | 0.34         | 0.46         | 0.14         | 0.193        |
| Zero-shot hier (SBERT gate). Prompt: definition                                                          | 0.06           | 0.28        | 0.29         | 0.07         | 0.07          | 0.05       | 0.23         | 0.06         | 0.35         | 0.53         | 0.13         | 0.205        |
| Few-shot (adapted). Prompt: definition-11                                                                | 0.33           | 0.32        | 0.29         | 0.06         | 0.06          | 0.04       | 0.22         | 0.03         | 0.32         | 0.52         | 0.17         | 0.230        |
| Few-shot hier (SBERT gate). Prompt: definition-11                                                        | 0.34           | 0.33        | 0.29         | 0.08         | 0.08          | 0.05       | 0.21         | 0.02         | 0.31         | 0.54         | 0.18         | <b>0.234</b> |
| QLoRA hier (SBERT gate). Args: LR=2e-4; r=8; $\alpha$ =16; epochs=3; max_seq_len=256. Prompt: definition | 0.41           | 0.47        | 0.38         | 0.05         | 0.05          | 0.06       | 0.15         | 0.17         | 0.04         | 0.27         | 0.06         | 0.206        |

Table S57: LLM (google-gemma-2-9b-it) validation F1-scores for moral values within the Personal Focus category. Best Macro- $F_1$  is bolded.

| Setup                                            | SD-t | SD-a | Stim | Hed  | Ach  | Pow-d | Pow-r | Face | Sec-per | Macro        |
|--------------------------------------------------|------|------|------|------|------|-------|-------|------|---------|--------------|
| Zero-shot (adapted). Prompt: definition          | 0.10 | 0.15 | 0.15 | 0.32 | 0.30 | 0.26  | 0.22  | 0.13 | 0.06    | 0.188        |
| Zero-shot hier (SBERT gate). Tora=0.25;          | 0.10 | 0.15 | 0.18 | 0.31 | 0.32 | 0.26  | 0.23  | 0.14 | 0.06    | 0.194        |
| Cov=0.865. Prompt: definition                    |      |      |      |      |      |       |       |      |         |              |
| Few-shot (adapted). Prompt: definition-10        | 0.11 | 0.20 | 0.15 | 0.25 | 0.32 | 0.32  | 0.28  | 0.14 | 0.08    | 0.205        |
| Few-shot hier (SBERT gate). Tora=0.29;           | 0.11 | 0.20 | 0.17 | 0.24 | 0.32 | 0.32  | 0.29  | 0.15 | 0.08    | 0.209        |
| Cov=0.821. Prompt: definition-10                 |      |      |      |      |      |       |       |      |         |              |
| QLoRA hier (SBERT gate). Args: LR=2e-4; r=8;     | 0.02 | 0.17 | 0.24 | 0.27 | 0.33 | 0.28  | 0.28  | 0.24 | 0.33    | <b>0.241</b> |
| $\alpha=16$ ; epochs=3; max_seq_len=256. Tora=0; |      |      |      |      |      |       |       |      |         |              |
| Cov=1. Prompt: definition                        |      |      |      |      |      |       |       |      |         |              |

Table S58: LLM (google-gemma-2-9b-it) test F1-scores for moral values within the Personal Focus category. Best Macro- $F_1$  is bolded.

| <b>Setup</b>                                                                                             | <b>SD-t</b> | <b>SD-a</b> | <b>Stim</b> | <b>Hed</b> | <b>Ach</b> | <b>Pow-d</b> | <b>Pow-r</b> | <b>Face</b> | <b>Sec-per</b> | <b>Macro</b> |
|----------------------------------------------------------------------------------------------------------|-------------|-------------|-------------|------------|------------|--------------|--------------|-------------|----------------|--------------|
| Zero-shot (adapted). Prompt: definition                                                                  | 0.13        | 0.16        | 0.13        | 0.31       | 0.29       | 0.23         | 0.23         | 0.14        | 0.07           | 0.187        |
| Zero-shot hier (SBERT gate). Prompt: definition                                                          | 0.13        | 0.14        | 0.15        | 0.27       | 0.26       | 0.21         | 0.21         | 0.17        | 0.08           | 0.179        |
| Few-shot (adapted). Prompt: definition-10                                                                | 0.14        | 0.17        | 0.12        | 0.24       | 0.31       | 0.26         | 0.30         | 0.15        | 0.10           | <b>0.198</b> |
| Few-shot hier (SBERT gate). Prompt: definition-10                                                        | 0.13        | 0.14        | 0.12        | 0.29       | 0.25       | 0.26         | 0.29         | 0.16        | 0.10           | 0.195        |
| QLoRA hier (SBERT gate). Args: LR=2e-4; r=8; $\alpha$ =16; epochs=3; max_seq_len=256. Prompt: definition | 0.03        | 0.12        | 0.13        | 0.21       | 0.21       | 0.22         | 0.31         | 0.18        | 0.25           | 0.184        |

Table S59: LLM (google-gemma-2-9b-it) validation F1-scores for moral values within the Openness category. Best Macro- $F_1$  is bolded.

| Setup                                                                                                                            | SD-t | SD-a | Stim | Hed  | Macro        |
|----------------------------------------------------------------------------------------------------------------------------------|------|------|------|------|--------------|
| Zero-shot (adapted). Prompt: definition                                                                                          | 0.07 | 0.07 | 0.09 | 0.10 | 0.084        |
| Zero-shot hier (SBERT gate).<br>Tora=0.39; Cov=0.686. Prompt:<br>definition                                                      | 0.08 | 0.07 | 0.13 | 0.08 | 0.089        |
| Few-shot (adapted). Prompt: definition-<br>5                                                                                     | 0.06 | 0.11 | 0.10 | 0.09 | 0.089        |
| Few-shot hier (SBERT gate). Tora=0.58;<br>Cov=0.387. Prompt: definition-5                                                        | 0.05 | 0.12 | 0.15 | 0.07 | 0.100        |
| QLoRA hier (SBERT gate). Args:<br>LR=2e-4; r=8; $\alpha$ =16; epochs=3;<br>max_seq_len=256. Tora=0; Cov=1.<br>Prompt: definition | 0.02 | 0.17 | 0.24 | 0.27 | <b>0.175</b> |

Table S60: LLM (google-gemma-2-9b-it) test F1-scores for moral values within the Openness category. Best Macro- $F_1$  is bolded.

| Setup                                                                                                          | SD-t | SD-a | Stim | Hed  | Macro        |
|----------------------------------------------------------------------------------------------------------------|------|------|------|------|--------------|
| Zero-shot (adapted). Prompt: definition                                                                        | 0.09 | 0.05 | 0.08 | 0.09 | 0.078        |
| Zero-shot hier (SBERT gate). Prompt:<br>definition                                                             | 0.10 | 0.05 | 0.12 | 0.10 | 0.090        |
| Few-shot (adapted). Prompt: definition-<br>5                                                                   | 0.07 | 0.13 | 0.08 | 0.09 | 0.093        |
| Few-shot hier (SBERT gate). Prompt:<br>definition-5                                                            | 0.07 | 0.14 | 0.12 | 0.12 | 0.113        |
| QLoRA hier (SBERT gate). Args:<br>LR=2e-4; r=8; $\alpha$ =16; epochs=3;<br>max_seq_len=256. Prompt: definition | 0.03 | 0.12 | 0.13 | 0.21 | <b>0.123</b> |

Table S61: LLM (google-gemma-2-9b-it) validation F1-scores for moral values within the Conservation category. Best Macro- $F_1$  is bolded.

| Setup                                                                                                                   | Face | Sec-per | Sec-soc | Trad | Conf-r | Conf-i | Hum  | Macro        |
|-------------------------------------------------------------------------------------------------------------------------|------|---------|---------|------|--------|--------|------|--------------|
| Zero-shot (adapted). Prompt: definition                                                                                 | 0.20 | 0.21    | 0.24    | 0.25 | 0.29   | 0.05   | 0.07 | 0.187        |
| Zero-shot hier (SBERT gate). Tora=0.45; Cov=0.592. Prompt: definition                                                   | 0.23 | 0.22    | 0.28    | 0.30 | 0.33   | 0.06   | 0.08 | 0.214        |
| Few-shot (adapted). Prompt: definition-8                                                                                | 0.22 | 0.27    | 0.38    | 0.34 | 0.34   | 0.07   | 0.03 | 0.237        |
| Few-shot hier (SBERT gate). Tora=0.39; Cov=0.686. Prompt: definition-8                                                  | 0.23 | 0.28    | 0.39    | 0.34 | 0.36   | 0.08   | 0.04 | 0.243        |
| QLoRA hier (SBERT gate). Args: LR=2e-4; r=8; $\alpha$ =16; epochs=3; max_seq_len=256. Tora=0; Cov=1. Prompt: definition | 0.24 | 0.33    | 0.46    | 0.40 | 0.46   | 0.04   | 0.07 | <b>0.289</b> |

Table S62: LLM (google-gemma-2-9b-it) test F1-scores for moral values within the Conservation category. Best Macro- $F_1$  is bolded.

| Setup                                                                                                    | Face | Sec-per | Sec-soc | Trad | Conf-r | Conf-i | Hum  | Macro        |
|----------------------------------------------------------------------------------------------------------|------|---------|---------|------|--------|--------|------|--------------|
| Zero-shot (adapted). Prompt: definition                                                                  | 0.18 | 0.26    | 0.22    | 0.23 | 0.28   | 0.04   | 0.05 | 0.182        |
| Zero-shot hier (SBERT gate). Prompt: definition                                                          | 0.21 | 0.28    | 0.27    | 0.31 | 0.30   | 0.05   | 0.04 | 0.210        |
| Few-shot (adapted). Prompt: definition-8                                                                 | 0.16 | 0.32    | 0.35    | 0.29 | 0.34   | 0.07   | 0.08 | 0.230        |
| Few-shot hier (SBERT gate). Prompt: definition-8                                                         | 0.15 | 0.30    | 0.36    | 0.31 | 0.34   | 0.08   | 0.05 | 0.227        |
| QLoRA hier (SBERT gate). Args: LR=2e-4; r=8; $\alpha$ =16; epochs=3; max_seq_len=256. Prompt: definition | 0.18 | 0.25    | 0.41    | 0.47 | 0.38   | 0.05   | 0.06 | <b>0.258</b> |

Table S63: LLM (google-gemma-2-9b-it) validation F1-scores for moral values within the Self-Transcendence category. Best Macro- $F_1$  is bolded.

| Setup                                                                                                                          | Hum  | Ben-C | Ben-D | Univ-C | Univ-N | Univ-T | Macro        |
|--------------------------------------------------------------------------------------------------------------------------------|------|-------|-------|--------|--------|--------|--------------|
| Zero-shot (adapted). Prompt: definition                                                                                        | 0.05 | 0.18  | 0.07  | 0.15   | 0.40   | 0.11   | 0.161        |
| Zero-shot hier (SBERT gate). Tora=0.47; Cov=0.561. Prompt: definition                                                          | 0.07 | 0.18  | 0.09  | 0.18   | 0.47   | 0.13   | 0.186        |
| Few-shot (adapted). Prompt: definition-7                                                                                       | 0.07 | 0.20  | 0.14  | 0.18   | 0.48   | 0.13   | 0.202        |
| Few-shot hier (SBERT gate). Tora=0.38; Cov=0.703. Prompt: definition-7                                                         | 0.08 | 0.20  | 0.15  | 0.19   | 0.53   | 0.14   | <b>0.216</b> |
| QLoRA hier (SBERT gate). Args: LR=2e-4; r=8; $\alpha$ =16; epochs=3; max_seq_len=256. Tora=0.29; Cov=0.821. Prompt: definition | 0.08 | 0.19  | 0.21  | 0.02   | 0.21   | 0.14   | 0.141        |

Table S64: LLM (google-gemma-2-9b-it) test F1-scores for moral values within the Self-Transcendence category. Best Macro- $F_1$  is bolded.

| Setup                                                                                                    | Hum  | Ben-c | Ben-d | Uni-c | Uni-n | Uni-t | Macro        |
|----------------------------------------------------------------------------------------------------------|------|-------|-------|-------|-------|-------|--------------|
| Zero-shot (adapted). Prompt: definition                                                                  | 0.03 | 0.19  | 0.08  | 0.18  | 0.36  | 0.12  | 0.159        |
| Zero-shot hier (SBERT gate). Prompt: definition                                                          | 0.01 | 0.19  | 0.11  | 0.21  | 0.45  | 0.14  | 0.187        |
| Few-shot (adapted). Prompt: definition-7                                                                 | 0.15 | 0.20  | 0.14  | 0.21  | 0.45  | 0.14  | 0.213        |
| Few-shot hier (SBERT gate). Prompt: definition-7                                                         | 0.12 | 0.20  | 0.13  | 0.23  | 0.50  | 0.15  | <b>0.221</b> |
| QLoRA hier (SBERT gate). Args: LR=2e-4; r=8; $\alpha$ =16; epochs=3; max_seq_len=256. Prompt: definition | 0.06 | 0.15  | 0.17  | 0.04  | 0.27  | 0.06  | 0.124        |

Table S65: LLM (google-gemma-2-9b-it) validation F1-scores for moral values within the Self-Enhancement category. Best Macro- $F_1$  is bolded.

| <b>Setup</b>                                                                                                                   | <b>Hed</b> | <b>Ach</b> | <b>Pow-d</b> | <b>Pow-r</b> | <b>Face</b> | <b>Macro</b> |
|--------------------------------------------------------------------------------------------------------------------------------|------------|------------|--------------|--------------|-------------|--------------|
| Zero-shot (adapted). Prompt: definition                                                                                        | 0.16       | 0.25       | 0.18         | 0.21         | 0.08        | 0.178        |
| Zero-shot hier (SBERT gate). Tora=0.39; Cov=0.686. Prompt: definition                                                          | 0.16       | 0.27       | 0.18         | 0.23         | 0.08        | 0.186        |
| Few-shot (adapted). Prompt: definition-6                                                                                       | 0.14       | 0.32       | 0.29         | 0.29         | 0.10        | 0.229        |
| Few-shot hier (SBERT gate). Tora=0.34; Cov=0.761. Prompt: definition-6                                                         | 0.15       | 0.33       | 0.30         | 0.30         | 0.10        | 0.235        |
| QLoRA hier (SBERT gate). Args: LR=2e-4; r=8; $\alpha$ =16; epochs=3; max_seq_len=256. Tora=0.11; Cov=0.976. Prompt: definition | 0.27       | 0.33       | 0.28         | 0.28         | 0.24        | <b>0.281</b> |

Table S66: LLM (google-gemma-2-9b-it) test F1-scores for moral values within the Self-Enhancement category. Best Macro- $F_1$  is bolded.

| <b>Setup</b>                                                                                             | <b>Hed</b> | <b>Ach</b> | <b>Pow-d</b> | <b>Pow-r</b> | <b>Face</b> | <b>Macro</b> |
|----------------------------------------------------------------------------------------------------------|------------|------------|--------------|--------------|-------------|--------------|
| Zero-shot (adapted). Prompt: definition                                                                  | 0.17       | 0.25       | 0.16         | 0.22         | 0.08        | 0.175        |
| Zero-shot hier (SBERT gate). Prompt: definition                                                          | 0.19       | 0.25       | 0.15         | 0.24         | 0.09        | 0.182        |
| Few-shot (adapted). Prompt: definition-6                                                                 | 0.16       | 0.31       | 0.23         | 0.31         | 0.09        | 0.221        |
| Few-shot hier (SBERT gate). Prompt: definition-6                                                         | 0.22       | 0.25       | 0.21         | 0.32         | 0.11        | 0.222        |
| QLoRA hier (SBERT gate). Args: LR=2e-4; r=8; $\alpha$ =16; epochs=3; max_seq_len=256. Prompt: definition | 0.21       | 0.21       | 0.22         | 0.31         | 0.18        | <b>0.227</b> |

## S6. Ensembles

This appendix reports ensemble results for moral value detection under higher-order category (HO) gates. For each HO category, we evaluate: (i) ensembles built from transformer-based moral-value detectors using the best HO gate models; (ii) ensembles of the best ensembles from (i); (iii) ensembles across architectures combining the HO-gated champion with the best direct and presence-based champions; (iv) ensembles of LLM-based detectors (only when the best validation ensemble contains more than one LLM); and (v) ensembles combining the best transformer ensemble with the best LLM ensemble (only when the best validation ensemble contains more than one model). Results are reported for Validation and Test. Thresholds of 0.50 correspond to fixed settings; any other numeric threshold indicates a tuned global threshold, while *CS* denotes class-specific tuned thresholds.

### S6.1. Growth

Table S67: Transformer ensembles for moral value detection within *Growth* using the best Growth gate models (Validation). Redundant single-member rows are omitted. Best Macro- $F_1$  is bolded (ties included).

| Configuration                                         | Ensemble | Thr  | Macro- $F_1$  |
|-------------------------------------------------------|----------|------|---------------|
| Model: Baseline@0.50. Gate: Baseline@0.50             | Single   | 0.50 | 0.2682        |
| Model: Baseline@0.50. Gate: Previous-Sentences-2@0.50 | Single   | 0.30 | <b>0.2701</b> |
| Model: Baseline@0.50. Gate: Previous-Sentences-2@0.50 | Soft     | 0.38 | 0.2698        |
| Model: Baseline@0.50. Gate: Previous-Sentences-2@0.18 | Single   | 0.50 | 0.2649        |
| Model: Baseline@0.50. Gate: Previous-Sentences-2@0.18 | Single   | 0.60 | 0.2654        |
| Model: Baseline@0.50. Gate: Previous-Sentences-2@0.18 | Soft     | 0.53 | 0.2652        |



Table S68: Transformer ensembles of the best Growth transformer ensembles (Growth (all), Validation). Best Macro- $F_1$  is bolded (ties included).

| Configuration                                         | Ensemble | Thr  | Macro- $F_1$  |
|-------------------------------------------------------|----------|------|---------------|
| Model: Baseline@0.50. Gate: Previous-Sentences-2@0.50 | Single   | 0.50 | 0.2670        |
| Model: Baseline@0.50. Gate: Previous-Sentences-2@0.50 | Single   | 0.45 | <b>0.2701</b> |
| Model: Baseline@0.50. Gate: Previous-Sentences-2@0.50 | Soft     | 0.48 | 0.2665        |

Table S69: Transformer ensembles across architectures (Values-Growth-All architectures, Validation). Best Macro- $F_1$  is bolded (ties included).

| Configuration                                                             | Ensemble | Thr  | Macro- $F_1$  |
|---------------------------------------------------------------------------|----------|------|---------------|
| Model: Baseline@0.50. Gate: Previous-Sentences-2@0.50                     | Single   | 0.50 | 0.2670        |
| Model: Baseline@0.50. Gate: Previous-Sentences-2@0.50 + Presence champion | Hard     | 0.50 | 0.2881        |
| Direct champion                                                           | Single   | 0.30 | <b>0.2898</b> |
| Direct champion                                                           | Soft     | 0.32 | 0.2867        |

Table S70: Transformer ensembles across architectures (Values-Growth-All architectures, Test). Best Macro- $F_1$  is bolded (ties included).

| Configuration   | Ensemble | Thr  | Macro- $F_1$  |
|-----------------|----------|------|---------------|
| Direct champion | Single   | 0.50 | 0.2518        |
| Direct champion | Single   | 0.30 | 0.2962        |
| Direct champion | Soft     | 0.32 | <b>0.3028</b> |

Table S71: LLM ensembles for Growth (Validation). The LLM is `google-gemma-2-9b-it`. Best Macro- $F_1$  is bolded (ties included).

| Configuration                                                                                                       | Ensemble | Thr  | Macro- $F_1$  |
|---------------------------------------------------------------------------------------------------------------------|----------|------|---------------|
| Gemma2: zero-shot hier (SBERT gate: Growth)                                                                         | Weighted | 0.50 | 0.1988        |
| Gemma2 ensemble: [zero-shot hier (SBERT gate: Growth) + QLoRA hier (SBERT gate: Growth) + few-shot $k=12$ (direct)] | Hard     | 0.50 | <b>0.2384</b> |
| Gemma2 ensemble: [zero-shot hier (SBERT gate: Growth) + QLoRA hier (SBERT gate: Growth) + few-shot $k=12$ (direct)] | Soft     | 0.50 | <b>0.2384</b> |

Table S72: LLM ensembles for Growth (Test). Best Macro- $F_1$  is bolded (ties included).

| Configuration                                                                                                       | Ensemble | Thr  | Macro- $F_1$  |
|---------------------------------------------------------------------------------------------------------------------|----------|------|---------------|
| Gemma2 ensemble: [zero-shot hier (SBERT gate: Growth) + QLoRA hier (SBERT gate: Growth) + few-shot $k=12$ (direct)] | Hard     | 0.50 | <b>0.2013</b> |
| Gemma2 ensemble: [zero-shot hier (SBERT gate: Growth) + QLoRA hier (SBERT gate: Growth) + few-shot $k=12$ (direct)] | Weighted | 0.50 | <b>0.2013</b> |
| Gemma2 ensemble: [zero-shot hier (SBERT gate: Growth) + QLoRA hier (SBERT gate: Growth) + few-shot $k=12$ (direct)] | Soft     | 0.50 | <b>0.2013</b> |

Table S73: Transformer + LLM ensembles for Growth (Validation). Best Macro- $F_1$  is bolded (ties included).

| Configuration                                           | Ensemble | Thr  | Macro- $F_1$  |
|---------------------------------------------------------|----------|------|---------------|
| Direct champion + Best Growth LLM ensemble (fixed hard) | Hard     | 0.50 | 0.2670        |
| Direct champion                                         | Hard     | CS   | <b>0.2898</b> |
| Direct champion                                         | Soft     | 0.25 | 0.2873        |

Table S74: Transformer ensembles for moral value detection within *Self-Protection* using the best Self-Protection gate models (Validation). Best Macro- $F_1$  is bolded (ties included).

| Configuration                              | Ensemble | Thr  | Macro- $F_1$  |
|--------------------------------------------|----------|------|---------------|
| Model: Baseline@0.50. Gate: Base-line@0.50 | Single   | 0.50 | 0.2953        |
| Model: Baseline@0.50. Gate: Base-line@0.50 | Single   | 0.15 | 0.3005        |
| Model: Baseline@0.50. Gate: Base-line@0.50 | Soft     | 0.12 | 0.3039        |
| Model: Baseline@0.50. Gate: Base-line@0.10 | Single   | 0.50 | 0.3055        |
| Model: Baseline@0.50. Gate: Base-line@0.10 | Single   | 0.60 | <b>0.3061</b> |
| Model: Baseline@0.50. Gate: Base-line@0.10 | Soft     | 0.60 | <b>0.3061</b> |

Table S75: Transformer ensembles of the best Self-Protection transformer ensembles (Self-Protection (all), Validation). Best Macro- $F_1$  is bolded (ties included).

| Configuration                              | Ensemble | Thr  | Macro- $F_1$  |
|--------------------------------------------|----------|------|---------------|
| Model: Baseline@0.50. Gate: Base-line@0.10 | Single   | 0.50 | 0.3055        |
| Model: Baseline@0.50. Gate: Base-line@0.10 | Single   | 0.60 | <b>0.3061</b> |
| Model: Baseline@0.50. Gate: Base-line@0.10 | Soft     | 0.47 | 0.3042        |

Table S76: Transformer ensembles across architectures (Values-Self-Protection-All architectures, Validation). Best Macro- $F_1$  is bolded (ties included).

| Configuration                       | Ensemble | Thr  | Macro- $F_1$  |
|-------------------------------------|----------|------|---------------|
| Direct champion                     | Single   | 0.50 | 0.3081        |
| Direct champion + Presence champion | Hard     | 0.50 | 0.3263        |
| Direct champion                     | Single   | CS   | <b>0.3386</b> |
| Direct champion                     | Soft     | 0.32 | 0.3357        |

Table S77: Transformer ensembles across architectures (Values–Self-Protection–All architectures, Test). Best Macro- $F_1$  is bolded (ties included).

| Configuration   | Ensemble | Thr  | Macro- $F_1$  |
|-----------------|----------|------|---------------|
| Direct champion | Single   | 0.50 | 0.3030        |
| Direct champion | Single   | 0.30 | 0.3356        |
| Direct champion | Soft     | 0.29 | <b>0.3416</b> |

Table S78: LLM ensembles for Self-Protection (Validation). The LLM is google-gemma-2-9b-it. Best Macro- $F_1$  is bolded (ties included).

| Configuration                                   | Ensemble | Thr  | Macro- $F_1$  |
|-------------------------------------------------|----------|------|---------------|
| Gemma2 QLoRA hier (SBERT gate: Self-Protection) | Single   | 0.50 | <b>0.2913</b> |

Table S79: Transformer + LLM ensembles for Self-Protection (Validation). Best Macro- $F_1$  is bolded (ties included).

| Configuration                                                     | Ensemble | Thr  | Macro- $F_1$  |
|-------------------------------------------------------------------|----------|------|---------------|
| Direct champion + Gemma2 QLoRA hier (SBERT gate: Self-Protection) | Hard     | 0.50 | 0.3507        |
| Direct champion + Gemma2 QLoRA hier (SBERT gate: Self-Protection) | Hard     | CS   | <b>0.3574</b> |
| Direct champion + Gemma2 QLoRA hier (SBERT gate: Self-Protection) | Soft     | 0.15 | <b>0.3574</b> |

Table S80: Transformer + LLM ensembles for Self-Protection (Test). Best Macro- $F_1$  is bolded (ties included).

| Configuration                                                     | Ensemble | Thr  | Macro- $F_1$  |
|-------------------------------------------------------------------|----------|------|---------------|
| Direct champion + Gemma2 QLoRA hier (SBERT gate: Self-Protection) | Hard     | 0.50 | 0.3408        |
| Direct champion + Gemma2 QLoRA hier (SBERT gate: Self-Protection) | Hard     | CS   | <b>0.3526</b> |
| Direct champion + Gemma2 QLoRA hier (SBERT gate: Self-Protection) | Soft     | 0.15 | <b>0.3526</b> |

Table S81: Transformer ensembles for moral value detection within *Social Focus* using the best Social Focus gate models (Validation). Best Macro- $F_1$  is bolded (ties included).

| Configuration                                         | Ensemble        | Thr  | Macro- $F_1$  |
|-------------------------------------------------------|-----------------|------|---------------|
| Model: Lex-LIWC@0.50. Gate: NER@0.10                  | Single          | 0.50 | 0.3197        |
| Model: Lex-LIWC@0.50. Gate: NER@0.10                  | Single          | 0.55 | 0.3219        |
| Model: Lex-WorryWords@0.50. Gate: NER@0.10            | Single          | 0.50 | 0.3175        |
| Model: Lex-WorryWords@0.50. Gate: NER@0.10            | Single          | 0.55 | 0.3191        |
| Model: NER@0.50. Gate: Baseline@0.10                  | Single          | 0.50 | 0.3210        |
| Model: NER@0.50. Gate: Baseline@0.10                  | Single          | 0.55 | <b>0.3223</b> |
| Model: 2 prev sent w/ label@0.50. Gate: Baseline@0.10 | Single          | 0.50 | 0.3163        |
| Model: 2 prev sent w/ label@0.50. Gate: Baseline@0.10 | Single          | 0.55 | 0.3171        |
| Model: TD-NMF@0.50. Gate: NER@0.50                    | Single          | 0.50 | 0.2994        |
| Model: TD-NMF@0.50. Gate: NER@0.50                    | Hard (2 models) | 0.50 | 0.3088        |
| Model: TD-NMF@0.50. Gate: NER@0.50                    | Single          | 0.25 | 0.3108        |
| Model: TD-NMF@0.50. Gate: NER@0.50                    | Soft            | 0.20 | 0.3108        |

Table S82: Transformer ensembles of the best Social Focus transformer ensembles (Social Focus (all), Validation). Best Macro- $F_1$  is bolded (ties included).

| Configuration                        | Ensemble | Thr  | Macro- $F_1$  |
|--------------------------------------|----------|------|---------------|
| Model: NER@0.50. Gate: Baseline@0.10 | Single   | 0.50 | 0.3210        |
| Model: NER@0.50. Gate: Baseline@0.10 | Single   | 0.55 | <b>0.3223</b> |
| Model: Lex-LIWC@0.50. Gate: NER@0.10 | Soft     | 0.34 | 0.3189        |

Table S83: Transformer ensembles across architectures (Values–Social Focus–All architectures, Validation). Best Macro- $F_1$  is bolded (ties included).

| Configuration                                           | Ensemble        | Thr  | Macro- $F_1$  |
|---------------------------------------------------------|-----------------|------|---------------|
| Model: NER@0.50. Gate: Base-line@0.10                   | Single          | 0.50 | 0.3210        |
| Model: NER@0.50. Gate: Base-line@0.10 + Direct champion | Hard (2 models) | 0.50 | 0.3296        |
| Direct champion                                         | Single          | CS   | <b>0.3424</b> |
| Direct champion                                         | Soft            | 0.35 | 0.3319        |

Table S84: Transformer ensembles across architectures (Values–Social Focus–All architectures, Test). Best Macro- $F_1$  is bolded (ties included).

| Configuration   | Ensemble | Thr  | Macro- $F_1$  |
|-----------------|----------|------|---------------|
| Direct champion | Single   | 0.50 | 0.3009        |
| Direct champion | Single   | 0.30 | 0.3393        |
| Direct champion | Soft     | 0.29 | <b>0.3455</b> |

Table S85: LLM ensembles for Social Focus (Validation). The LLM is google-gemma-2-9b-it. Best Macro- $F_1$  is bolded (ties included).

| Configuration                                                              | Ensemble | Thr  | Macro- $F_1$  |
|----------------------------------------------------------------------------|----------|------|---------------|
| Gemma2 few-shot hier (k=11) + Gemma2 QLoRA hier (SBERT gate: Social Focus) | Hard     | 0.50 | <b>0.2810</b> |
| Gemma2 few-shot hier (k=11) + Gemma2 QLoRA hier (SBERT gate: Social Focus) | Soft     | 0.50 | <b>0.2810</b> |

Table S86: LLM ensembles for Social Focus (Test). Best Macro- $F_1$  is bolded (ties included).

| Configuration                                                              | Ensemble | Thr         | Macro- $F_1$  |
|----------------------------------------------------------------------------|----------|-------------|---------------|
| Gemma2 few-shot hier (k=11) + Gemma2 QLoRA hier (SBERT gate: Social Focus) | Hard     | <b>0.50</b> | <b>0.2667</b> |
| Gemma2 few-shot hier (k=11) + Gemma2 QLoRA hier (SBERT gate: Social Focus) | Soft     | <b>0.50</b> | <b>0.2667</b> |

Table S87: Transformer + LLM ensembles for Social Focus (Validation). Best Macro- $F_1$  is bolded (ties included).

| Configuration                                    | Ensemble | Thr  | Macro- $F_1$  |
|--------------------------------------------------|----------|------|---------------|
| Direct champion                                  | Single   | 0.50 | 0.3034        |
| Direct champion                                  | Single   | CS   | <b>0.3424</b> |
| Direct champion + LLM Social Focus hard-champion | Weighted | CS   | 0.3307        |
| Direct champion                                  | Soft     | 0.27 | 0.3403        |

Table S88: Transformer ensembles for moral value detection within *Personal Focus* using the best Personal Focus gate models (Validation). Best Macro- $F_1$  is bolded (ties included).

| Configuration                                   | Ensemble | Thr  | Macro- $F_1$  |
|-------------------------------------------------|----------|------|---------------|
| Model: Lex-LIWC@0.50. Gate: Baseline@0.17       | Single   | 0.50 | 0.2805        |
| Model: Lex-LIWC@0.50. Gate: Baseline@0.17       | Single   | 0.55 | 0.2810        |
| Model: Lex-Schwartz@0.50. Gate: Baseline@0.21   | Single   | 0.50 | 0.2829        |
| Model: Lex-Schwartz@0.50. Gate: Baseline@0.21   | Single   | 0.55 | <b>0.2840</b> |
| Model: Lex-WorryWords@0.50. Gate: Baseline@0.21 | Single   | 0.50 | 0.2798        |
| Model: Lex-WorryWords@0.50. Gate: Baseline@0.21 | Single   | 0.55 | 0.2810        |
| Model: NER@0.50. Gate: Baseline@0.19            | Single   | 0.50 | 0.2772        |
| Model: NER@0.50. Gate: Baseline@0.19            | Single   | 0.55 | 0.2783        |
| Model: TD-BERTopic@0.50. Gate: Baseline@0.22    | Single   | 0.50 | 0.2809        |
| Model: TD-BERTopic@0.50. Gate: Baseline@0.22    | Single   | 0.55 | 0.2830        |
| Model: TD-NMF@0.50. Gate: Baseline@0.20         | Single   | 0.50 | 0.2781        |
| Model: TD-NMF@0.50. Gate: Baseline@0.20         | Single   | 0.45 | 0.2784        |

Table S89: Transformer ensembles of the best Personal Focus transformer ensembles (Personal Focus (all), Validation). Best Macro- $F_1$  is bolded (ties included).

| Configuration                                           | Ensemble | Thr  | Macro- $F_1$  |
|---------------------------------------------------------|----------|------|---------------|
| Model: Lex-Schwartz@0.50. Gate: Single<br>Baseline@0.21 |          | 0.50 | 0.2829        |
| Model: Lex-Schwartz@0.50. Gate: Single<br>Baseline@0.21 |          | 0.45 | 0.2840        |
| Model: Lex-Schwartz@0.50. Gate: Soft<br>Baseline@0.21   |          | 0.53 | <b>0.2852</b> |

Table S90: Transformer ensembles across architectures (Values-Personal Focus-All architectures, Validation). Best Macro- $F_1$  is bolded (ties included).

| Configuration                                                                      | Ensemble | Thr  | Macro- $F_1$  |
|------------------------------------------------------------------------------------|----------|------|---------------|
| Model: Lex-Schwartz@0.50. Gate: Single<br>Baseline@0.21                            |          | 0.50 | 0.2829        |
| Model: Lex-Schwartz@0.50. Gate: Hard (2 models)<br>Baseline@0.21 + Direct champion |          | 0.50 | 0.2970        |
| Model: Lex-Schwartz@0.50. Gate: Weighted<br>Baseline@0.21 + Presence champion      |          | 0.50 | 0.2984        |
| Model: Lex-Schwartz@0.50. Gate: Soft<br>Baseline@0.21 + Presence champion          |          | 0.50 | 0.2980        |
| Direct champion                                                                    | Single   | CS   | 0.3085        |
| Direct champion                                                                    | Soft     | 0.29 | <b>0.3090</b> |

Table S91: Transformer ensembles across architectures (Values-Personal Focus-All architectures, Test). Best Macro- $F_1$  is bolded (ties included).

| Configuration   | Ensemble | Thr  | Macro- $F_1$  |
|-----------------|----------|------|---------------|
| Direct champion | Single   | 0.50 | 0.2723        |
| Direct champion | Single   | CS   | 0.3160        |
| Direct champion | Soft     | 0.29 | <b>0.3168</b> |



Table S92: LLM ensembles for Personal Focus (Validation). The LLM is `google-gemma-2-9b-it`. Best Macro- $F_1$  is bolded (ties included).

| Configuration                                  | Ensemble           | Thr  | Macro- $F_1$  |
|------------------------------------------------|--------------------|------|---------------|
| Gemma2 QLoRA hier (SBERT gate: Personal Focus) | Hard/Soft/Weighted | 0.50 | <b>0.2413</b> |

Table S93: Transformer + LLM ensembles for Personal Focus (Validation). Best Macro- $F_1$  is bolded (ties included).

| Configuration                                                    | Ensemble      | Thr  | Macro- $F_1$  |
|------------------------------------------------------------------|---------------|------|---------------|
| Direct champion + Gemma2 QLoRA hier (SBERT gate: Personal Focus) | Hard          | 0.50 | 0.3141        |
| Direct champion                                                  | Weighted/Soft | 0.50 | 0.2778        |
| Direct champion + Gemma2 QLoRA hier (SBERT gate: Personal Focus) | Hard          | 0.15 | <b>0.3230</b> |
| Direct champion + Gemma2 QLoRA hier (SBERT gate: Personal Focus) | Soft          | 0.15 | <b>0.3230</b> |

Table S94: Transformer + LLM ensembles for Personal Focus (Test). Best Macro- $F_1$  is bolded (ties included).

| Configuration                                                    | Ensemble | Thr  | Macro- $F_1$  |
|------------------------------------------------------------------|----------|------|---------------|
| Direct champion + Gemma2 QLoRA hier (SBERT gate: Personal Focus) | Hard     | 0.50 | 0.3008        |
| Direct champion + Gemma2 QLoRA hier (SBERT gate: Personal Focus) | Hard     | 0.15 | <b>0.3259</b> |
| Direct champion + Gemma2 QLoRA hier (SBERT gate: Personal Focus) | Soft     | 0.15 | <b>0.3259</b> |

Table S95: Transformer ensembles for moral value detection within *Openness* using the best Openness gate models (Validation). Best Macro- $F_1$  is bolded (ties included).

| Configuration                                                                                 | Ensemble | Thr  | Macro- $F_1$  |
|-----------------------------------------------------------------------------------------------|----------|------|---------------|
| Model: Lex- Single (hard/soft/weighted)<br>LIWC22+LingFeat@0.50.<br>Gate: NER@0.50            |          | 0.50 | 0.2354        |
| Model: Lex-<br>LIWC22+LingFeat@0.50.<br>Gate: NER@0.50                                        | Hard     | 0.50 | <b>0.2366</b> |
| Model: Lex-<br>LIWC22+LingFeat@0.50.<br>Gate: NER@0.50                                        | Soft     | 0.52 | 0.2358        |
| Model: Lex- Single (hard/soft/weighted)<br>LIWC22+LingFeat@0.82.<br>Gate: NER+TD-<br>LDA@0.50 |          | 0.50 | 0.2118        |
| Model: Lex-<br>LIWC22+LingFeat@0.82.<br>Gate: NER@0.25                                        | Hard     | 0.25 | 0.2179        |
| Model: Lex-<br>LIWC22+LingFeat@0.82.<br>Gate: NER+TD-<br>LDA@0.50                             | Soft     | 0.14 | 0.2211        |

Table S96: Transformer ensembles of the best Openness transformer ensembles (Openness (all), Validation). Best Macro- $F_1$  is bolded (ties included).

| Configuration                                                                                 | Ensemble | Thr  | Macro- $F_1$  |
|-----------------------------------------------------------------------------------------------|----------|------|---------------|
| Model: Lex- Single<br>LIWC22+LingFeat@0.50.<br>Gate: NER@0.50                                 |          | 0.50 | 0.2354        |
| Model: Lex-<br>LIWC22+LingFeat@0.50.<br>Gate: NER@0.50                                        | Hard     | 0.25 | 0.2366        |
| Model: Lex- Soft (2 models)<br>LIWC22+LingFeat@0.50 + Lex-<br>LIWC22+LingFeat@0.82. Gate: NER |          | 0.32 | <b>0.2418</b> |

Table S97: Transformer ensembles across architectures (Values–Openness–All architectures, Validation). Best Macro- $F_1$  is bolded (ties included).

| Configuration                       | Ensemble                    | Thr  | Macro- $F_1$  |
|-------------------------------------|-----------------------------|------|---------------|
| Direct champion                     | Single (hard/soft/weighted) | 0.50 | 0.2294        |
| Direct champion + Presence champion | Hard (2 models)             | 0.50 | 0.2515        |
| Presence champion                   | Single                      | CS   | 0.2607        |
| Presence champion                   | Soft                        | 0.28 | <b>0.2618</b> |

Table S98: Transformer ensembles across architectures (Values–Openness–All architectures, Test). Best Macro- $F_1$  is bolded (ties included).

| Configuration     | Ensemble | Thr  | Macro- $F_1$  |
|-------------------|----------|------|---------------|
| Presence champion | Single   | 0.50 | 0.2061        |
| Presence champion | Single   | CS   | 0.2390        |
| Presence champion | Soft     | 0.28 | <b>0.2413</b> |

Table S99: LLM ensembles for Openness (Validation). The LLM is google-gemma-2-9b-it. Best Macro- $F_1$  is bolded (ties included).

| Configuration                                      | Ensemble           | Thr  | Macro- $F_1$  |
|----------------------------------------------------|--------------------|------|---------------|
| Gemma2 QLoRA hier (SBERT gate: Openness to Change) | Hard/Soft/Weighted | 0.50 | <b>0.1754</b> |

Table S100: Transformer + LLM ensembles for Openness (Validation). Best Macro- $F_1$  is bolded (ties included).

| Configuration                                                          | Ensemble      | Thr  | Macro- $F_1$  |
|------------------------------------------------------------------------|---------------|------|---------------|
| Presence champion                                                      | Hard          | 0.50 | 0.2586        |
| Presence champion                                                      | Weighted/Soft | 0.50 | 0.2266        |
| Presence champion + Gemma2 QLoRA hier (SBERT gate: Openness to Change) | Hard          | 0.17 | 0.2736        |
| Presence champion + Gemma2 QLoRA hier (SBERT gate: Openness to Change) | Soft          | 0.17 | <b>0.2771</b> |

Table S101: Transformer + LLM ensembles for Openness (Test). Best Macro- $F_1$  is bolded (ties included).

| Configuration                                                             | Ensemble | Thr  | Macro- $F_1$  |
|---------------------------------------------------------------------------|----------|------|---------------|
| Presence champion + Gemma2 QLoRA<br>hier (SBERT gate: Openness to Change) | Hard     | 0.50 | 0.2299        |
| Presence champion + Gemma2 QLoRA<br>hier (SBERT gate: Openness to Change) | Hard     | 0.17 | 0.2474        |
| Presence champion + Gemma2 QLoRA<br>hier (SBERT gate: Openness to Change) | Soft     | 0.17 | <b>0.2486</b> |

*S6.2. Self-Protection*

*S6.3. Social Focus*

*S6.4. Personal Focus*

*S6.5. Openness To Change*

*S6.6. Conservation*

*S6.7. Self-Transcendence*

*S6.8. Self-Enhancement*

Table S102: Transformer ensembles for moral value detection within *Conservation* using the best Conservation gate models (Validation). Best Macro- $F_1$  is bolded (ties included).

| Configuration                                           | Ensemble                    | Thr  | Macro- $F_1$  |
|---------------------------------------------------------|-----------------------------|------|---------------|
| Model: Baseline@0.50.<br>Gate: Lex-MJD@0.50             | Single (hard/soft/weighted) | 0.50 | 0.2794        |
| Model: Baseline@0.50.<br>Gate: Baseline@0.50            | Hard                        | 0.30 | 0.2830        |
| Model: Baseline@0.50.<br>Gate: NER@0.50                 | Soft                        | 0.17 | 0.2795        |
| Model: Lex-LIWC22+LingFeat@0.10.<br>Gate: TD-LDA@0.50   | Single (hard/soft/weighted) | 0.50 | 0.3053        |
| Model: Lex-LIWC22+LingFeat@0.10.<br>Gate: Baseline@0.40 | Hard                        | 0.40 | <b>0.3058</b> |
| Model: Lex-LIWC22+LingFeat@0.10.<br>Gate: TD-LDA@0.50   | Soft                        | 0.54 | 0.3029        |
| Model: Lex-LIWC22+LingFeat@0.50.<br>Gate: NER@0.50      | Single (hard/soft/weighted) | 0.50 | 0.2885        |
| Model: Lex-LIWC22+LingFeat@0.50.<br>Gate: TD-LDA@0.30   | Hard                        | 0.30 | 0.2917        |
| Model: Lex-LIWC22+LingFeat@0.50.<br>Gate: NER@0.50      | Soft                        | 0.17 | 0.2865        |

Table S103: Transformer ensembles of the best Conservation transformer ensembles (Conservation (all), Validation). Best Macro- $F_1$  is bolded (ties included).

| Configuration                                           | Ensemble | Thr  | Macro- $F_1$  |
|---------------------------------------------------------|----------|------|---------------|
| Model: Lex-LIWC22+LingFeat@0.10.<br>Gate: Baseline@0.50 | Single   | 0.50 | 0.2964        |
| Model: Lex-LIWC22+LingFeat@0.10.<br>Gate: Baseline@0.50 | Hard     | 0.30 | <b>0.3058</b> |
| Model: Lex-LIWC22+LingFeat@0.10.<br>Gate: Baseline@0.50 | Soft     | 0.28 | 0.2973        |

Table S104: Transformer ensembles across architectures (Values–Conservation–All architectures, Validation). Best Macro- $F_1$  is bolded (ties included).

| Configuration   | Ensemble                    | Thr  | Macro- $F_1$  |
|-----------------|-----------------------------|------|---------------|
| Direct champion | Single (hard/soft/weighted) | 0.50 | 0.3043        |
| Direct champion | Hard                        | 0.30 | <b>0.3262</b> |
| Direct champion | Soft                        | 0.35 | 0.3226        |

Table S105: Transformer ensembles across architectures (Values–Conservation–All architectures, Test). Best Macro- $F_1$  is bolded (ties included).

| Configuration   | Ensemble                    | Thr  | Macro- $F_1$  |
|-----------------|-----------------------------|------|---------------|
| Direct champion | Single (hard/soft/weighted) | 0.50 | 0.2896        |
| Direct champion | Hard                        | 0.30 | 0.3129        |
| Direct champion | Soft                        | 0.15 | <b>0.3129</b> |

Table S106: LLM ensembles for Conservation (Validation). The LLM is `google-gemma-2-9b-it`. Best Macro- $F_1$  is bolded (ties included).

| Configuration                                | Ensemble           | Thr  | Macro- $F_1$  |
|----------------------------------------------|--------------------|------|---------------|
| Gemma2 QLoRA hier (SBERT gate: Conservation) | Hard/Soft/Weighted | 0.50 | <b>0.2885</b> |

Table S107: Transformer + LLM ensembles for Conservation (Validation). Best Macro- $F_1$  is bolded (ties included).

| Configuration                                                  | Ensemble | Thr  | Macro- $F_1$  |
|----------------------------------------------------------------|----------|------|---------------|
| Direct champion + Gemma2 QLoRA hier (SBERT gate: Conservation) | Hard     | 0.50 | 0.3447        |
| Direct champion + Gemma2 QLoRA hier (SBERT gate: Conservation) | Hard     | 0.15 | <b>0.3465</b> |
| Direct champion + Gemma2 QLoRA hier (SBERT gate: Conservation) | Soft     | 0.15 | <b>0.3465</b> |

Table S108: Transformer + LLM ensembles for Conservation (Test). Best Macro- $F_1$  is bolded (ties included).

| Configuration                                                     | Ensemble | Thr  | Macro- $F_1$  |
|-------------------------------------------------------------------|----------|------|---------------|
| Direct champion + Gemma2 QLoRA hier<br>(SBERT gate: Conservation) | Hard     | 0.50 | 0.3297        |
| Direct champion + Gemma2 QLoRA hier<br>(SBERT gate: Conservation) | Hard     | 0.15 | <b>0.3339</b> |
| Direct champion + Gemma2 QLoRA hier<br>(SBERT gate: Conservation) | Soft     | 0.15 | <b>0.3339</b> |

Table S109: Transformer ensembles for moral value detection within *Self-Transcendence* using the best Self-Transcendence gate models (Validation). Best Macro- $F_1$  is bolded (ties included).

| Configuration                                                       | Ensemble                    | Thr  | Macro- $F_1$  |
|---------------------------------------------------------------------|-----------------------------|------|---------------|
| Model: Baseline. Gate: Single (hard/soft/weighted)<br>Baseline@0.50 |                             | 0.50 | 0.2661        |
| Model: Baseline. Gate: Lex-Schwartz@0.50                            | Hard                        | 0.15 | 0.2789        |
| Model: Lex-MFD-20. Gate: Lex-Schwartz@0.50                          | Single (hard/soft/weighted) | 0.50 | 0.2732        |
| Model: Lex-MFD-20. Gate: Lex-MFD@0.50                               | Hard                        | 0.25 | 0.2816        |
| Model: Lex-MFD-20. Gate: Lex-MFD@0.21                               | Single (hard/soft/weighted) | 0.50 | 0.2909        |
| Model: Lex-MFD-20. Gate: Lex-MFD@0.21                               | Single (hard/soft/weighted) | 0.65 | 0.2909        |
| Model: WorryWords. Gate: Lex-MFD@0.16                               | Single (hard/soft/weighted) | 0.50 | <b>0.2988</b> |
| Model: TD-BERTopic. Gate: Lex-MFD@0.19                              | Single (hard/soft/weighted) | 0.50 | 0.2958        |

Table S110: Transformer ensembles of the best Self-Transcendence transformer ensembles (Self-Transcendence (all), Validation). Best Macro- $F_1$  is bolded (ties included).

| Configuration                                                                                  | Ensemble                    | Thr  | Macro- $F_1$  |
|------------------------------------------------------------------------------------------------|-----------------------------|------|---------------|
| Model: Lex-<br>WorryWords. Gate:<br>Lex-MFD@0.16                                               | Single (hard/soft/weighted) | 0.50 | 0.2988        |
| Model: Lex-<br>WorryWords. Gate:<br>Lex-MFD@0.16 +<br>Model: Lex-MFD-20.<br>Gate: Lex-MFD@0.50 | Soft                        | 0.29 | <b>0.3005</b> |

Table S111: Transformer ensembles across architectures (Values-Self-Transcendence-All architectures, Validation). Best Macro- $F_1$  is bolded (ties included).

| Configuration                                         | Ensemble                    | Thr  | Macro- $F_1$  |
|-------------------------------------------------------|-----------------------------|------|---------------|
| Self-Transcendence<br>champion                        | Single (hard/soft/weighted) | 0.50 | 0.2700        |
| Self-Transcendence<br>champion + Presence<br>champion | Hard                        | 0.50 | 0.2976        |
| Self-Transcendence<br>champion                        | Hard                        | 0.29 | <b>0.3005</b> |
| Direct champion                                       | Soft                        | 0.27 | 0.2998        |

Table S112: Transformer ensembles across architectures (Values-Self-Transcendence-All architectures, Test). Best Macro- $F_1$  is bolded (ties included).

| Configuration                  | Ensemble                    | Thr  | Macro- $F_1$  |
|--------------------------------|-----------------------------|------|---------------|
| Self-Transcendence<br>champion | Single (hard/soft/weighted) | 0.50 | 0.2586        |
| Self-Transcendence<br>champion | Hard                        | 0.29 | <b>0.3194</b> |
| Self-Transcendence<br>champion | Soft                        | 0.29 | <b>0.3194</b> |



Table S113: LLM ensembles for Self-Transcendence (Validation). The LLM is google-gemma-2-9b-it. Best Macro- $F_1$  is bolded (ties included).

| Configuration                                                                                                                           | Ensemble  | Thr  | Macro- $F_1$  |
|-----------------------------------------------------------------------------------------------------------------------------------------|-----------|------|---------------|
| Gemma2 zero-shot + Gemma2 few-shot ( $k=7$ ) hier (SBERT gate: Self-Transcendence) + Gemma2 QLoRA hier (SBERT gate: Self-Transcendence) | Hard/Soft | 0.50 | <b>0.2377</b> |
| Gemma2 few-shot ( $k=7$ ) hier (SBERT gate: Self-Transcendence)                                                                         | Weighted  | 0.50 | 0.2162        |

Table S114: LLM ensembles for Self-Transcendence (Test). Best Macro- $F_1$  is bolded (ties included).

| Configuration                                                                                                                           | Ensemble           | Thr  | Macro- $F_1$  |
|-----------------------------------------------------------------------------------------------------------------------------------------|--------------------|------|---------------|
| Gemma2 zero-shot + Gemma2 few-shot ( $k=7$ ) hier (SBERT gate: Self-Transcendence) + Gemma2 QLoRA hier (SBERT gate: Self-Transcendence) | Hard/Soft/Weighted | 0.50 | <b>0.2201</b> |

Table S115: Transformer + LLM ensembles for Self-Transcendence (Validation). Best Macro- $F_1$  is bolded (ties included).

| Configuration               | Ensemble                    | Thr  | Macro- $F_1$  |
|-----------------------------|-----------------------------|------|---------------|
| Self-Transcendence champion | Single (hard/soft/weighted) | 0.50 | 0.2700        |
| Self-Transcendence champion | Hard                        | 0.29 | <b>0.3005</b> |
| Self-Transcendence champion | Soft                        | 0.57 | 0.2664        |

Table S116: Transformer ensembles for moral value detection within *Self-Enhancement* using the best Self-Enhancement gate models (Validation). Best Macro- $F_1$  is bolded (ties included).

| Configuration                                         | Ensemble                    | Thr  | Macro- $F_1$  |
|-------------------------------------------------------|-----------------------------|------|---------------|
| Model: Lex-MFD-<br>20. Gate: Lex-<br>Schwartz@0.50    | Single (hard/soft/weighted) | 0.50 | 0.2980        |
| Model: Lex-MFD-<br>20. Gate: Lex-<br>Schwartz@0.50    | Hard                        | 0.25 | 0.3011        |
| Model: Lex-MFD-<br>20. Gate: Lex-<br>Schwartz@0.24    | Single (hard/soft/weighted) | 0.50 | 0.3154        |
| Model: Lex-MFD-<br>20. Gate: Lex-<br>Schwartz@0.24    | Hard                        | 0.55 | 0.3169        |
| Model: Lex-<br>WorryWords. Gate:<br>Lex-Schwartz@0.23 | Single (hard/soft/weighted) | 0.50 | 0.3169        |
| Model: Lex-<br>WorryWords. Gate:<br>Lex-Schwartz@0.23 | Hard                        | 0.60 | <b>0.3189</b> |
| Model: TD-<br>BERTopic. Gate:<br>Lex-Schwartz@0.50    | Single (hard/soft/weighted) | 0.50 | 0.3012        |
| Model: TD-<br>BERTopic. Gate:<br>Lex-Schwartz@0.50    | Hard                        | 0.30 | 0.3042        |
| Model: TD-<br>BERTopic. Gate:<br>Lex-Schwartz@0.29    | Single (hard/soft/weighted) | 0.50 | 0.3156        |
| Model: TD-<br>BERTopic. Gate:<br>Lex-Schwartz@0.29    | Hard                        | 0.55 | 0.3165        |

Table S117: Transformer ensembles of the best Self-Enhancement transformer ensembles (Self-Enhancement (all), Validation). Best Macro- $F_1$  is bolded (ties included).

| Configuration                                  | Ensemble                    | Thr  | Macro- $F_1$  |
|------------------------------------------------|-----------------------------|------|---------------|
| Model: Lex–WorryWords. Gate: Lex–Schwartz@0.23 | Single (hard/soft/weighted) | 0.50 | 0.3169        |
| Model: Lex–WorryWords. Gate: Lex–Schwartz@0.23 | Hard                        | 0.55 | <b>0.3189</b> |

Table S118: Transformer ensembles across architectures (Values–Self-Enhancement–All architectures, Validation). Best Macro- $F_1$  is bolded (ties included).

| Configuration                                                    | Ensemble      | Thr  | Macro- $F_1$  |
|------------------------------------------------------------------|---------------|------|---------------|
| Model: Lex–WorryWords. Gate: Lex–Schwartz@0.23                   | Single (hard) | 0.50 | 0.3169        |
| Model: Lex–WorryWords. Gate: Lex–Schwartz@0.23 + Direct champion | Weighted      | 0.50 | 0.3272        |
| Model: Lex–WorryWords. Gate: Lex–Schwartz@0.23 + Direct champion | Soft          | 0.50 | 0.3311        |
| Presence champion                                                | Hard          | —    | 0.3434        |
| Presence champion                                                | Soft          | 0.29 | <b>0.3438</b> |

Table S119: Transformer ensembles across architectures (Values–Self-Enhancement–All architectures, Test). Best Macro- $F_1$  is bolded (ties included).

| Configuration     | Ensemble                    | Thr  | Macro- $F_1$  |
|-------------------|-----------------------------|------|---------------|
| Presence champion | Single (hard/soft/weighted) | 0.50 | 0.3030        |
| Presence champion | Hard                        | 0.55 | 0.3362        |
| Presence champion | Soft                        | 0.29 | <b>0.3373</b> |

Table S120: LLM ensembles for Self-Enhancement (Validation). The LLM is `google-gemma-2-9b-it`. Best Macro- $F_1$  is bolded (ties included).

| Configuration                                    | Ensemble           | Thr  | Macro- $F_1$  |
|--------------------------------------------------|--------------------|------|---------------|
| Gemma2 QLoRA hier (SBERT gate: Self-Enhancement) | Hard/Soft/Weighted | 0.50 | <b>0.2809</b> |

Table S121: Transformer + LLM ensembles for Self-Enhancement (Validation). Best Macro- $F_1$  is bolded (ties included).

| Configuration                                                        | Ensemble      | Thr  | Macro- $F_1$  |
|----------------------------------------------------------------------|---------------|------|---------------|
| Presence champion + Gemma2 QLoRA hier (SBERT gate: Self-Enhancement) | Hard          | 0.50 | 0.3516        |
| Presence champion + Gemma2 QLoRA hier (SBERT gate: Self-Enhancement) | Hard          | 0.17 | 0.3604        |
| Presence champion + Gemma2 QLoRA hier (SBERT gate: Self-Enhancement) | Soft          | 0.17 | <b>0.3664</b> |
| Presence champion                                                    | Weighted/Soft | 0.50 | 0.3068        |

Table S122: Transformer + LLM ensembles for Self-Enhancement (Test). Best Macro- $F_1$  is bolded (ties included).

| Configuration                                                        | Ensemble | Thr  | Macro- $F_1$  |
|----------------------------------------------------------------------|----------|------|---------------|
| Presence champion + Gemma2 QLoRA hier (SBERT gate: Self-Enhancement) | Hard     | 0.50 | 0.3383        |
| Presence champion + Gemma2 QLoRA hier (SBERT gate: Self-Enhancement) | Hard     | 0.17 | <b>0.3487</b> |
| Presence champion + Gemma2 QLoRA hier (SBERT gate: Self-Enhancement) | Soft     | 0.17 | 0.3480        |
| Presence champion + Gemma2 QLoRA hier (SBERT gate: Self-Enhancement) | Weighted | 0.50 | 0.2757        |
| Presence champion + Gemma2 QLoRA hier (SBERT gate: Self-Enhancement) | Soft     | 0.50 | 0.2267        |

## S7. Statistical significance tests

All paired model comparisons use a nonparametric bootstrap over instances to estimate a one-sided lower 95% confidence bound for  $\Delta\text{Macro-}F_1$  and a one-sided  $p$ -value for the hypothesis  $\Delta > 0$ . For per-label analysis on positive instances, we apply McNemar’s exact test with Benjamini–Hochberg FDR control ( $\alpha = 0.05$ ). We fix the number of bootstrap resamples to  $B=2000$  and report the lower bound and one-sided  $p$  for key comparisons.

For transparency, we summarise the main significance comparisons in tabular form. Each comparison table reports the test Macro- $F_1$  scores of the two systems, the bootstrap estimate for  $\Delta\text{Macro-}F_1$  (Model2–Model1) via its one-sided lower 95% confidence bound, and the corresponding one-sided  $p$ -value. Per-label McNemar analyses are presented separately, listing only those labels whose differences remain significant after Benjamini–Hochberg correction.

*S7.1. Growth*

*S7.2. Self-Protection*

*S7.3. Social Focus*

*S7.4. Personal Focus*

*S7.5. Openness To Change*

*S7.6. Conservation*

*S7.7. Self-Transcendence*

*S7.8. Self-Enhancement*

Table S123: Growth: system registry (test split). Each system is assigned an ID to avoid repeating long configuration strings in the comparison table. Best Macro- $F_1$  for Growth is shown in bold. Values are reported with 5 decimals to avoid artificial ties.

| ID  | System (configuration)                                                               | Macro- $F_1$   |
|-----|--------------------------------------------------------------------------------------|----------------|
| T1  | Transformer / Direct: Baseline (thr=0.50)                                            | 0.25057        |
| T2  | Transformer / Direct: 2 prev sent w/ label (thr=0.50)                                | 0.25160        |
| T3  | Transformer / Direct: Baseline (thr=0.30)                                            | 0.28646        |
| T4  | Transformer / Direct: 2 prev sent w/ label (thr=0.15)                                | 0.29269        |
| P1  | Transformer / Presence: Baseline (thr=0.50), filter=Lex-LIWC-22_LingFeat (thr=0.10)  | 0.26856        |
| P2  | Transformer / Presence: Lex - MJD (thr=0.50), filter=Lex-LIWC-22_LingFeat (thr=0.10) | 0.27606        |
| P3  | Transformer / Presence: Baseline (thr=0.50), filter=Lex-LIWC-22_LingFeat (thr=0.50)  | 0.25992        |
| P4  | Transformer / Presence: Baseline (thr=0.25), filter=Lex-LIWC-22_LingFeat (thr=0.50)  | 0.28391        |
| P5  | Transformer / Presence: Lex - MJD (thr=0.20), filter=Lex-LIWC-22_LingFeat (thr=0.50) | 0.28440        |
| G1  | Transformer / Growth: Baseline (thr=0.50), filter=Baseline (thr=0.18)                | 0.26926        |
| G2  | Transformer / Growth: Baseline (thr=0.50), filter=Baseline (thr=0.50)                | 0.26289        |
| G3  | Transformer / Growth: Baseline (thr=0.30), filter=Baseline (thr=0.50)                | 0.27071        |
| ETr | Transformer / Ensemble (Transformers): champions ensemble (soft voting; thr=0.29)    | <b>0.30283</b> |
| L1  | LLM / Growth: Gemma 2 9B Zero-Shot                                                   | 0.18264        |
| L2  | LLM / Growth: Gemma 2 9B Zero-Shot + SBERT gate (filter-thr=0.36)                    | 0.19218        |
| L3  | LLM / Growth: Gemma 2 9B Few-Shot                                                    | 0.19094        |
| L4  | LLM / Growth: Gemma 2 9B Few-Shot + SBERT gate (filter-thr=0.29)                     | 0.19351        |
| L5  | LLM / Growth: Gemma 2 9B QLoRA + SBERT gate (filter-thr=0.00)                        | 0.13155        |
| ELL | LLM / Growth: ensemble (hard voting; fixed thr=0.50; test)                           | 0.20128        |

Table S124: Growth: paired statistical comparisons on the **test** split. Each row compares Model1 vs. Model2 (by ID from Table S123), reporting their test Macro- $F_1$ , the one-sided lower 95% bootstrap confidence bound for  $\Delta$  Macro- $F_1$  (Model2 – Model1), and the one-sided  $p$ -value for  $\Delta > 0$ . Values are reported with 5 decimals to avoid artificial ties.

| Comparison                                        | Model1 ID | Macro- $F_1$ (M1) | Model2 ID | Macro- $F_1$ (M2) | $\Delta$ Macro- $F_1$ LB <sub>0.95</sub> | $p$ / Sig.    |
|---------------------------------------------------|-----------|-------------------|-----------|-------------------|------------------------------------------|---------------|
| Model (Direct)                                    | T1        | 0.25057           | T2        | 0.25160           | -0.10800                                 | 0.43500 / No  |
| Tuning threshold (Direct)                         | T1        | 0.25057           | T3        | 0.28646           | 0.02520                                  | 0 / Yes       |
| Tuning threshold + Model (Direct)                 | T3        | 0.28646           | T4        | 0.29269           | 0.00900                                  | 0.23750 / No  |
| Model (Presence)                                  | P1        | 0.26856           | P2        | 0.27606           | -0.00090                                 | 0.07100 / No  |
| Tuning threshold (Presence)                       | P3        | 0.25992           | P4        | 0.28391           | 0.01350                                  | 0 / Yes       |
| Tuning threshold + Model (Presence)               | P4        | 0.28391           | P5        | 0.28440           | -0.00670                                 | 0.45400 / No  |
| Tuning threshold (Growth)                         | G2        | 0.26289           | G3        | 0.27071           | 0.00090                                  | 0.02850 / Yes |
| Architecture champion (Presence vs Direct)        | P4        | 0.28391           | T3        | 0.28646           | -0.00650                                 | 0.31850 / No  |
| Architecture champion (Growth vs Direct)          | G3        | 0.27071           | T3        | 0.28646           | 0.00300                                  | 0.02050 / Yes |
| Single vs Ensemble Transformer champions          | T3        | 0.28646           | ETr       | <b>0.30283</b>    | 0.00160                                  | 0.03850 / Yes |
| Adding SBERT gate (LLM)                           | L1        | 0.18264           | L2        | 0.19218           | 0.00140                                  | 0.03100 / Yes |
| Zero-shot vs Few-shot (LLM)                       | L1        | 0.18264           | L3        | 0.19094           | 0.00050                                  | 0.04500 / Yes |
| Adding SBERT gate (LLM, few-shot)                 | L3        | 0.19094           | L4        | 0.19351           | -0.00420                                 | 0.27350 / No  |
| Finetuning with QLoRA vs best zero/few-shot (LLM) | L2        | 0.19218           | L5        | 0.13155           | -0.07710                                 | 1.00000 / No  |
| Single vs Ensemble LLM                            | L2        | 0.19218           | ELL       | 0.20128           | 0.00250                                  | 0.01450 / Yes |
| Transformer vs LLM champions                      | ELL       | 0.20128           | ETr       | <b>0.30283</b>    | 0.08400                                  | 0 / Yes       |

Table S125: Growth: per-label McNemar exact tests on positives. We list only labels with McNemar  $p \leq 0.05$  after Benjamini–Hochberg FDR control ( $\alpha = 0.05$ ) for the corresponding comparison (Model2 vs. Model1). Abbreviations are used for label names. Model IDs refer to Table S123.

| Comparison                                        | Model1 ID | Model2 ID | Significant labels (McNemar $p$ )                                                                                                                                                |
|---------------------------------------------------|-----------|-----------|----------------------------------------------------------------------------------------------------------------------------------------------------------------------------------|
| Tuning threshold (Direct)                         | T1        | T3        | <b>SD-t</b> ( $p=0.0024$ ), <b>SD-a</b> ( $p=0$ ), <b>Stim</b> ( $p=0$ ), <b>Hed</b> ( $p=0.0172$ ), <b>Uni-c</b> ( $p=0$ ), <b>Uni-n</b> ( $p=0$ ), <b>Uni-t</b> ( $p=0.0002$ ) |
| Tuning threshold (Presence)                       | P3        | P4        | <b>SD-t</b> ( $p=0$ ), <b>SD-a</b> ( $p=0$ ), <b>Stim</b> ( $p=0$ )                                                                                                              |
| Tuning threshold (Growth)                         | G2        | G3        | <b>SD-a</b> ( $p=0.0061$ ), <b>Stim</b> ( $p=0.0002$ ), <b>Conf-i</b> ( $p=0.0036$ ), <b>Uni-t</b> ( $p=0$ ), <b>Ben-d</b> ( $p=0.0011$ )                                        |
| Architecture champion (Growth vs Direct)          | G3        | T3        | <b>Pow-d</b> ( $p=0.0004$ )                                                                                                                                                      |
| Single vs Ensemble Transformer champions          | T3        | ETr       | <b>SD-a</b> ( $p=0.0001$ ), <b>Conf-i</b> ( $p=0.0222$ )                                                                                                                         |
| Adding SBERT gate (LLM)                           | L1        | L2        | <b>SD-t</b> ( $p=0.0003$ ), <b>SD-a</b> ( $p=0$ ), <b>Stim</b> ( $p=0$ ), <b>Hed</b> ( $p=0$ ), <b>Uni-t</b> ( $p=0.0021$ )                                                      |
| Finetuning with QLoRA vs best zero/few-shot (LLM) | L2        | L5        | <b>SD-t</b> ( $p=0.0003$ ), <b>Stim</b> ( $p=0.0109$ ), <b>Hed</b> ( $p=0.0235$ ), <b>Uni-t</b> ( $p=0.0008$ )                                                                   |
| Single vs Ensemble LLM                            | L2        | ELL       | <b>SD-a</b> ( $p=0$ ), <b>Stim</b> ( $p=0.0010$ )                                                                                                                                |
| Transformer vs LLM champions                      | ELL       | ETr       | <b>SD-a</b> ( $p=0.0011$ ), <b>Stim</b> ( $p=0$ ), <b>Hed</b> ( $p=0$ ), <b>Uni-t</b> ( $p=0.0001$ ), <b>Uni-n</b> ( $p=0.0004$ )                                                |



Table S126: Self-Protection: system registry (test split). Each system is assigned an ID to avoid repeating long configuration strings in the comparison table. Best Macro- $F_1$  for Self-Protection is shown in bold. Values are reported with 5 decimals to avoid artificial ties.

| ID    | System (configuration)                                                                           | Macro- $F_1$   |
|-------|--------------------------------------------------------------------------------------------------|----------------|
| T1    | Transformer / Direct: Baseline (thr=0.50)                                                        | 0.29206        |
| T2    | Transformer / Direct: Lex - LIWC 22 (thr=0.50)                                                   | 0.29793        |
| T3    | Transformer / Direct: Baseline (thr=0.30)                                                        | 0.32074        |
| T4    | Transformer / Direct: Lex - LIWC 22 (thr=0.25)                                                   | 0.33089        |
| P1    | Transformer / Presence: Baseline (thr=0.50), filter=Previous-Sentences-2-Lex-LIWC-22 (thr=0.10)  | 0.29631        |
| P2    | Transformer / Presence: Lex - MJD (thr=0.50), filter=Previous-Sentences-2-Lex-LIWC-22 (thr=0.10) | 0.30967        |
| P3    | Transformer / Presence: Baseline (thr=0.30), filter=Previous-Sentences-2-Lex-LIWC-22 (thr=0.10)  | 0.30479        |
| P4    | Transformer / Presence: Lex - MJD (thr=0.40), filter=Previous-Sentences-2-Lex-LIWC-22 (thr=0.10) | 0.32443        |
| S1    | Transformer / Self-Protection: Baseline (thr=0.50), filter=Baseline (thr=0.10)                   | 0.29875        |
| S2    | Transformer / Self-Protection: Baseline (thr=0.50), filter=Baseline (thr=0.50)                   | 0.29354        |
| S3    | Transformer / Self-Protection: Baseline (thr=0.15), filter=Baseline (thr=0.50)                   | 0.30622        |
| ETr   | Transformer / Ensemble (Transformers): champions ensemble (soft voting; thr=0.29)                | 0.34160        |
| L1    | LLM / Self-Protection: Gemma 2 9B Zero-Shot                                                      | 0.20393        |
| L2    | LLM / Self-Protection: Gemma 2 9B Zero-Shot + SBERT gate (filter-thr=0.28)                       | 0.20915        |
| L3    | LLM / Self-Protection: Gemma 2 9B Few-Shot                                                       | 0.21974        |
| L4    | LLM / Self-Protection: Gemma 2 9B Few-Shot + SBERT gate (filter-thr=0.36)                        | 0.21163        |
| L5    | LLM / Self-Protection: Gemma 2 9B QLoRA + SBERT gate (filter-thr=0.00)                           | 0.25411        |
| EBoth | Ensemble (Transformers+LLMs): hard voting; tuned threshold (test)                                | <b>0.35263</b> |

Table S127: Self-Protection: paired statistical comparisons on the **test** split. Each row compares Model1 vs. Model2 (by ID from Table S126), reporting their test Macro- $F_1$ , the one-sided lower 95% bootstrap confidence bound for  $\Delta$  Macro- $F_1$  (Model2 – Model1), and the one-sided  $p$ -value for  $\Delta > 0$ . Best Macro- $F_1$  is shown in bold. Values are reported with 5 decimals to avoid artificial ties.

| Comparison                                        | Model1 ID | Macro- $F_1$ (M1) | Model2 ID | Macro- $F_1$ (M2) | $\Delta$ Macro- $F_1$ LB <sub>0.95</sub> | $p$ / Sig.    |
|---------------------------------------------------|-----------|-------------------|-----------|-------------------|------------------------------------------|---------------|
| Model (Direct)                                    | T1        | 0.29206           | T2        | 0.29793           | -0.00240                                 | 0.11200 / No  |
| Tuning threshold (Direct)                         | T1        | 0.29206           | T3        | 0.32074           | 0.01770                                  | 0 / Yes       |
| Tuning threshold + Model (Direct)                 | T3        | 0.32074           | T4        | 0.33089           | -0.00550                                 | 0.14050 / No  |
| Model (Presence)                                  | P1        | 0.29631           | P2        | 0.30967           | 0.00550                                  | 0.00600 / Yes |
| Tuning threshold (Presence)                       | P1        | 0.29631           | P3        | 0.30479           | 0.00330                                  | 0.00300 / Yes |
| Tuning threshold + Model (Presence)               | P3        | 0.30479           | P4        | 0.32443           | 0.00840                                  | 0.00050 / Yes |
| Tuning threshold (Self-Protection)                | S2        | 0.29354           | S3        | 0.30622           | 0.00280                                  | 0.01250 / Yes |
| Architecture champion (Presence vs Direct)        | T3        | 0.32074           | P4        | 0.32443           | -0.00510                                 | 0.24700 / No  |
| Architecture champion (Self-Protection vs Direct) | S3        | 0.30622           | T3        | 0.32074           | 0.00190                                  | 0.02850 / Yes |
| Single vs Ensemble Transformer champions          | T3        | 0.32074           | ETr       | 0.34160           | 0.00580                                  | 0.00800 / Yes |
| Adding SBERT gate (LLM)                           | L1        | 0.20393           | L2        | 0.20915           | -0.00450                                 | 0.16850 / No  |
| Zero-shot vs Few-shot (LLM)                       | L1        | 0.20393           | L3        | 0.21974           | 0.00840                                  | 0.00050 / Yes |
| Adding SBERT gate (LLM, few-shot)                 | L3        | 0.21974           | L4        | 0.21163           | -0.01620                                 | 0.96850 / No  |
| Finetuning with QLoRA vs best zero/few-shot (LLM) | L3        | 0.21974           | L5        | 0.25411           | 0.01790                                  | 0 / Yes       |
| Transformer vs LLM champions                      | L5        | 0.25411           | ETr       | 0.34160           | 0.07570                                  | 0 / Yes       |
| Best (Transformer/LLM) vs Ensemble (both)         | ETr       | 0.34160           | EBoth     | <b>0.35263</b>    | 0.00700                                  | 0 / Yes       |

Table S128: Self-Protection: per-label McNemar exact tests on positives. We list only labels with McNemar  $p \leq 0.05$  after Benjamini–Hochberg FDR control ( $\alpha = 0.05$ ) for the corresponding comparison (Model2 vs. Model1). Abbreviations are used for label names. Model IDs refer to Table S126.

| Comparison                                        | Model1 ID | Model2 ID | Significant labels (McNemar $p$ )                                                                                                                                                         |
|---------------------------------------------------|-----------|-----------|-------------------------------------------------------------------------------------------------------------------------------------------------------------------------------------------|
| Tuning threshold (Direct)                         | T1        | T3        | <b>Face</b> (p=0), <b>Sec-per</b> (p=0), <b>Sec-soc</b> (p=0), <b>Trad</b> (p=0), <b>Conf-r</b> (p=0), <b>Conf-i</b> (p=0), <b>Hum</b> (p=0.0001), <b>Ben-c</b> (p=0), <b>Ben-d</b> (p=0) |
| Model (Presence)                                  | P1        | P2        | <b>Ach</b> (p=0)                                                                                                                                                                          |
| Tuning threshold (Presence)                       | P1        | P3        | <b>Ach</b> (p=0), <b>Pow-d</b> (p=0), <b>Pow-r</b> (p=0), <b>Face</b> (p=0), <b>Sec-per</b> (p=0), <b>Sec-soc</b> (p=0), <b>Trad</b> (p=0), <b>Conf-r</b> (p=0), <b>Conf-i</b> (p=0.0312) |
| Tuning threshold + Model (Presence)               | P3        | P4        | <b>Ach</b> (p=0.0116), <b>Pow-r</b> (p=0.0152), <b>Sec-per</b> (p=0.0288), <b>Sec-soc</b> (p=0)                                                                                           |
| Tuning threshold (Self-Protection)                | S2        | S3        | <b>Ach</b> (p=0), <b>Pow-d</b> (p=0), <b>Pow-r</b> (p=0), <b>Face</b> (p=0), <b>Sec-per</b> (p=0), <b>Sec-soc</b> (p=0), <b>Trad</b> (p=0.0043), <b>Conf-r</b> (p=0), <b>Conf-i</b> (p=0) |
| Architecture champion (Self-Protection vs Direct) | S3        | T3        | <b>Face</b> (p=0.0001), <b>Sec-soc</b> (p=0), <b>Conf-r</b> (p=0.0089), <b>Conf-i</b> (p=0.0065)                                                                                          |
| Single vs Ensemble Transformer champions          | T3        | ETr       | <b>Sec-per</b> (p=0), <b>Sec-soc</b> (p=0.0122), <b>Trad</b> (p=0.0082), <b>Conf-r</b> (p=0.0021), <b>Conf-i</b> (p=0.0001), <b>Hum</b> (p=0.0274), <b>Ben-c</b> (p=0.0003)               |
| Zero-shot vs Few-shot (LLM)                       | L1        | L3        | <b>Sec-per</b> (p=0), <b>Sec-soc</b> (p=0.0014), <b>Trad</b> (p=0), <b>Conf-r</b> (p=0), <b>Conf-i</b> (p=0.0002), <b>Hum</b> (p=0.0065), <b>Ben-d</b> (p=0), <b>Uni-c</b> (p=0)          |
| Finetuning with QLoRA vs best zero/few-shot (LLM) | L3        | L5        | <b>Ach</b> (p=0), <b>Pow-d</b> (p=0.0005), <b>Pow-r</b> (p=0), <b>Sec-per</b> (p=0), <b>Sec-soc</b> (p=0), <b>Trad</b> (p=0), <b>Conf-r</b> (p=0), <b>Conf-i</b> (p=0)                    |
| Transformer vs LLM champions                      | L5        | ETr       | <b>Face</b> (p=0), <b>Sec-per</b> (p=0), <b>Sec-soc</b> (p=0), <b>Trad</b> (p=0), <b>Conf-r</b> (p=0), <b>Conf-i</b> (p=0), <b>Hum</b> (p=0), <b>Ben-c</b> (p=0), <b>Ben-d</b> (p=0)      |
| Best (Transformer/LLM) vs Ensemble (both)         | ETr       | EBoth     | <b>Sec-per</b> (p=0.0463), <b>Trad</b> (p=0), <b>Conf-r</b> (p=0.0114), <b>Hum</b> (p=0), <b>Ben-c</b> (p=0.0022), <b>Ben-d</b> (p=0)                                                     |

Table S129: Social Focus: system registry (test split). Each system is assigned an ID to avoid repeating long configuration strings in the comparison table. Best Macro- $F_1$  for Social Focus is shown in bold. Values are reported with 5 decimals to avoid artificial ties.

| ID  | System (configuration)                                                                          | Macro- $F_1$   |
|-----|-------------------------------------------------------------------------------------------------|----------------|
| T1  | Transformer / Direct: Baseline (thr=0.50)                                                       | 0.29378        |
| T2  | Transformer / Direct: Lex - LIWC 22 (thr=0.50)                                                  | 0.29606        |
| T3  | Transformer / Direct: Baseline (thr=0.30)                                                       | 0.32989        |
| T4  | Transformer / Direct: Lex - LIWC 22 (thr=0.25)                                                  | 0.33491        |
| P1  | Transformer / Presence: Baseline (thr=0.50), filter=Previous-Sentences-2-Lex-EmoLex (thr=0.10)  | 0.30305        |
| P2  | Transformer / Presence: Lex - VAD (thr=0.50), filter=Previous-Sentences-2-Lex-EmoLex (thr=0.10) | 0.32031        |
| P3  | Transformer / Presence: Baseline (thr=0.50), filter=Lex-LIWC-22_LingFeat (thr=0.50)             | 0.30161        |
| P4  | Transformer / Presence: Baseline (thr=0.25), filter=Lex-LIWC-22_LingFeat (thr=0.50)             | 0.32627        |
| P5  | Transformer / Presence: Lex - WorryWords (thr=0.25), filter=Lex-LIWC-22_LingFeat (thr=0.50)     | 0.33214        |
| S1  | Transformer / Social Focus: Baseline (thr=0.50), filter=Lex - WorryWords (thr=0.10)             | 0.30982        |
| S2  | Transformer / Social Focus: TD - LDA (thr=0.50), filter=Lex - WorryWords (thr=0.10)             | 0.31689        |
| S3  | Transformer / Social Focus: Baseline (thr=0.50), filter=TD - NMF (thr=0.50)                     | 0.30904        |
| S4  | Transformer / Social Focus: Baseline (thr=0.25), filter=TD - NMF (thr=0.50)                     | 0.31830        |
| S5  | Transformer / Social Focus: Lex - MJD (thr=0.25), filter=TD - NMF (thr=0.50)                    | 0.32561        |
| ETr | Transformer / Ensemble (Transformers): champions ensemble (soft voting; thr=0.29)               | <b>0.34545</b> |
| L1  | LLM / Social Focus: Gemma 2 9B Zero-Shot                                                        | 0.19270        |
| L2  | LLM / Social Focus: Gemma 2 9B Zero-Shot + SBERT gate (filter-thr=0.38)                         | 0.20476        |
| L3  | LLM / Social Focus: Gemma 2 9B Few-Shot                                                         | 0.23030        |
| L4  | LLM / Social Focus: Gemma 2 9B Few-Shot + SBERT gate (filter-thr=0.38)                          | 0.23411        |
| L5  | LLM / Social Focus: Gemma 2 9B QLoRA + SBERT gate (filter-thr=0.00)                             | 0.20579        |
| ELL | LLM / Social Focus: ensemble (hard voting; fixed thr=0.50; test)                                | 0.26690        |

Table S130: Social Focus: paired statistical comparisons on the **test** split. Each row compares Model1 vs. Model2 (by ID from Table S129), reporting their test Macro- $F_1$ , the one-sided lower 95% bootstrap confidence bound for  $\Delta$  Macro- $F_1$  (Model2-Model1), and the one-sided  $p$ -value for  $\Delta > 0$ . Values are reported with 5 decimals to avoid artificial ties.

| Comparison                                        | Model1 ID | Macro- $F_1$ (M1) | Model2 ID | Macro- $F_1$ (M2) | $\Delta$ Macro- $F_1$ LB <sub>0.95</sub> | $p$ / Sig.    |
|---------------------------------------------------|-----------|-------------------|-----------|-------------------|------------------------------------------|---------------|
| Model (Direct)                                    | T1        | 0.29378           | T2        | 0.29606           | -0.00750                                 | 0.34550 / No  |
| Tuning threshold (Direct)                         | T1        | 0.29378           | T3        | 0.32989           | 0.02480                                  | 0 / Yes       |
| Tuning threshold + Model (Direct)                 | T3        | 0.32989           | T4        | 0.33491           | -0.01120                                 | 0.29700 / No  |
| Model (Presence)                                  | P1        | 0.30305           | P2        | 0.32031           | 0.00790                                  | 0 / Yes       |
| Tuning threshold (Presence)                       | P3        | 0.30161           | P4        | 0.32627           | 0.01300                                  | 0 / Yes       |
| Tuning threshold + Model (Presence)               | P4        | 0.32627           | P5        | 0.33214           | -0.00190                                 | 0.10050 / No  |
| Model (Social Focus)                              | S1        | 0.30982           | S2        | 0.31689           | -0.00060                                 | 0.06800 / No  |
| Tuning threshold (Social Focus)                   | S3        | 0.30904           | S4        | 0.31830           | 0.00350                                  | 0.00450 / Yes |
| Tuning threshold + Model (Social Focus)           | S4        | 0.31830           | S5        | 0.32561           | -0.00300                                 | 0.05850 / No  |
| Architecture champion (Presence vs Direct)        | P4        | 0.32627           | T3        | 0.32989           | -0.00520                                 | 0.23850 / No  |
| Architecture champion (Social Focus vs Direct)    | S4        | 0.31830           | T3        | 0.32989           | -0.00200                                 | 0.07500 / No  |
| Single vs Ensemble Transformer champions          | T3        | 0.32989           | ETr       | <b>0.34545</b>    | -0.00080                                 | 0.05850 / No  |
| Adding SBERT gate (LLM)                           | L1        | 0.19270           | L2        | 0.20476           | 0.00370                                  | 0.01450 / Yes |
| Zero-shot vs Few-shot (LLM)                       | L1        | 0.19270           | L3        | 0.23030           | 0.02690                                  | 0 / Yes       |
| Adding SBERT gate (LLM, few-shot)                 | L3        | 0.23030           | L4        | 0.23411           | -0.00180                                 | 0.13750 / No  |
| Finetuning with QLoRA vs best zero/few-shot (LLM) | L3        | 0.23030           | L5        | 0.20579           | -0.04170                                 | 0.98900 / No  |
| Single vs Ensemble LLM                            | L3        | 0.23030           | ELL       | 0.26690           | 0.02690                                  | 0 / Yes       |
| Transformer vs LLM champions                      | ELL       | 0.26690           | T3        | 0.32989           | 0.04480                                  | 0 / Yes       |

Table S131: Social Focus: per-label McNemar exact tests on positives. We list only labels with McNemar  $p \leq 0.05$  after Benjamini–Hochberg FDR control ( $\alpha = 0.05$ ) for the corresponding comparison (Model2 vs. Model1). Abbreviations are used for label names. Model IDs refer to Table S129.

| Comparison                      | Model1 ID | Model2 ID | Significant labels (McNemar $p$ )                                                                                                                                                                                                     |
|---------------------------------|-----------|-----------|---------------------------------------------------------------------------------------------------------------------------------------------------------------------------------------------------------------------------------------|
| Tuning threshold (Direct)       | T1        | T3        | <b>Face</b> (p=0), <b>Sec-per</b> (p=0.0001), <b>Sec-soc</b> (p=0), <b>Trad</b> (p=0), <b>Conf-r</b> (p=0), <b>Hum</b> (p=0), <b>Ben-c</b> (p=0), <b>Ben-d</b> (p=0), <b>Uni-c</b> (p=0), <b>Uni-n</b> (p=0), <b>Uni-t</b> (p=0.0001) |
| Model (Presence)                | P1        | P2        | <b>Uni-c</b> (p=0.0032)                                                                                                                                                                                                               |
| Tuning threshold (Presence)     | P3        | P4        | <b>Sec-soc</b> (p=0), <b>Trad</b> (p=0), <b>Conf-r</b> (p=0), <b>Conf-i</b> (p=0.0043), <b>Ben-c</b> (p=0), <b>Ben-d</b> (p=0), <b>Uni-c</b> (p=0), <b>Uni-n</b> (p=0), <b>Uni-t</b> (p=0)                                            |
| Tuning threshold (Social Focus) | S3        | S4        | <b>Sec-soc</b> (p=0), <b>Trad</b> (p=0.0100), <b>Conf-r</b> (p=0), <b>Ben-c</b> (p=0), <b>Ben-d</b> (p=0), <b>Uni-c</b> (p=0), <b>Uni-t</b> (p=0.0007)                                                                                |
| Adding SBERT gate (LLM)         | L1        | L2        | <b>Trad</b> (p=0), <b>Conf-r</b> (p=0), <b>Conf-i</b> (p=0), <b>Ben-c</b> (p=0), <b>Uni-c</b> (p=0), <b>Uni-n</b> (p=0)                                                                                                               |
| Zero-shot vs Few-shot (LLM)     | L1        | L3        | <b>Sec-soc</b> (p=0), <b>Trad</b> (p=0.0010), <b>Conf-r</b> (p=0), <b>Conf-i</b> (p=0.0010), <b>Uni-c</b> (p=0), <b>Uni-n</b> (p=0)                                                                                                   |
| Single vs Ensemble LLM          | L3        | ELL       | <b>Trad</b> (p=0.0151), <b>Conf-r</b> (p=0), <b>Conf-i</b> (p=0), <b>Ben-c</b> (p=0.0001), <b>Ben-d</b> (p=0), <b>Uni-n</b> (p=0)                                                                                                     |
| Transformer vs LLM champions    | ELL       | T3        | <b>Conf-i</b> (p=0.0421), <b>Ben-c</b> (p=0.0024), <b>Ben-d</b> (p=0.0001), <b>Uni-c</b> (p=0)                                                                                                                                        |

Table S132: Personal Focus: system registry (test split). Each system is assigned an ID to avoid repeating long configuration strings in the comparison table. Best Macro- $F_1$  for Personal Focus is shown in bold. Values are reported with 5 decimals to avoid artificial ties.

| ID    | System (configuration)                                                                           | Macro- $F_1$   |
|-------|--------------------------------------------------------------------------------------------------|----------------|
| T1    | Transformer / Direct: Baseline (thr=0.50)                                                        | 0.26705        |
| T2    | Transformer / Direct: Lex - LIWC 22 (thr=0.50)                                                   | 0.27467        |
| T3    | Transformer / Direct: Baseline (thr=0.30)                                                        | 0.29104        |
| T4    | Transformer / Direct: TD - BERTopic (thr=0.20)                                                   | 0.30534        |
| P1    | Transformer / Presence: Baseline (thr=0.50), filter=Lex-LIWC-22_LingFeat (thr=0.10)              | 0.27987        |
| P2    | Transformer / Presence: Lex - MJD (thr=0.50), filter=Lex-LIWC-22_LingFeat (thr=0.10)             | 0.28750        |
| P3    | Transformer / Presence: Baseline (thr=0.50), filter=Previous-Sentences-2-Lex-LIWC-22 (thr=0.10)  | 0.28186        |
| P4    | Transformer / Presence: Lex - MJD (thr=0.50), filter=Previous-Sentences-2-Lex-LIWC-22 (thr=0.10) | 0.29010        |
| P5    | Transformer / Presence: Baseline (thr=0.30), filter=Previous-Sentences-2-Lex-LIWC-22 (thr=0.10)  | 0.28948        |
| P6    | Transformer / Presence: Lex - MJD (thr=0.40), filter=Previous-Sentences-2-Lex-LIWC-22 (thr=0.10) | 0.29624        |
| PF1   | Transformer / Personal Focus: Baseline (thr=0.50), filter=NER (thr=0.19)                         | 0.28422        |
| PF2   | Transformer / Personal Focus: Baseline (thr=0.55), filter=NER (thr=0.19)                         | 0.28359        |
| ETr   | Transformer / Ensemble (Transformers): champions ensemble (soft voting; thr=0.29)                | 0.31677        |
| L1    | LLM / Personal Focus: Gemma 2 9B Zero-Shot                                                       | 0.18699        |
| L2    | LLM / Personal Focus: Gemma 2 9B Zero-Shot + SBERT gate (filter-thr=0.25)                        | 0.17881        |
| L3    | LLM / Personal Focus: Gemma 2 9B Few-Shot                                                        | 0.19781        |
| L4    | LLM / Personal Focus: Gemma 2 9B Few-Shot + SBERT gate (filter-thr=0.29)                         | 0.19528        |
| L5    | LLM / Personal Focus: Gemma 2 9B QLoRA + SBERT gate (filter-thr=0.00)                            | 0.18405        |
| EBoth | Ensemble (Transformer+LLM): tuned hard voting (test)                                             | <b>0.32592</b> |

Table S133: Personal Focus: paired statistical comparisons on the **test** split. Each row compares Model1 vs. Model2 (by ID from Table S132), reporting their test Macro- $F_1$ , the one-sided lower 95% bootstrap confidence bound for  $\Delta$  Macro- $F_1$  (Model2-Model1), and the one-sided  $p$ -value for  $\Delta > 0$ . Best Macro- $F_1$  for Personal Focus is shown in bold. Values are reported with 5 decimals to avoid artificial ties.

| Comparison                                        | Model1 ID | Macro- $F_1$ (M1) | Model2 ID | Macro- $F_1$ (M2) | $\Delta$ Macro- $F_1$ LB <sub>0.95</sub> | $p$ / Sig.    |
|---------------------------------------------------|-----------|-------------------|-----------|-------------------|------------------------------------------|---------------|
| Model (Direct)                                    | T1        | 0.26705           | T2        | 0.27467           | -0.00310                                 | 0.11550 / No  |
| Tuning threshold (Direct)                         | T1        | 0.26705           | T3        | 0.29104           | 0.01600                                  | 0 / Yes       |
| Tuning threshold + Model (Direct)                 | T3        | 0.29104           | T4        | 0.30534           | 0.00510                                  | 0.00400 / Yes |
| Model (Presence, Lex-LIWC-22_LingFeat gate)       | P1        | 0.27987           | P2        | 0.28750           | -0.00070                                 | 0.07050 / No  |
| Model (Presence, PrevSent2+Lex-LIWC-22 gate)      | P3        | 0.28186           | P4        | 0.29010           | -0.00050                                 | 0.06150 / No  |
| Tuning threshold (Presence)                       | P3        | 0.28186           | P5        | 0.28948           | 0.00140                                  | 0.02550 / Yes |
| Tuning threshold + Model (Presence)               | P5        | 0.28948           | P6        | 0.29624           | -0.00200                                 | 0.10550 / No  |
| Tuning threshold (Personal Focus)                 | PF1       | 0.28422           | PF2       | 0.28359           | -0.00390                                 | 0.62900 / No  |
| Architecture champion (Presence vs Direct)        | P5        | 0.28948           | T4        | 0.30534           | 0.00660                                  | 0.00400 / Yes |
| Architecture champion (Personal Focus vs Direct)  | PF1       | 0.28422           | T4        | 0.30534           | 0.01060                                  | 0.00150 / Yes |
| Single vs Ensemble Transformer champions          | T4        | 0.30534           | ETr       | 0.31677           | 0.00290                                  | 0.01600 / Yes |
| Adding SBERT gate (LLM)                           | L1        | 0.18699           | L2        | 0.17881           | -0.01670                                 | 0.94250 / No  |
| Zero-shot vs Few-shot (LLM)                       | L1        | 0.18699           | L3        | 0.19781           | 0.00370                                  | 0.00750 / Yes |
| Adding SBERT gate (LLM, few-shot)                 | L3        | 0.19781           | L4        | 0.19528           | -0.01010                                 | 0.72000 / No  |
| Finetuning with QLoRA vs best zero/few-shot (LLM) | L3        | 0.19781           | L5        | 0.18405           | -0.02800                                 | 0.94250 / No  |
| Transformer vs LLM champions                      | L3        | 0.19781           | ETr       | 0.31677           | 0.10710                                  | 0 / Yes       |
| Transformer vs LLM winner vs Ensemble of both     | ETr       | 0.31677           | EBoth     | <b>0.32592</b>    | 0.00510                                  | 0.00100 / Yes |



Table S134: Personal Focus: per-label McNemar exact tests on positives. We list only labels with McNemar  $p \leq 0.05$  after Benjamini–Hochberg FDR control ( $\alpha = 0.05$ ) for the corresponding comparison (Model2 vs. Model1). Abbreviations are used for label names. Model IDs refer to Table S132.

| Comparison                                       | Model1 ID | Model2 ID | Significant labels (McNemar $p$ )                                                                                                      |
|--------------------------------------------------|-----------|-----------|----------------------------------------------------------------------------------------------------------------------------------------|
| Tuning threshold (Direct)                        | T1        | T3        | <b>SD-t</b> (p=0.0022), <b>SD-a</b> (p=0), <b>Stim</b> (p=0), <b>Hed</b> (p=0.0156)                                                    |
| Tuning threshold + Model (Direct)                | T3        | T4        | <b>SD-t</b> (p=0.0058), <b>SD-a</b> (p=0), <b>Stim</b> (p=0), <b>Face</b> (p=0.0058)                                                   |
| Tuning threshold (Presence)                      | P3        | P5        | <b>SD-t</b> (p=0.0005), <b>SD-a</b> (p=0), <b>Stim</b> (p=0)                                                                           |
| Architecture champion (Presence vs Direct)       | P5        | T4        | <b>SD-t</b> (p=0), <b>SD-a</b> (p=0.0186), <b>Stim</b> (p=0.0009), <b>Face</b> (p=0.0009), <b>Pow-d</b> (p=0.0046)                     |
| Architecture champion (Personal Focus vs Direct) | PF1       | T4        | <b>Ach</b> (p=0.0012), <b>Pow-d</b> (p=0), <b>Pow-r</b> (p=0)                                                                          |
| Single vs Ensemble Transformer champions         | T4        | ETr       | <b>SD-t</b> (p=0.0009), <b>SD-a</b> (p=0.0006), <b>Stim</b> (p=0.0006), <b>Pow-d</b> (p=0), <b>Pow-r</b> (p=0), <b>Face</b> (p=0.0242) |
| Zero-shot vs Few-shot (LLM)                      | L1        | L3        | <b>SD-t</b> (p=0.0009), <b>SD-a</b> (p=0.0021), <b>Hed</b> (p=0)                                                                       |
| Transformer vs LLM champions                     | L3        | ETr       | <b>SD-t</b> (p=0.0001), <b>Stim</b> (p=0), <b>Hed</b> (p=0.0001), <b>Ach</b> (p=0.0462), <b>Pow-d</b> (p=0.0003)                       |
| Transformer vs LLM winner vs Ensemble of both    | ETr       | EBoth     | <b>Face</b> (p=0.0286)                                                                                                                 |

Table S135: Openness: system registry (test split). Each system is assigned an ID to avoid repeating long configuration strings in the comparison table. Best Macro- $F_1$  for Openness is shown in bold. Values are reported with 5 decimals to avoid artificial ties.

| ID    | System (configuration)                                                                               | Macro- $F_1$   |
|-------|------------------------------------------------------------------------------------------------------|----------------|
| T1    | Transformer / Direct: Baseline (thr=0.50)                                                            | 0.22424        |
| T2    | Transformer / Direct: TD - BERTopic (thr=0.50)                                                       | 0.23236        |
| T3    | Transformer / Direct: Baseline (thr=0.30)                                                            | 0.23985        |
| T4    | Transformer / Direct: 2 prev sent w/ label (thr=0.15)                                                | <b>0.25077</b> |
| P1    | Transformer / Presence: Baseline (thr=0.50), filter=Previous-Sentences-2-Lex-LIWC-22 (thr=0.10)      | 0.23117        |
| P2    | Transformer / Presence: Lex - LIWC 22 (thr=0.50), filter=Previous-Sentences-2-Lex-LIWC-22 (thr=0.10) | 0.23255        |
| P3    | Transformer / Presence: Baseline (thr=0.50), filter=Lex-LIWC-22_LingFeat (thr=0.10)                  | 0.23230        |
| P4    | Transformer / Presence: Baseline (thr=0.30), filter=Lex-LIWC-22_LingFeat (thr=0.10)                  | 0.24159        |
| P5    | Transformer / Presence: Baseline (thr=0.30), filter=Previous-Sentences-2-Lex-LIWC-22 (thr=0.10)      | 0.23809        |
| O1    | Transformer / Openness: Baseline (thr=0.50), filter=Lex - LIWC 22 + Ling Feat (thr=0.50)             | 0.22277        |
| O2    | Transformer / Openness: NER + TD - LDA (thr=0.50), filter=Lex - LIWC 22 + Ling Feat (thr=0.50)       | 0.23493        |
| ETr   | Transformer / Ensemble (Transformers): champions ensemble (soft voting; thr=0.28)                    | 0.24132        |
| L1    | LLM / Openness: Gemma 2 9B Zero-Shot                                                                 | 0.07849        |
| L2    | LLM / Openness: Gemma 2 9B Zero-Shot + SBERT gate (filter-thr=0.39)                                  | 0.09018        |
| L3    | LLM / Openness: Gemma 2 9B Few-Shot                                                                  | 0.09263        |
| L4    | LLM / Openness: Gemma 2 9B Few-Shot + SBERT gate (filter-thr=0.58)                                   | 0.11255        |
| L5    | LLM / Openness: Gemma 2 9B QLoRA + SBERT gate (filter-thr=0.00)                                      | 0.12274        |
| EBoth | Ensemble (Transformer+LLM): tuned soft voting (thr=0.17; test)                                       | 0.24860        |

Table S136: Openness: paired statistical comparisons on the **test** split. Each row compares Model1 vs. Model2 (by ID from Table S135), reporting their test Macro- $F_1$ , the one-sided lower 95% bootstrap confidence bound for  $\Delta$  Macro- $F_1$  (Model2-Model1), and the one-sided  $p$ -value for  $\Delta > 0$ . Best Macro- $F_1$  for Openness is shown in bold. Values are reported with 5 decimals to avoid artificial ties.

| Comparison                                              | Model1 ID | Macro- $F_1$ (M1) | Model2 ID | Macro- $F_1$ (M2) | $\Delta$ Macro- $F_1$ LB <sub>0.95</sub> | $p$ / Sig.    |
|---------------------------------------------------------|-----------|-------------------|-----------|-------------------|------------------------------------------|---------------|
| Model (Direct)                                          | T1        | 0.22424           | T2        | 0.23236           | -0.01110                                 | 0.26250 / No  |
| Tuning threshold (Direct)                               | T1        | 0.22424           | T3        | 0.23985           | 0.00260                                  | 0.02550 / Yes |
| Tuning threshold + Model (Direct)                       | T3        | 0.23985           | T4        | <b>0.25077</b>    | -0.00660                                 | 0.13900 / No  |
| Model (Presence, PrevSent2+Lex-LIWC-22 gate)            | P1        | 0.23117           | P2        | 0.23255           | -0.01500                                 | 0.45650 / No  |
| Tuning threshold (Presence, Lex-LIWC-22_LingFeat gate)  | P3        | 0.23230           | P4        | 0.24159           | -0.00200                                 | 0.09650 / No  |
| Tuning threshold (Presence, PrevSent2+Lex-LIWC-22 gate) | P1        | 0.23117           | P5        | 0.23809           | -0.00400                                 | 0.15650 / No  |
| Model (Openness gate)                                   | O1        | 0.22277           | O2        | 0.23493           | -0.00190                                 | 0.07500 / No  |
| Architecture champion (Presence vs Direct)              | P3        | 0.23230           | T3        | 0.23985           | -0.00940                                 | 0.23500 / No  |
| Architecture champion (Openness vs Direct)              | O1        | 0.22277           | T3        | 0.23985           | -0.00260                                 | 0.07850 / No  |
| Single vs Ensemble Transformer champions                | T3        | 0.23985           | ETr       | 0.24132           | -0.01570                                 | 0.44650 / No  |
| Adding SBERT gate (LLM)                                 | L1        | 0.07849           | L2        | 0.09018           | 0.00410                                  | 0.00400 / Yes |
| Zero-shot vs Few-shot (LLM)                             | L1        | 0.07849           | L3        | 0.09263           | 0.00850                                  | 0 / Yes       |
| Adding SBERT gate (LLM, few-shot)                       | L3        | 0.09263           | L4        | 0.11255           | 0.01290                                  | 0 / Yes       |
| Finetuning with QLoRA vs best zero/few-shot (LLM)       | L4        | 0.11255           | L5        | 0.12274           | -0.01210                                 | 0.23500 / No  |
| Transformer vs LLM champions                            | L4        | 0.11255           | T3        | 0.23985           | 0.10690                                  | 0 / Yes       |
| Transformer vs LLM winner vs Ensemble of both           | T3        | 0.23985           | EBoth     | 0.24860           | -0.01020                                 | 0.21150 / No  |

Table S137: Openness: per-label McNemar exact tests on positives. We list only labels with McNemar  $p \leq 0.05$  after Benjamini–Hochberg FDR control ( $\alpha = 0.05$ ) for the corresponding comparison (Model2 vs. Model1). Abbreviations are used for label names. Model IDs refer to Table S135.

| Comparison                |       |          |    | Model1 ID | Model2 ID | Significant labels (McNemar $p$ )                                                                   |
|---------------------------|-------|----------|----|-----------|-----------|-----------------------------------------------------------------------------------------------------|
| Tuning threshold (Direct) |       | (Di-     | T1 |           | T3        | <b>SD-t</b> ( $p=0.0026$ ), <b>SD-a</b> ( $p=0$ ), <b>Stim</b> ( $p=0$ ), <b>Hed</b> ( $p=0.0156$ ) |
| Adding (LLM)              | SBERT | gate     | L1 |           | L2        | <b>SD-t</b> ( $p=0$ ), <b>SD-a</b> ( $p=0$ ), <b>Stim</b> ( $p=0$ ), <b>Hed</b> ( $p=0$ )           |
| Zero-shot (LLM)           | vs    | Few-shot | L1 |           | L3        | <b>SD-t</b> ( $p=0$ ), <b>SD-a</b> ( $p=0$ ), <b>Hed</b> ( $p=0.0046$ )                             |
| Adding (LLM, few-shot)    | SBERT | gate     | L3 |           | L4        | <b>SD-t</b> ( $p=0$ ), <b>SD-a</b> ( $p=0$ ), <b>Stim</b> ( $p=0$ ), <b>Hed</b> ( $p=0$ )           |
| Transformer champions     | vs    | LLM      | L4 |           | T3        | <b>SD-t</b> ( $p=0.0005$ ), <b>SD-a</b> ( $p=0$ ), <b>Stim</b> ( $p=0$ )                            |

Table S138: Conservation: system registry (test split). Each system is assigned an ID to avoid repeating long configuration strings in the comparison table. Best Macro- $F_1$  for Conservation is shown in bold. Values are reported with 5 decimals to avoid artificial ties.

| ID    | System (configuration)                                                                             | Macro- $F_1$   |
|-------|----------------------------------------------------------------------------------------------------|----------------|
| T1    | Transformer / Direct: Baseline (thr=0.50)                                                          | 0.27655        |
| T2    | Transformer / Direct: Lex – LIWC 22 (thr=0.50)                                                     | 0.28341        |
| T3    | Transformer / Direct: Baseline (thr=0.30)                                                          | 0.30057        |
| T4    | Transformer / Direct: Lex – LIWC 22 (thr=0.25)                                                     | 0.31141        |
| P1    | Transformer / Presence: Baseline (thr=0.50), filter=Previous-Sentences-2 + Lex-LIWC-22 (thr=0.10)  | 0.27588        |
| P2    | Transformer / Presence: Lex – MJD (thr=0.50), filter=Previous-Sentences-2 + Lex-LIWC-22 (thr=0.10) | 0.29033        |
| P3    | Transformer / Presence: Baseline (thr=0.25), filter=Lex-LIWC-22_LingFeat (thr=0.50)                | 0.29995        |
| P4    | Transformer / Presence: Lex – VAD (thr=0.25), filter=Lex-LIWC-22_LingFeat (thr=0.50)               | 0.30931        |
| C1    | Transformer / Conservation: Baseline (thr=0.50), filter=Lex-LIWC-22 + Ling Feat (thr=0.10)         | 0.29164        |
| C2    | Transformer / Conservation: Lex – Schwartz (thr=0.50), filter=Lex-LIWC-22 + Ling Feat (thr=0.10)   | 0.29719        |
| C3    | Transformer / Conservation: Baseline (thr=0.50), filter=Lex-LIWC-22 + Ling Feat (thr=0.50)         | 0.28545        |
| C4    | Transformer / Conservation: Baseline (thr=0.30), filter=Lex-LIWC-22 + Ling Feat (thr=0.50)         | 0.29607        |
| ETr   | Transformer / Ensemble (Transformers): champions ensemble (soft voting; thr=0.30; test)            | 0.31293        |
| L1    | LLM / Conservation: Gemma 2 9B Zero-Shot                                                           | 0.18232        |
| L2    | LLM / Conservation: Gemma 2 9B Zero-Shot + SBERT gate (filter-thr=0.45)                            | 0.20993        |
| L3    | LLM / Conservation: Gemma 2 9B Few-Shot                                                            | 0.22986        |
| L4    | LLM / Conservation: Gemma 2 9B Few-Shot + SBERT gate (filter-thr=0.39)                             | 0.22682        |
| L5    | LLM / Conservation: Gemma 2 9B QLoRA + SBERT gate (filter-thr=0.00)                                | 0.25787        |
| EBoth | Ensemble (Transformer+LLM): hard voting (tuned; test)                                              | <b>0.33393</b> |

Table S139: Conservation: paired statistical comparisons on the **test** split. Each row compares Model1 vs. Model2 (by ID from Table S138), reporting their test Macro- $F_1$ , the one-sided lower 95% bootstrap confidence bound for  $\Delta$  Macro- $F_1$  (Model2–Model1), and the one-sided  $p$ -value for  $\Delta > 0$ . Values are reported with 5 decimals to avoid artificial ties.

| Comparison                                        | Model1 ID | Macro- $F_1$ (M1) | Model2 ID | Macro- $F_1$ (M2) | $\Delta$ Macro- $F_1$ LB <sub>0.95</sub> | $p$ / Sig.    |
|---------------------------------------------------|-----------|-------------------|-----------|-------------------|------------------------------------------|---------------|
| Model (Direct)                                    | T1        | 0.27655           | T2        | 0.28341           | -0.00380                                 | 0.14200 / No  |
| Tuning threshold (Direct)                         | T1        | 0.27655           | T3        | 0.30057           | 0.00960                                  | 0 / Yes       |
| Tuning threshold + Model (Direct)                 | T3        | 0.30057           | T4        | 0.31141           | -0.01090                                 | 0.20950 / No  |
| Model (Presence)                                  | P1        | 0.27588           | P2        | 0.29033           | 0.00370                                  | 0.01100 / Yes |
| Tuning threshold + Model (Presence)               | P3        | 0.29995           | P4        | 0.30931           | -0.00010                                 | 0.05250 / No  |
| Model (Conservation)                              | C1        | 0.29164           | C2        | 0.29719           | -0.00520                                 | 0.22050 / No  |
| Tuning threshold (Conservation)                   | C3        | 0.28545           | C4        | 0.29607           | 0.00300                                  | 0.01000 / Yes |
| Architecture champion (Presence vs Direct)        | P3        | 0.29995           | T3        | 0.30057           | -0.01040                                 | 0.45800 / No  |
| Architecture champion (Conservation vs Direct)    | C4        | 0.29607           | T3        | 0.30057           | -0.00860                                 | 0.28250 / No  |
| Single vs Ensemble Transformer champions          | T3        | 0.30057           | ETr       | 0.31293           | -0.00580                                 | 0.12050 / No  |
| Adding SBERT gate (LLM)                           | L1        | 0.18232           | L2        | 0.20993           | 0.01710                                  | 0 / Yes       |
| Zero-shot vs Few-shot (LLM)                       | L1        | 0.18232           | L3        | 0.22986           | 0.03420                                  | 0 / Yes       |
| Adding SBERT gate (LLM, few-shot)                 | L3        | 0.22986           | L4        | 0.22682           | -0.01610                                 | 0.63700 / No  |
| Finetuning with QLoRA vs best zero/few-shot (LLM) | L3        | 0.22986           | L5        | 0.25787           | 0.00430                                  | 0.02800 / Yes |
| Transformer vs LLM champions                      | L5        | 0.25787           | T3        | 0.30057           | 0.01830                                  | 0.00300 / Yes |
| Transformer vs Ensemble (Transformer+LLM)         | T3        | 0.30057           | EBoth     | <b>0.33393</b>    | 0.01140                                  | 0.00850 / Yes |

Table S140: Conservation: per-label McNemar exact tests on positives. We list only labels with McNemar  $p \leq 0.05$  after Benjamini–Hochberg FDR control ( $\alpha = 0.05$ ) for the corresponding comparison (Model2 vs. Model1). Abbreviations are used for label names. Model IDs refer to Table S138.

| Comparison                                        | Model1 ID | Model2 ID | Significant labels (McNemar $p$ )                                                                                                    |
|---------------------------------------------------|-----------|-----------|--------------------------------------------------------------------------------------------------------------------------------------|
| Tuning threshold (Direct)                         | T1        | T3        | <b>Face</b> (p=0), <b>Sec-per</b> (p=0), <b>Sec-soc</b> (p=0), <b>Trad</b> (p=0.0001), <b>Conf-r</b> (p=0), <b>Conf-i</b> (p=0)      |
| Tuning threshold (Conservation)                   | C3        | C4        | <b>Face</b> (p=0.0002), <b>Sec-per</b> (p=0), <b>Sec-soc</b> (p=0), <b>Conf-r</b> (p=0), <b>Conf-i</b> (p=0.0023)                    |
| Adding SBERT gate (LLM)                           | L1        | L2        | <b>Face</b> (p=0), <b>Sec-per</b> (p=0), <b>Sec-soc</b> (p=0), <b>Trad</b> (p=0), <b>Conf-r</b> (p=0), <b>Conf-i</b> (p=0)           |
| Zero-shot vs Few-shot (LLM)                       | L1        | L3        | <b>Face</b> (p=0), <b>Sec-per</b> (p=0.0010), <b>Sec-soc</b> (p=0), <b>Conf-r</b> (p=0), <b>Conf-i</b> (p=0)                         |
| Finetuning with QLoRA vs best zero/few-shot (LLM) | L3        | L5        | <b>Sec-per</b> (p=0), <b>Sec-soc</b> (p=0), <b>Trad</b> (p=0), <b>Conf-r</b> (p=0), <b>Conf-i</b> (p=0)                              |
| Transformer vs LLM champions                      | L5        | T3        | <b>Face</b> (p=0.0342), <b>Sec-per</b> (p=0), <b>Sec-soc</b> (p=0), <b>Trad</b> (p=0.0003), <b>Conf-r</b> (p=0), <b>Conf-i</b> (p=0) |
| Transformer vs Ensemble (Transformer+LLM)         | T3        | EBoth     | <b>Face</b> (p=0), <b>Sec-per</b> (p=0.0007), <b>Sec-soc</b> (p=0), <b>Trad</b> (p=0), <b>Conf-r</b> (p=0)                           |

Table S141: Self-Transcendence: system registry (test split). Each system is assigned an ID to avoid repeating long configuration strings in the comparison table. Best Macro- $F_1$  for Self-Transcendence is shown in bold. Values are reported with 5 decimals to avoid artificial ties.

| ID  | System (configuration)                                                                          | Macro- $F_1$   |
|-----|-------------------------------------------------------------------------------------------------|----------------|
| T1  | Transformer / Direct: Baseline (thr=0.50)                                                       | 0.25396        |
| T2  | Transformer / Direct: 2 prev sent w/ label (thr=0.50)                                           | 0.26317        |
| T3  | Transformer / Direct: Baseline (thr=0.30)                                                       | 0.30233        |
| T4  | Transformer / Direct: 2 prev sent w/ label (thr=0.15)                                           | 0.30747        |
| P1  | Transformer / Presence: Baseline (thr=0.50), filter=Previous-Sentences-2-Lex-EmoLex (thr=0.10)  | 0.28012        |
| P2  | Transformer / Presence: Lex - VAD (thr=0.50), filter=Previous-Sentences-2-Lex-EmoLex (thr=0.10) | 0.29678        |
| P3  | Transformer / Presence: Baseline (thr=0.25), filter=Previous-Sentences-2-Lex-EmoLex (thr=0.10)  | 0.30181        |
| P4  | Transformer / Presence: Lex - MJD (thr=0.30), filter=Previous-Sentences-2-Lex-EmoLex (thr=0.10) | 0.31059        |
| ST1 | Transformer / Self-Transcendence: Baseline (thr=0.50), filter=Lex - WorryWords (thr=0.16)       | 0.30067        |
| ST2 | Transformer / Self-Transcendence: Lex - Schwartz (thr=0.50), filter=Lex - WorryWords (thr=0.16) | 0.30137        |
| ST3 | Transformer / Self-Transcendence: Baseline (thr=0.50), filter=Lex - MFD-20 (thr=0.50)           | 0.29836        |
| ST4 | Transformer / Self-Transcendence: Baseline (thr=0.25), filter=Lex - MFD-20 (thr=0.50)           | 0.30734        |
| ETr | Transformer / Ensemble (Transformers): champions ensemble (soft voting; thr=0.29; test)         | <b>0.31937</b> |
| L1  | LLM / Self-Transcendence: Gemma 2 9B Zero-Shot                                                  | 0.15871        |
| L2  | LLM / Self-Transcendence: Gemma 2 9B Zero-Shot + SBERT gate (filter-thr=0.47)                   | 0.18697        |
| L3  | LLM / Self-Transcendence: Gemma 2 9B Few-Shot                                                   | 0.21326        |
| L4  | LLM / Self-Transcendence: Gemma 2 9B Few-Shot + SBERT gate (filter-thr=0.38)                    | 0.22149        |
| L5  | LLM / Self-Transcendence: Gemma 2 9B QLoRA + SBERT gate (filter-thr=0.29)                       | 0.12381        |
| ELL | LLM / Self-Transcendence: ensemble (hard voting; fixed thr=0.50; test)                          | 0.22009        |



Table S142: Self-Transcendence: paired statistical comparisons on the **test** split. Each row compares Model1 vs. Model2 (by ID from Table S141), reporting their test Macro- $F_1$ , the one-sided lower 95% bootstrap confidence bound for  $\Delta$  Macro- $F_1$  (Model2 – Model1), and the one-sided  $p$ -value for  $\Delta > 0$ . Values are reported with 5 decimals to avoid artificial ties.

| Comparison                                           | Model1 ID | Macro- $F_1$ (M1) | Model2 ID | Macro- $F_1$ (M2) | $\Delta$ Macro- $F_1$ LB <sub>0.95</sub> | $p$ / Sig.    |
|------------------------------------------------------|-----------|-------------------|-----------|-------------------|------------------------------------------|---------------|
| Model (Direct)                                       | T1        | 0.25396           | T2        | 0.26317           | -0.00480                                 | 0.14440 / No  |
| Tuning threshold (Direct)                            | T1        | 0.25396           | T3        | 0.30233           | 0.03130                                  | 0 / Yes       |
| Tuning threshold + Model (Direct)                    | T3        | 0.30233           | T4        | 0.30747           | -0.02090                                 | 0.35500 / No  |
| Model (Presence)                                     | P1        | 0.28012           | P2        | 0.29678           | 0.00490                                  | 0.01100 / Yes |
| Tuning threshold (Presence)                          | P1        | 0.28012           | P3        | 0.30181           | 0.00480                                  | 0.00800 / Yes |
| Tuning threshold + Model (Presence)                  | P3        | 0.30181           | P4        | 0.31059           | -0.00030                                 | 0.05600 / No  |
| Model (Self-Transcendence)                           | ST1       | 0.30067           | ST2       | 0.30137           | -0.01260                                 | 0.41800 / No  |
| Tuning threshold (Self-Transcendence)                | ST3       | 0.29836           | ST4       | 0.30734           | 0.00220                                  | 0.01450 / Yes |
| Architecture champion (Presence vs Direct)           | P3        | 0.30181           | T3        | 0.30233           | -0.01090                                 | 0.46550 / No  |
| Architecture champion (Self-Transcendence vs Direct) | T3        | 0.30233           | ST4       | 0.30734           | -0.01620                                 | 0.36850 / No  |
| Single vs Ensemble Transformer champions             | T3        | 0.30233           | ETr       | <b>0.31937</b>    | -0.00710                                 | 0.12500 / No  |
| Adding SBERT gate (LLM)                              | L1        | 0.15871           | L2        | 0.18697           | 0.02150                                  | 0 / Yes       |
| Zero-shot vs Few-shot (LLM)                          | L1        | 0.15871           | L3        | 0.21326           | 0.03740                                  | 0 / Yes       |
| Adding SBERT gate (LLM, few-shot)                    | L3        | 0.21326           | L4        | 0.22149           | -0.00620                                 | 0.13700 / No  |
| Finetuning with QLoRA vs best zero/few-shot (LLM)    | L3        | 0.21326           | L5        | 0.12381           | -0.11690                                 | 1.00000 / No  |
| Single vs Ensemble LLM                               | L3        | 0.21326           | ELL       | 0.22009           | -0.01180                                 | 0.26200 / No  |
| Transformer vs LLM champions                         | L3        | 0.21326           | T3        | 0.30233           | 0.06160                                  | 0 / Yes       |

Table S143: Self-Transcendence: per-label McNemar exact tests on positives. We list only labels with McNemar  $p \leq 0.05$  after Benjamini–Hochberg FDR control ( $\alpha = 0.05$ ) for the corresponding comparison (Model2 vs. Model1). Abbreviations are used for label names. Model IDs refer to Table S141.

| Comparison                            |             |  |  | Model1 ID | Model2 ID | Significant labels (McNemar $p$ )                                                                       |
|---------------------------------------|-------------|--|--|-----------|-----------|---------------------------------------------------------------------------------------------------------|
| Tuning threshold (Direct)             | (Di-        |  |  | T1        | T3        | <b>Ben-c</b> (p=0), <b>Ben-d</b> (p=0), <b>Uni-c</b> (p=0), <b>Uni-n</b> (p=0), <b>Uni-t</b> (p=0.0001) |
| Model (Presence)                      |             |  |  | P1        | P2        | <b>Ben-d</b> (p=0.0332), <b>Uni-c</b> (p=0.0018)                                                        |
| Tuning threshold (Presence)           | (Pres-      |  |  | P1        | P3        | <b>Ben-c</b> (p=0), <b>Ben-d</b> (p=0), <b>Uni-c</b> (p=0), <b>Uni-n</b> (p=0), <b>Uni-t</b> (p=0)      |
| Tuning threshold (Self-Transcendence) | (Self-      |  |  | ST3       | ST4       | <b>Ben-d</b> (p=0.0104), <b>Uni-c</b> (p=0.0005), <b>Uni-t</b> (p=0.0005)                               |
| Adding SBERT (LLM)                    | gate        |  |  | L1        | L2        | <b>Ben-c</b> (p=0), <b>Ben-d</b> (p=0), <b>Uni-c</b> (p=0), <b>Uni-n</b> (p=0), <b>Uni-t</b> (p=0.0003) |
| Zero-shot (LLM)                       | vs Few-shot |  |  | L1        | L3        | <b>Ben-c</b> (p=0.0002), <b>Ben-d</b> (p=0), <b>Uni-n</b> (p=0.0251)                                    |
| Transformer champions                 | vs LLM      |  |  | L3        | T3        | <b>Ben-c</b> (p=0), <b>Ben-d</b> (p=0.0019), <b>Uni-c</b> (p=0), <b>Uni-n</b> (p=0)                     |

Table S144: Self-Enhancement: system registry (test split). Each system is assigned an ID to avoid repeating long configuration strings in the comparison table. Best Macro- $F_1$  for Self-Enhancement is shown in bold. Values are reported with 5 decimals to avoid artificial ties.

| ID  | System (configuration)                                                                           | Macro- $F_1$   |
|-----|--------------------------------------------------------------------------------------------------|----------------|
| T1  | Transformer / Direct: Baseline (thr=0.50)                                                        | 0.29242        |
| T2  | Transformer / Direct: Lex - LIWC 22 (thr=0.50)                                                   | 0.30440        |
| T3  | Transformer / Direct: Baseline (thr=0.30)                                                        | 0.32178        |
| T4  | Transformer / Direct: 2 prev sent w/ label (thr=0.15)                                            | <b>0.33843</b> |
| P1  | Transformer / Presence: Baseline (thr=0.50), filter=Previous-Sentences-2-Lex-LIWC-22 (thr=0.10)  | 0.32005        |
| P2  | Transformer / Presence: Lex - MJD (thr=0.50), filter=Previous-Sentences-2-Lex-LIWC-22 (thr=0.10) | 0.33118        |
| P3  | Transformer / Presence: Baseline (thr=0.30), filter=Previous-Sentences-2-Lex-LIWC-22 (thr=0.10)  | 0.32572        |
| SE1 | Transformer / Self-Enhancement: Baseline (thr=0.50), filter=Lex - WorryWords (thr=0.23)          | 0.31398        |
| SE2 | Transformer / Self-Enhancement: Lex - Schwartz (thr=0.50), filter=Lex - WorryWords (thr=0.23)    | 0.31881        |
| SE3 | Transformer / Self-Enhancement: Baseline (thr=0.60), filter=Lex - WorryWords (thr=0.23)          | 0.30954        |
| SE4 | Transformer / Self-Enhancement: Lex - Schwartz (thr=0.55), filter=Lex - WorryWords (thr=0.23)    | 0.31916        |
| ETr | Transformer / Ensemble (Transformers): champions ensemble (soft voting; thr=0.29; test)          | 0.33728        |
| L1  | LLM / Self-Enhancement: Gemma 2 9B Zero-Shot                                                     | 0.17485        |
| L2  | LLM / Self-Enhancement: Gemma 2 9B Zero-Shot + SBERT gate (filter-thr=0.39)                      | 0.18154        |
| L3  | LLM / Self-Enhancement: Gemma 2 9B Few-Shot                                                      | 0.22129        |
| L4  | LLM / Self-Enhancement: Gemma 2 9B Few-Shot + SBERT gate (filter-thr=0.34)                       | 0.22174        |
| L5  | LLM / Self-Enhancement: Gemma 2 9B QLoRA + SBERT gate (filter-thr=0.11)                          | 0.22667        |
| EHy | Hybrid / Ensemble (Transformer+LLM): ensemble of both (test)                                     | 0.34866        |

Table S145: Self-Enhancement: paired statistical comparisons on the **test** split. Each row compares Model1 vs. Model2 (by ID from Table S144), reporting their test Macro- $F_1$ , the one-sided lower 95% bootstrap confidence bound for  $\Delta$  Macro- $F_1$  (Model2–Model1), and the one-sided  $p$ -value for  $\Delta > 0$ . Values are reported with 5 decimals to avoid artificial ties.

| Comparison                                         | Model1 ID | Macro- $F_1$ (M1) | Model2 ID | Macro- $F_1$ (M2) | $\Delta$ Macro- $F_1$ LB <sub>0.95</sub> | $p$ / Sig.    |
|----------------------------------------------------|-----------|-------------------|-----------|-------------------|------------------------------------------|---------------|
| Model (Direct)                                     | T1        | 0.29242           | T2        | 0.30440           | -0.00230                                 | 0.08300 / No  |
| Tuning threshold (Direct)                          | T1        | 0.29242           | T3        | 0.32178           | 0.01930                                  | 0.00000 / Yes |
| Tuning threshold + Model (Direct)                  | T3        | 0.32178           | T4        | <b>0.33843</b>    | 0.00180                                  | 0.03100 / Yes |
| Model (Presence)                                   | P1        | 0.32005           | P2        | 0.33118           | -0.00070                                 | 0.06200 / No  |
| Tuning threshold (Presence)                        | P1        | 0.32005           | P3        | 0.32572           | -0.00210                                 | 0.11250 / No  |
| Model (Self-Enhancement)                           | SE1       | 0.31398           | SE2       | 0.31881           | -0.00330                                 | 0.17050 / No  |
| Post-hoc Tuning threshold (Self-Enhancement)       | SE1       | 0.31398           | SE3       | 0.30954           | -0.00990                                 | 0.03450 / No  |
| Post-hoc Tuning threshold + Model (over tuned)     | SE3       | 0.30954           | SE4       | 0.31916           | 0.00110                                  | 0.02950 / Yes |
| Post-hoc Tuning threshold + Model (over fixed)     | SE1       | 0.31398           | SE4       | 0.31916           | -0.00320                                 | 0.15250 / No  |
| Architecture champion (Presence vs Direct)         | P1        | 0.32005           | T4        | <b>0.33843</b>    | 0.00370                                  | 0.01700 / Yes |
| Architecture champion (Self-Enhancement vs Direct) | SE1       | 0.31398           | T4        | <b>0.33843</b>    | 0.00970                                  | 0.00450 / Yes |
| Single vs Ensemble Transformer champions           | T4        | 0.33843           | ETr       | 0.33728           | -0.01360                                 | 0.54700 / No  |
| Adding SBERT gate (LLM)                            | L1        | 0.17485           | L2        | 0.18154           | -0.00080                                 | 0.07050 / No  |
| Zero-shot vs Few-shot (LLM)                        | L1        | 0.17485           | L3        | 0.22129           | 0.03830                                  | 0.00000 / Yes |
| Adding SBERT gate (LLM, few-shot)                  | L3        | 0.22129           | L4        | 0.22174           | -0.00830                                 | 0.48600 / No  |
| Finetuning with QLoRA vs best zero/few-shot (LLM)  | L3        | 0.22129           | L5        | 0.22667           | -0.01470                                 | 0.34100 / No  |
| Transformer vs LLM champions                       | L3        | 0.22129           | T4        | <b>0.33843</b>    | 0.10260                                  | 0.00000 / Yes |
| Transformer vs LLM winner vs Hybrid ensemble       | T4        | 0.33843           | EHy       | 0.34866           | -0.00250                                 | 0.09200 / No  |

Table S146: Self-Enhancement: per-label McNemar exact tests on positives. We list only labels with McNemar  $p \leq 0.05$  after Benjamini–Hochberg FDR control ( $\alpha = 0.05$ ) for the corresponding comparison (Model2 vs. Model1). Abbreviations are used for label names. Model IDs refer to Table S144.

| Comparison                                     | Model1 ID | Model2 ID | Significant labels (McNemar $p$ )                                                                       |
|------------------------------------------------|-----------|-----------|---------------------------------------------------------------------------------------------------------|
| Tuning threshold (Direct)                      | T1        | T3        | <b>Hed</b> (p=0), <b>Ach</b> (p=0), <b>Pow-d</b> (p=0), <b>Pow-r</b> (p=0)                              |
| Tuning threshold + Model (Direct)              | T3        | T4        | <b>Ach</b> (p=0.0006)                                                                                   |
| Post-hoc Tuning threshold + Model (over tuned) | SE3       | SE4       | <b>Hed</b> (p=0.0041), <b>Ach</b> (p=0.0272), <b>Pow-d</b> (p=0.0272)                                   |
| Zero-shot vs Few-shot (LLM)                    | L1        | L3        | <b>Hed</b> (p=0.0029), <b>Ach</b> (p=0), <b>Pow-d</b> (p=0), <b>Pow-r</b> (p=0)                         |
| Transformer vs LLM champions                   | L3        | T4        | <b>Hed</b> (p=0.0002), <b>Ach</b> (p=0), <b>Pow-d</b> (p=0), <b>Pow-r</b> (p=0), <b>Face</b> (p=0.0414) |
